# Supplementary material for: Statistically Significant Detection of Linguistic Change
Source: arXiv:1411.3315 source file (2014-11-12)
Supplement: Supplementary file 1 [file appendices.tex]

\newpage
\appendix
\section{Language change trends}
We seek to obtain some insight into the trends of language change on the media of linguistic expression we analyzed. For each data set, we looked at all the words that our method detected to have changed (at a \pvalue\ < 0.01$ and $Z-Score > 1.75$). Figure \ref{fig:cp_hist} shows the distribution of change points. Based on this , we observe the following:
\begin{itemize}
\item Word meaning changes occur in bursts and not uniformly. This is consistent with the observations made by \cite{Atkinson01022008} who observed that language change is not uniform across time and "tends to evolve in rapid or punctuational bursts".
\item Observe that in Google Book Ngrams, we notice several changes in periods $1960-1980$. On the online forum of Amazon movie reviews, we observe the change is concentrated around $2006-2008$ which we hypothesize corresponds to a surge in online viewing and downloading (as we observe words like $streaming$, $download$, $delivered$ to have changed during this period). On Twitter we observe quite a large number of words changed during Aug 2012. We observe most of these words are abbreviations like $RT$ (retweet) etc. We are still investigating an explanation for this behavior.

\end{itemize}

\begin{figure}[htb]
\begin{subfigure}{0.25\textwidth}
  \centering
  \includegraphics[width = 1.0\textwidth]{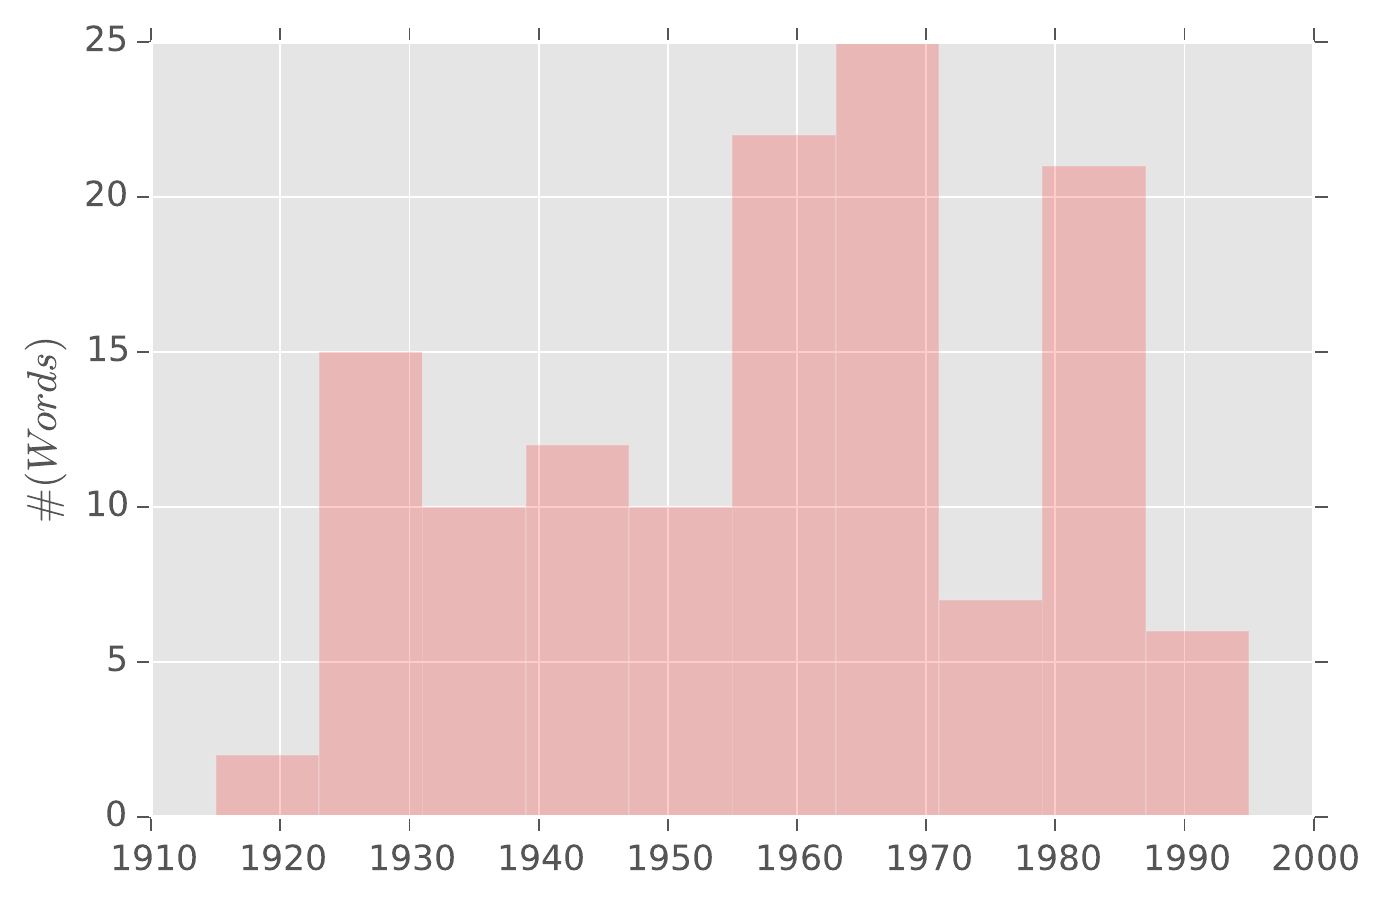}
  \caption{Google Book Ngrams}
  \label{fig:ngrams_hist}
\end{subfigure}%
\begin{subfigure}{0.25\textwidth}
  \centering
  \includegraphics[width = 1.0\textwidth]{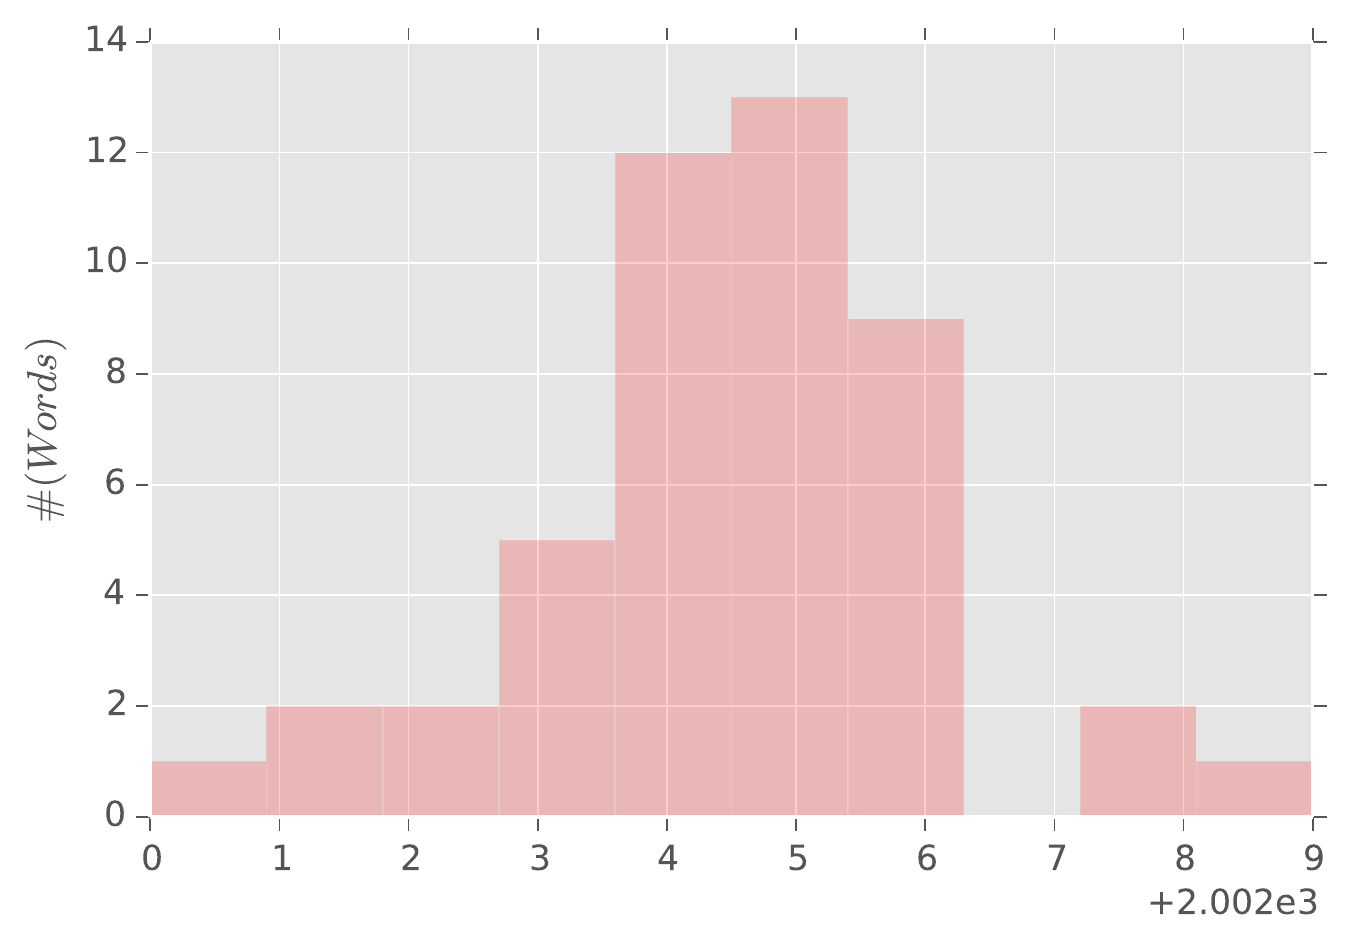}
  \caption{Amazon Movie Reviews}
  \label{fig:movies_hist}
\end{subfigure}%
\\
\begin{subfigure}{0.25\textwidth}
  \centering
  \includegraphics[width = 1.0\textwidth]{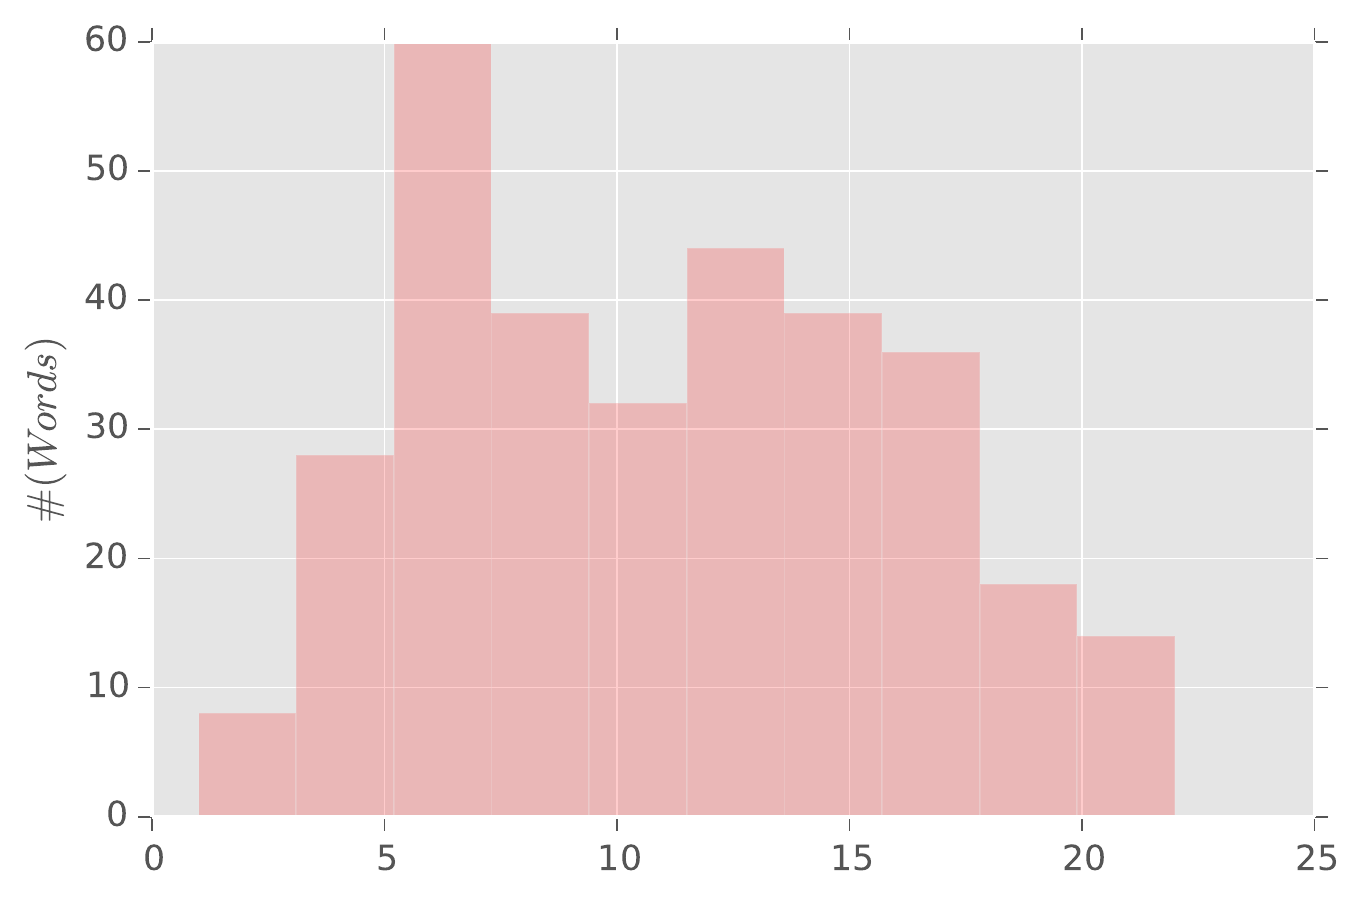}
  \caption{Twitter}
  \label{fig:twitter_hist}
\end{subfigure}%
\caption{Distribution of changepoints for our method detects as changed ( pvalue < 0.01 and Z-Score >= 1.75)}
\label{fig:cp_hist}
\end{figure}

We also tried to study how language drifts through time (at a global level) as well. In order to achieve this, we draw on concepts from Language Modeling. A language model learns a probability distribution over a sequence of words (usually unigrams, bigrams and trigrams). To evaluate the quality of a language model , inorder to understand how well the model captures the underlying probability distribution of the language, we use the well known metric of Perplexity to evaluate the model on evaluation data set. Perplexity is related to the cross entropy between the distribution learnt by the model and that of the evaluation data. We can use this metric to get some insight into language change at a global level as follows:
\begin{itemize}
\item Estimate a language model (LM) on corpus snapshot $C_0$ which we take as the baseline.
\item For each subsequent snapshot $C_i$, we calculate the perplexity $P_i$ of the learnt model. When language at a snapshot is similar to the perplexity wiil be low. However as language changes and drifts apart the perplexity will increase.
\end{itemize}

We use the MIT Language Modeling Toolkit \cite{MITLM} to estimate a trigram Language model. We restrict the language model to only the vocabulary common across all time snapshots of the corpora. Figure \ref{fig:perpl} shows how the perplexity changes for subsequent $C_i$ for all the three data sets we consider.

\begin{figure*}
\begin{subfigure}{0.3\textwidth}
  \centering
  \includegraphics[width = 1.0\textwidth]{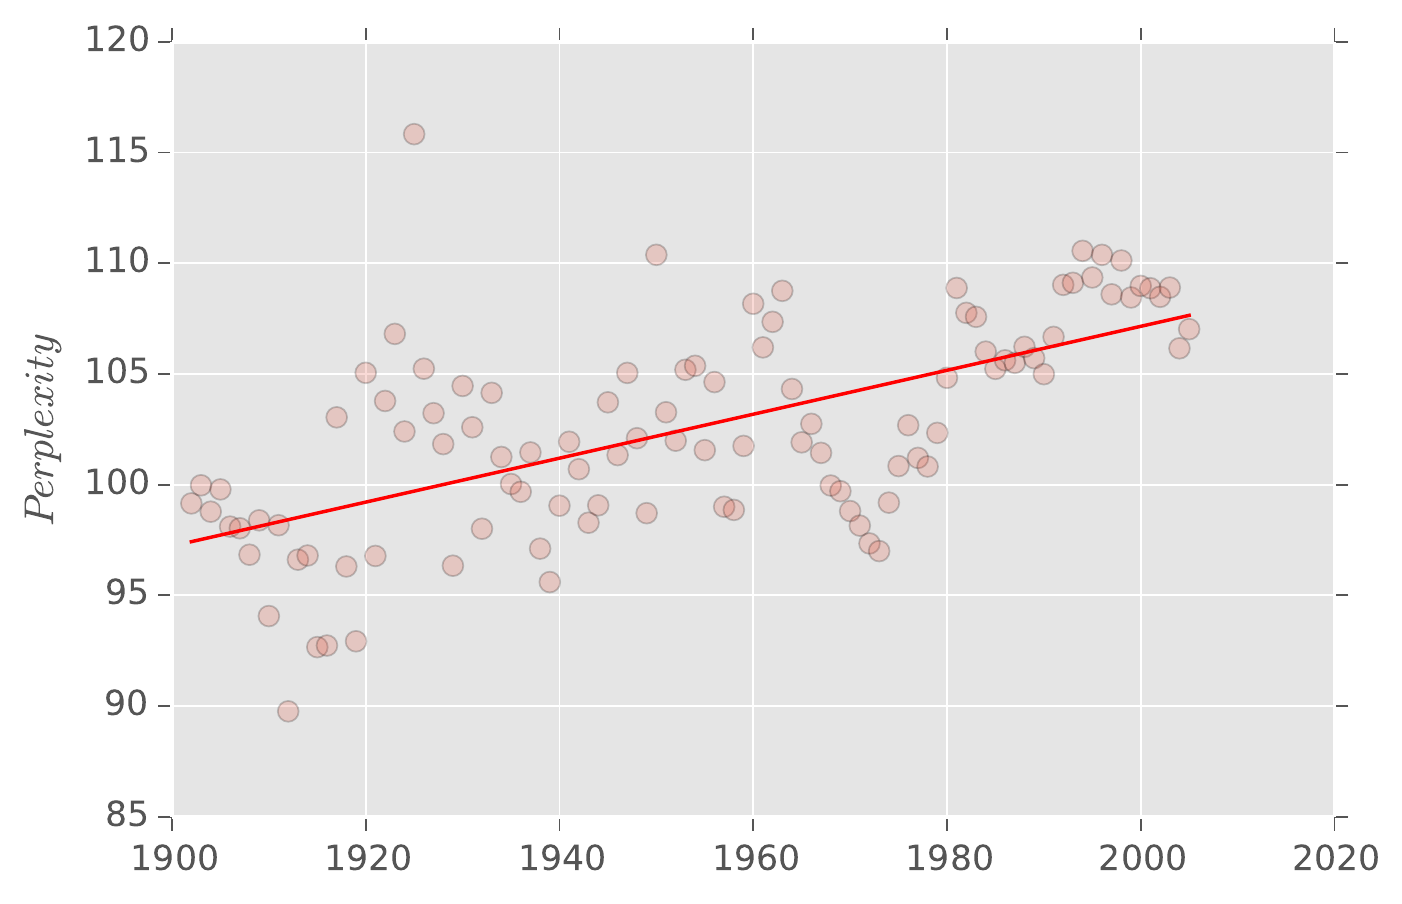}
  \caption{Google Book Ngrams \\ \emph{Slope}:0.09}
  \label{fig:ngrams_perpl}
\end{subfigure}%
\begin{subfigure}{0.3\textwidth}
  \centering
  \includegraphics[width = 1.0\textwidth]{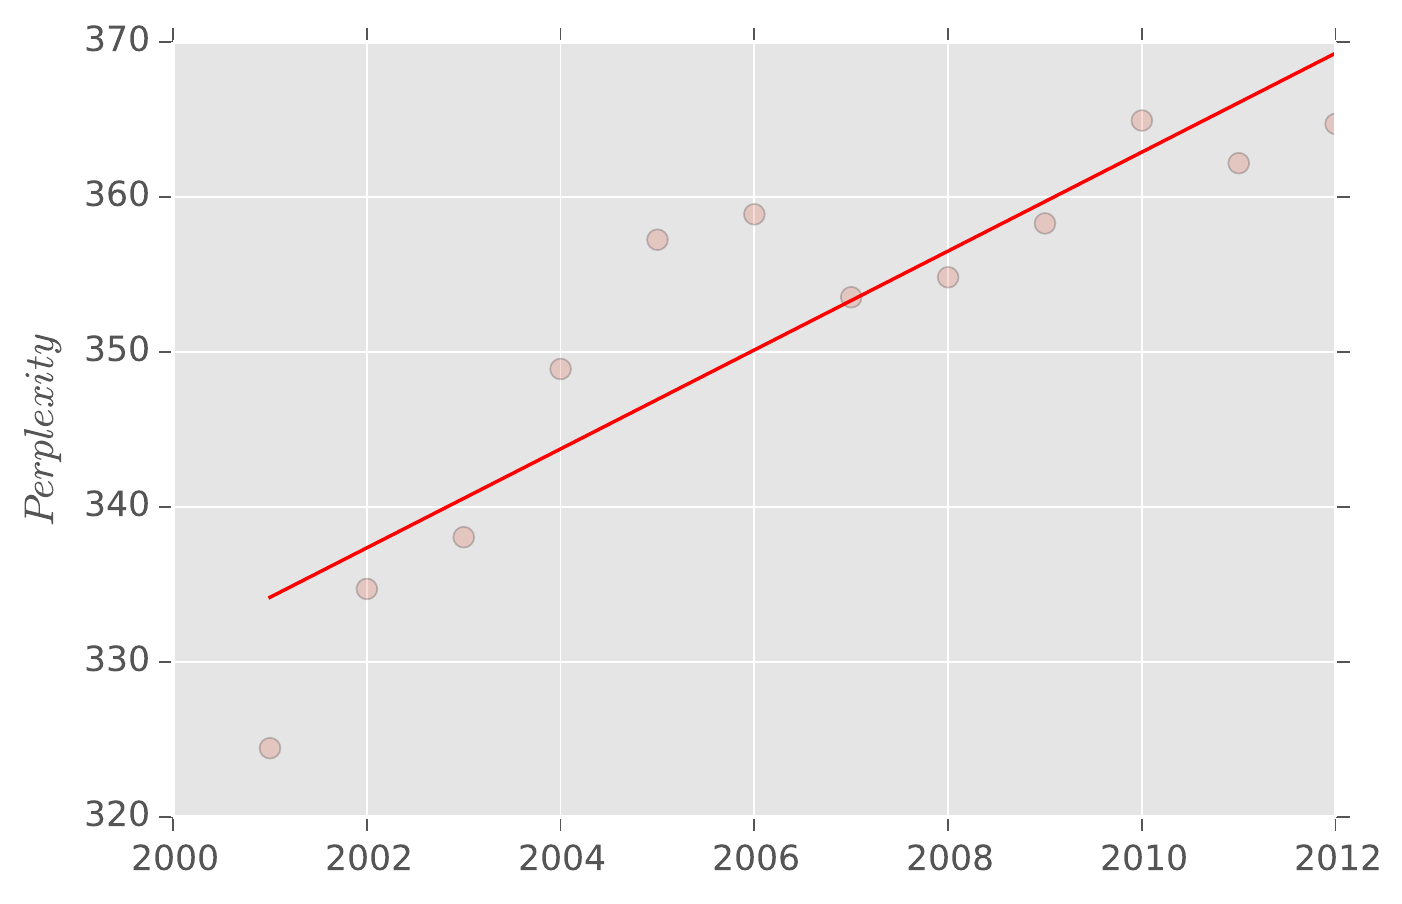}
  \caption{Amazon Movie Reviews \\ \emph{Slope}:3.19}
  \label{fig:movies_perpl}
\end{subfigure}%
\begin{subfigure}{0.3\textwidth}
  \centering
  \includegraphics[width = 1.0\textwidth]{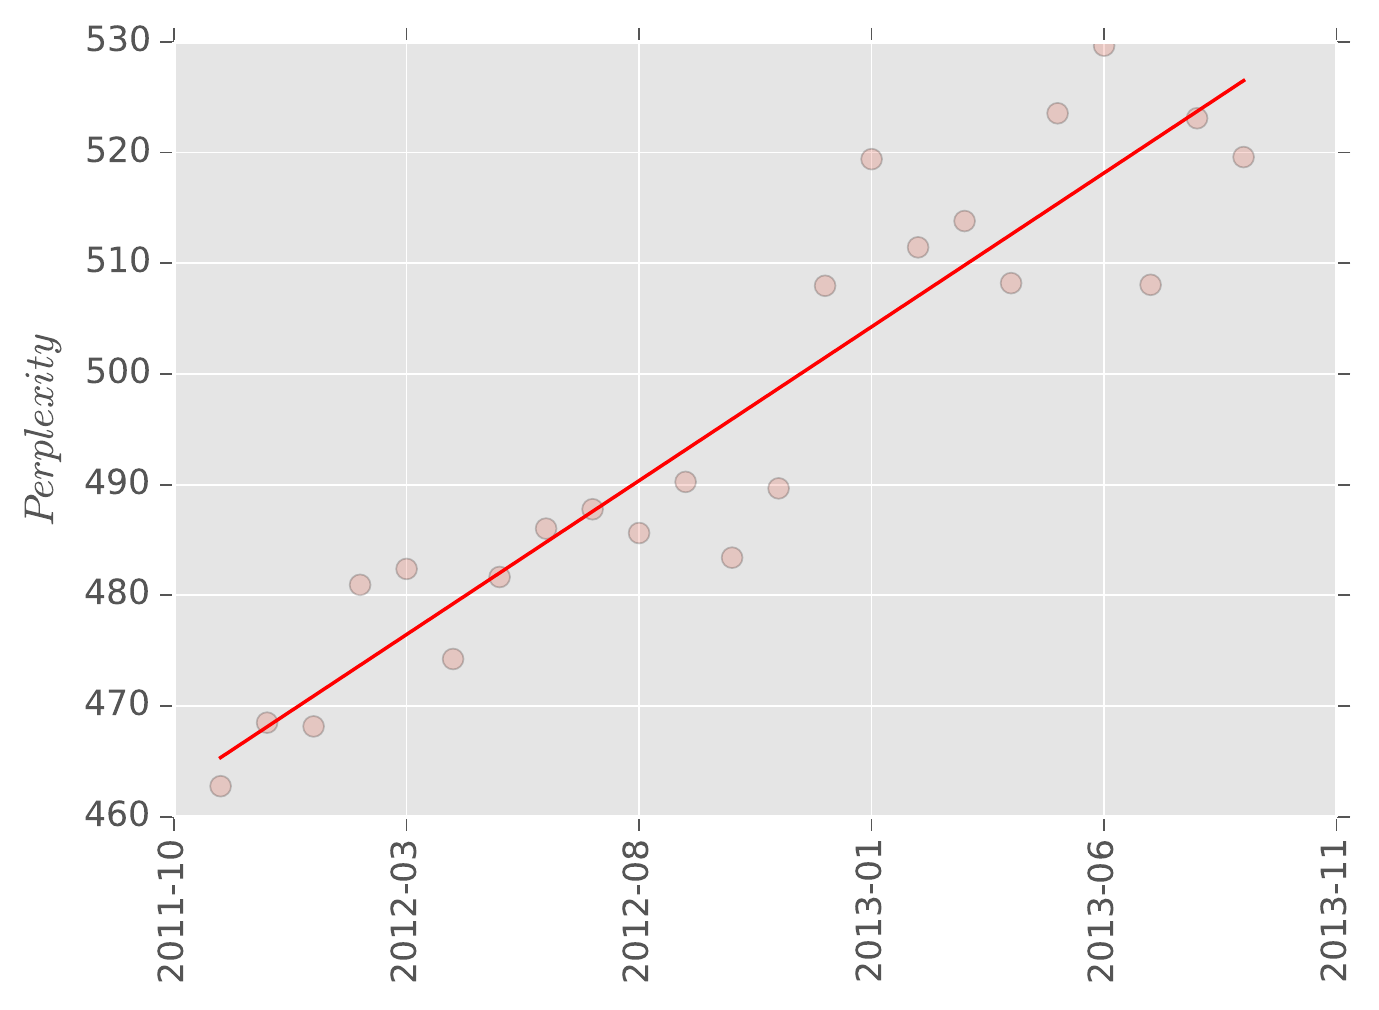}
  \caption{Twitter Slope \\ \emph{Slope}:2.77}
  \label{fig:twitter_perpl}
\end{subfigure}%
\caption{Evolution of perplexity of language over time compared to baseline. \todo{Fix the timepoints for Twitter}}
\label{fig:perpl}
\end{figure*}

We fit a least squares line to the above to obtain an estimate of the rate of drift . Observe that the rate of change is highest in Twitter, followed by Amazon Movie Reviews, followed by Google Book Ngrams.

\section{Snippets}

The choice of words or phrases is essential for the insights that could be drawn from the data.
Word ambiguity and semantic changes complicate the analysis of purely frequency based approach and limits the utility of such approaches.

To address these concerns, a new version of Google Book ngrams \cite{goldberg:syntacticngrams} was released to enable more fine-grain search.
The corpora is annotated with Part-Of-Speech tags to identify the different senses a word may have.
This enable the user to pick which part of speech to use when they are searching.

\section{Figures}
\begin{figure}[t!]
\begin{subfigure}{0.25\textwidth}
  \centering
  \includegraphics[width=\textwidth]{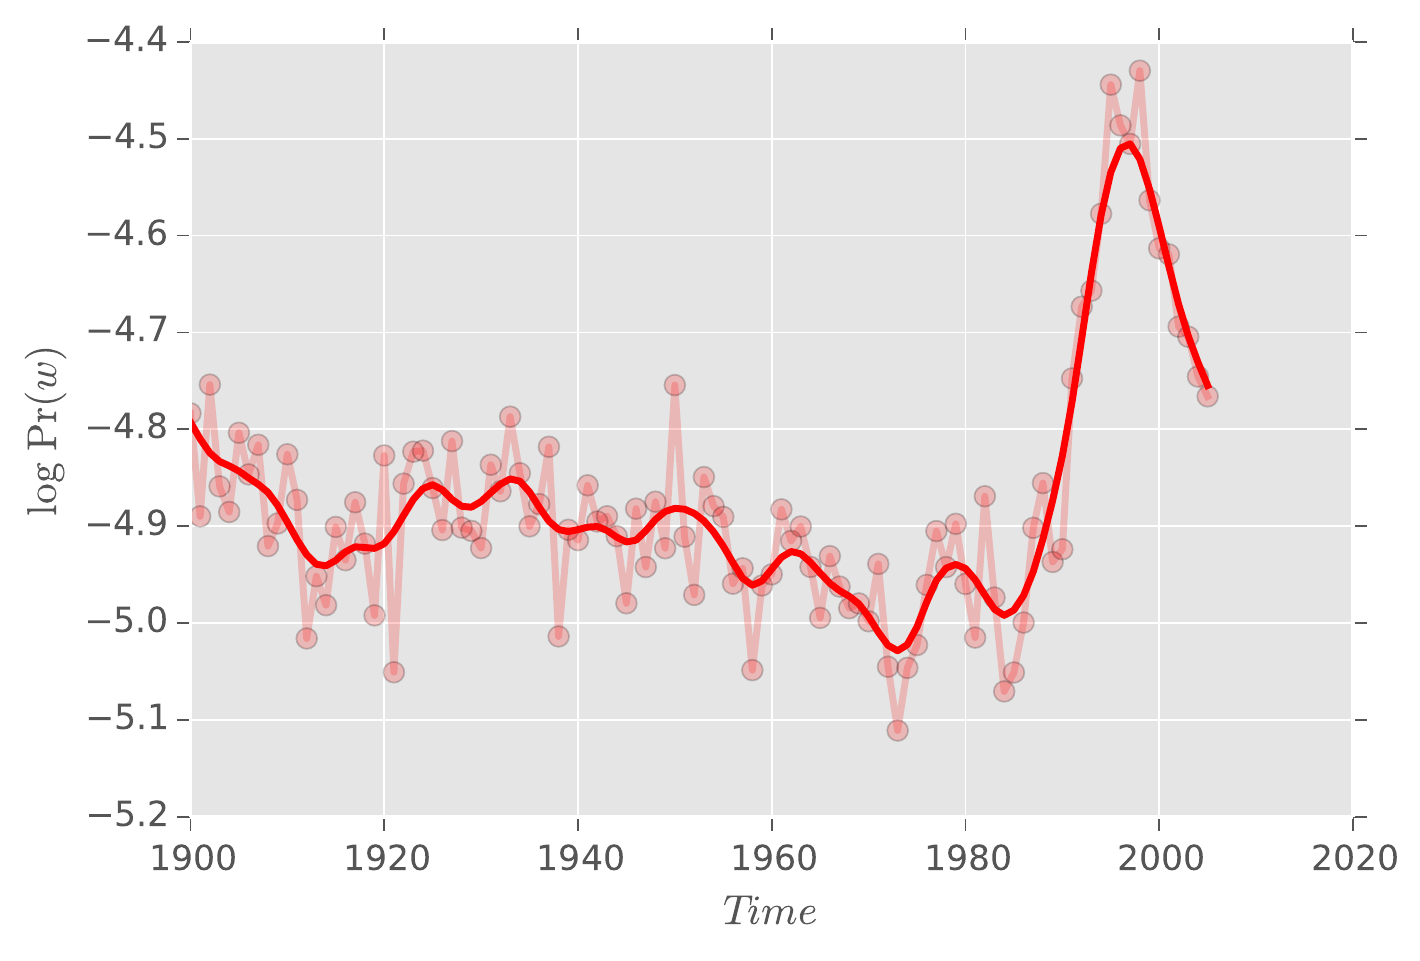}
  \caption{\texttt{gay}.}
  \label{fig:sfig1}
\end{subfigure}%
\begin{subfigure}{0.25\textwidth}
  \centering
  \includegraphics[width=\textwidth]{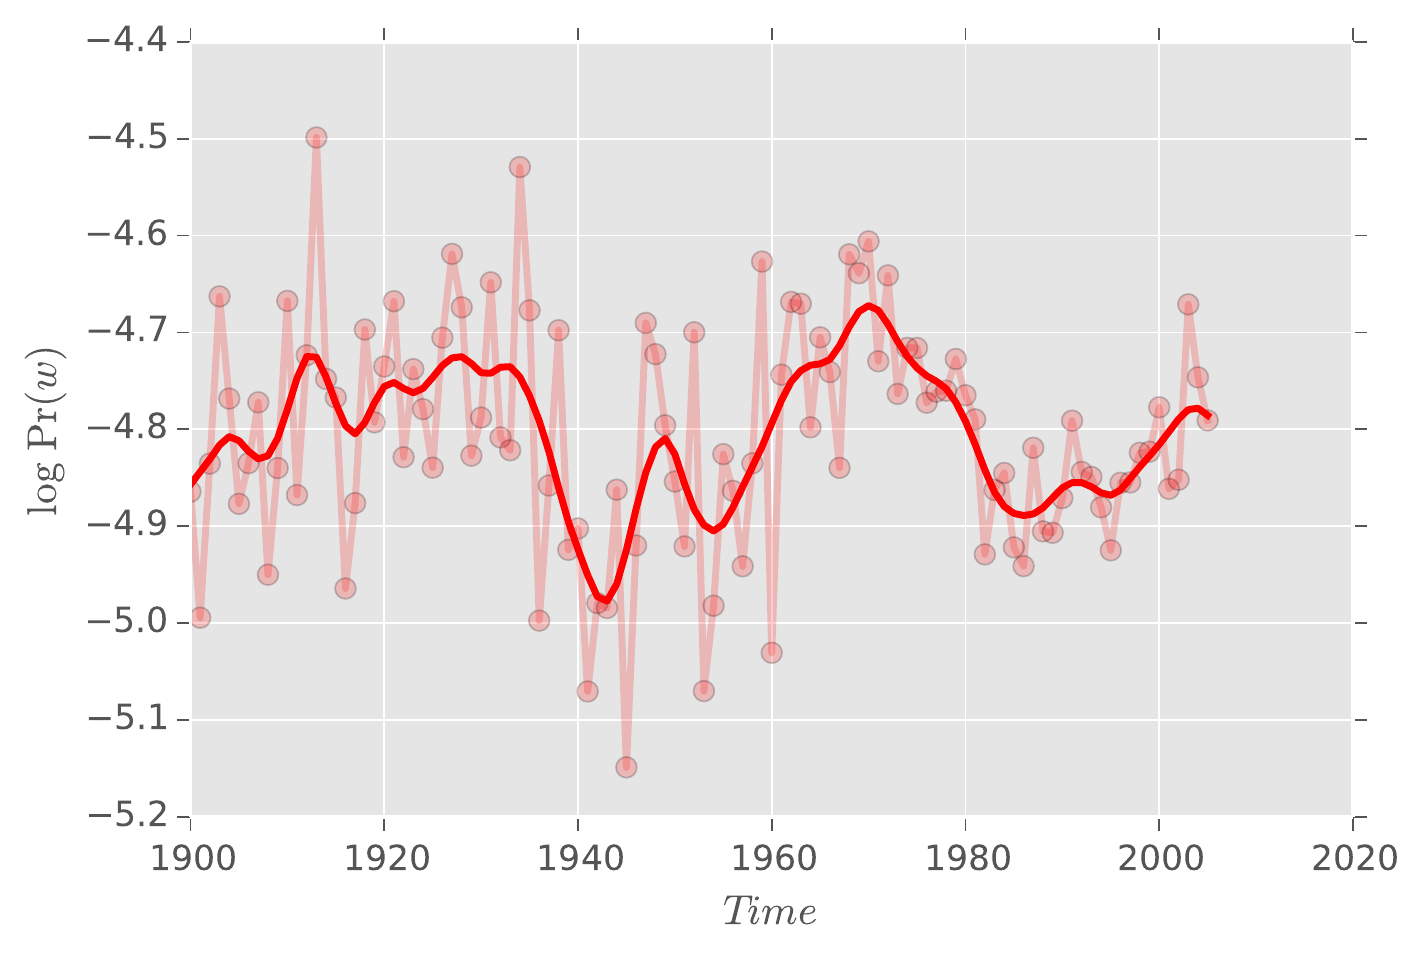}
  \caption{\texttt{God}}
  \label{fig:sfig2}
\end{subfigure}%
	\caption{Frequency usage of \emph{gay, God} over time, the first has undergone a shift while the other stable.
Observe the sudden change in frequency of \emph{gay} around $1970$.}
%\label{fig:freq}
\end{figure}

\begin{figure}
\begin{subfigure}{0.25\textwidth}
  \centering
  \includegraphics[width=\textwidth]{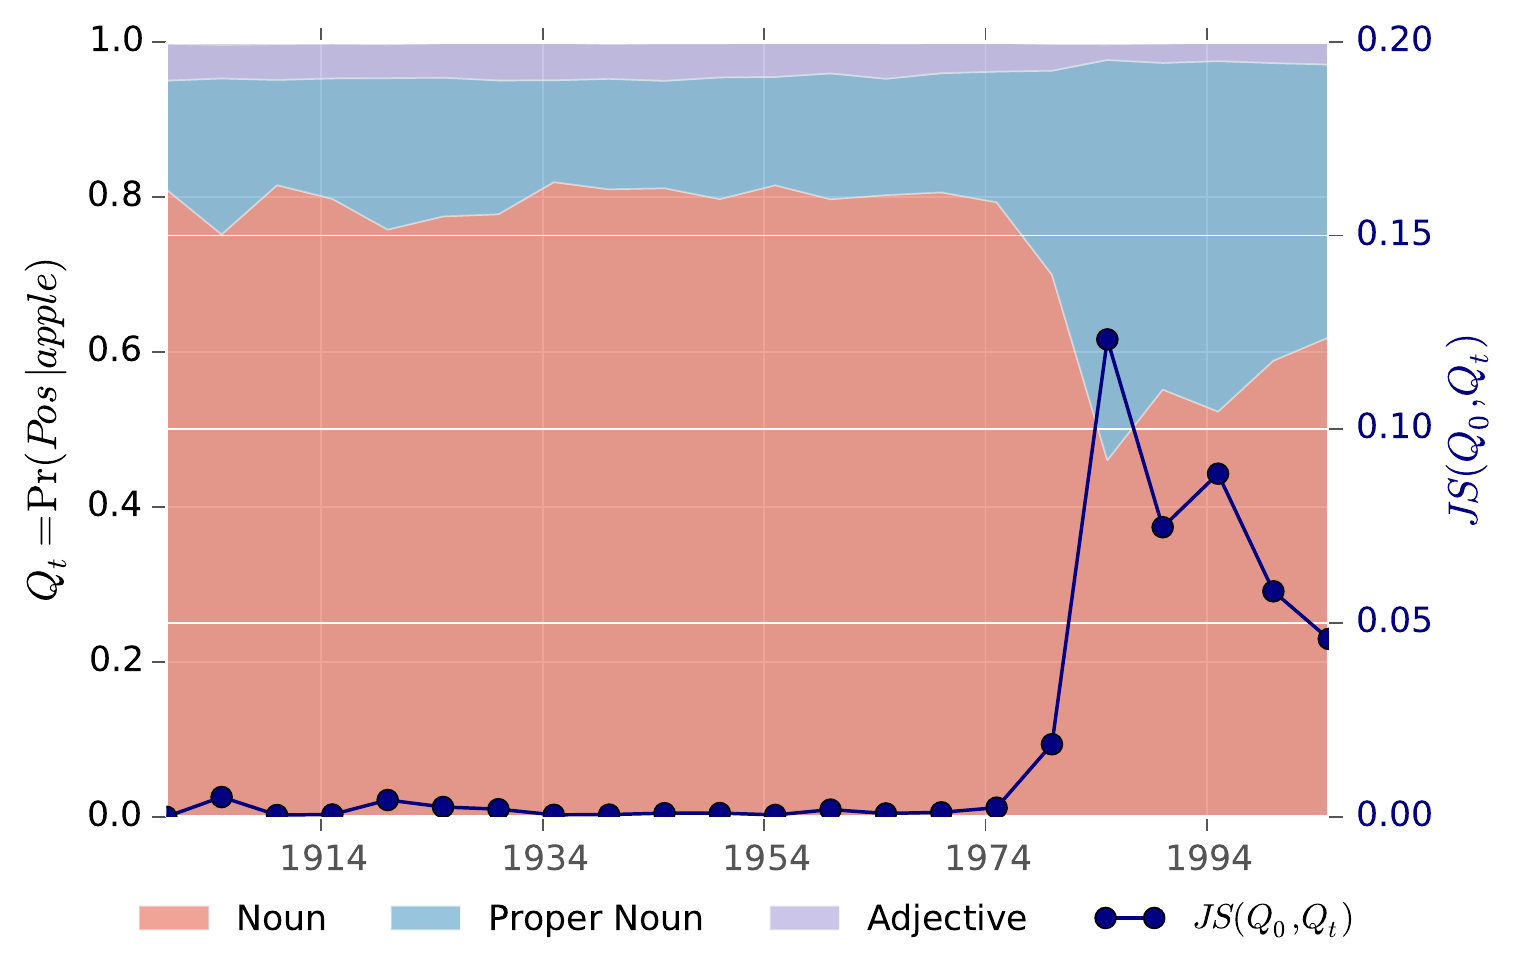}
  \caption{\emph{apple} }
  \label{fig:pfig1}
\end{subfigure}%
\begin{subfigure}{0.25\textwidth}
  \centering
  \includegraphics[width=\textwidth]{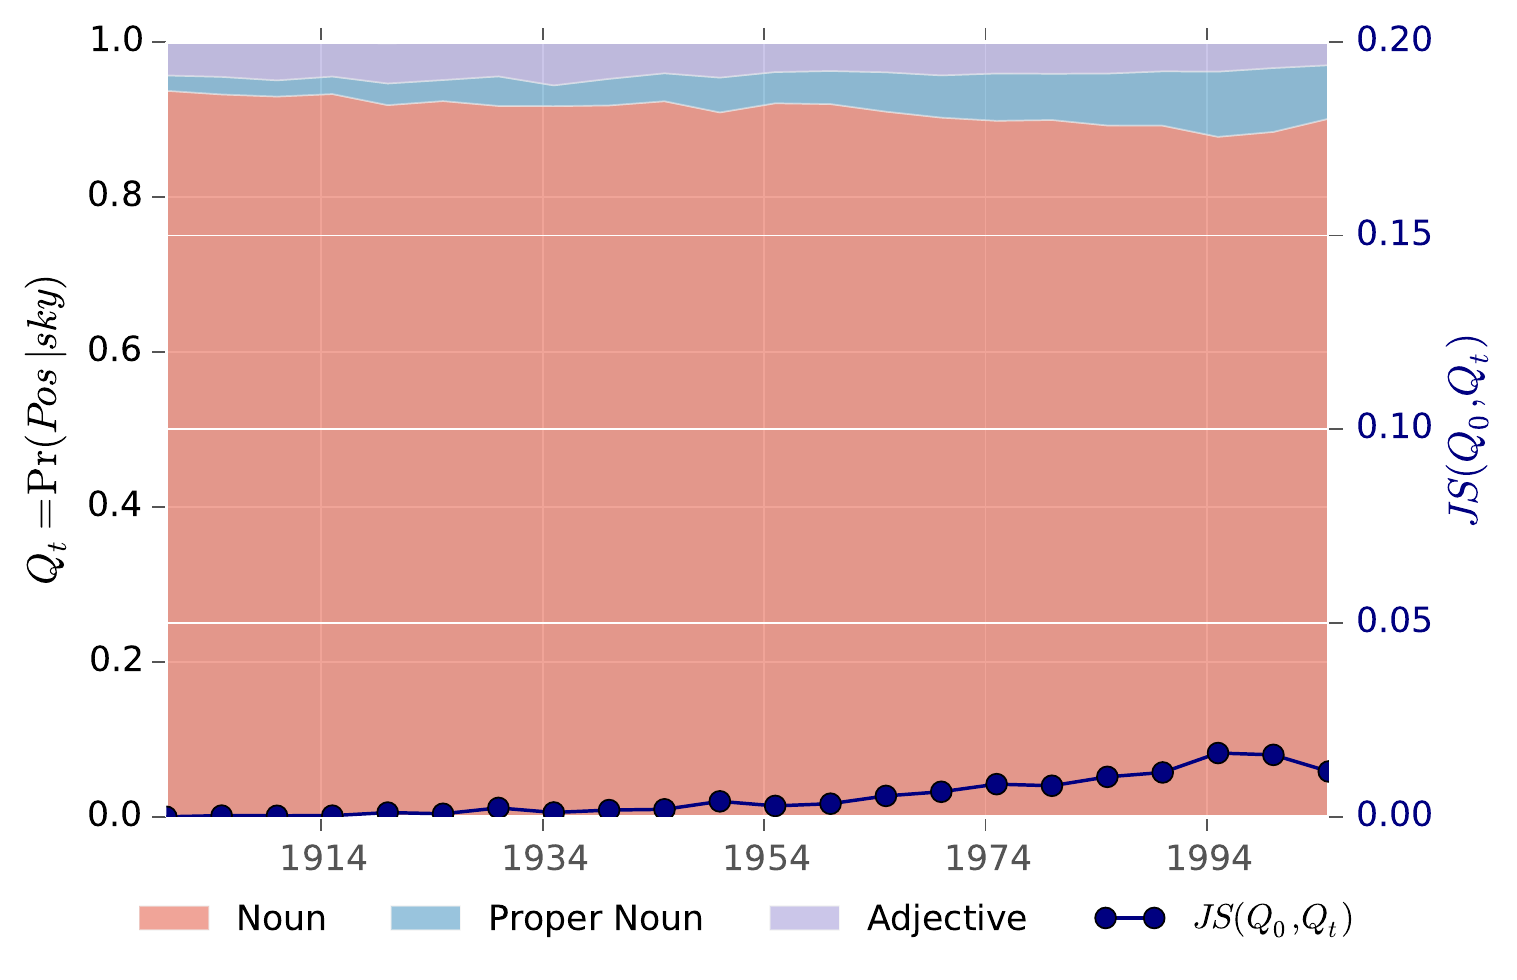}
  \caption{\emph{sky} }
  \label{fig:pfig2}
\end{subfigure}%
\caption{\small Stacked area chart represents the POS Distributions while the dotted line represents the time series constructed from the JS divergence.
On the left, the usage of \emph{apple} as ``Proper Noun" has dramatically increased in 1980s while \emph{sky} (on the right) stayed relatively stable.}
%\label{fig:pos}
\end{figure}

\begin{figure}
\begin{subfigure}{0.25\textwidth}
  \centering
  \includegraphics[width=\textwidth]{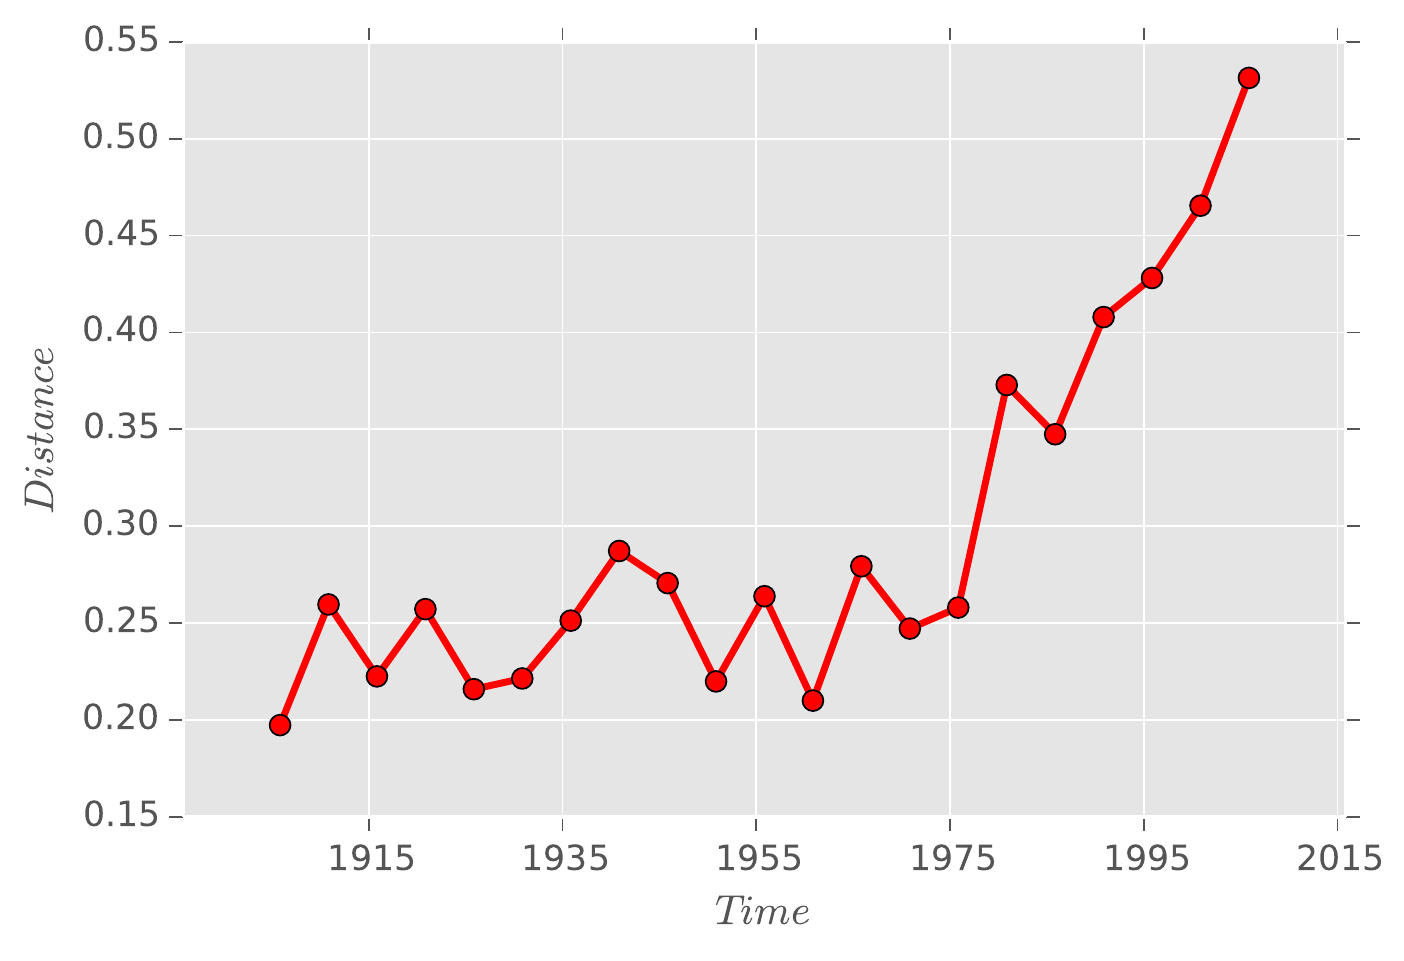}
  \caption{gay}
  \label{fig:embfig1}
\end{subfigure}%
\begin{subfigure}{0.25\textwidth}
  \centering
  \includegraphics[width=\textwidth]{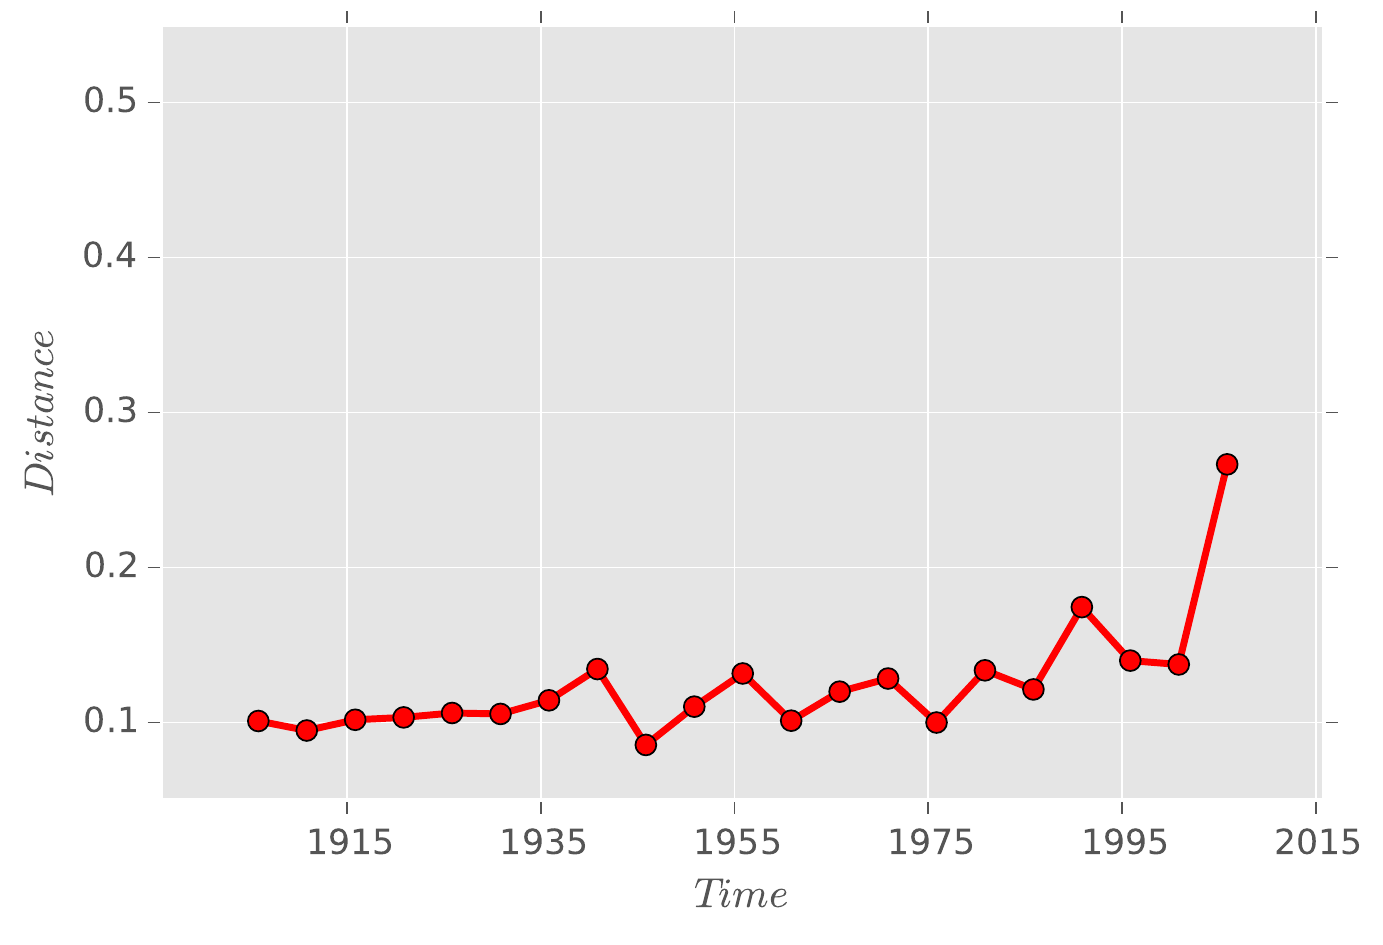}
  \caption{God}
  \label{fig:embfig2}
\end{subfigure}%
\caption{Distributional time series for \texttt{gay}, \texttt{God} over time using word embeddings. Observe the change around 1970 for \texttt{gay} while \texttt{God} is fairly stable.}
%\label{fig:embeddings}
\end{figure}

Figure \ref{fig:vis_embeddings} shows a multi-dimensional scaling of some region in the word embedding space. Note how the nearest neighbors reflect both syntactic and semantic similarities among words.
\begin{figure}
  \centering
  \includegraphics[trim= 0 0 0 0, clip=true,width = 0.5\textwidth]{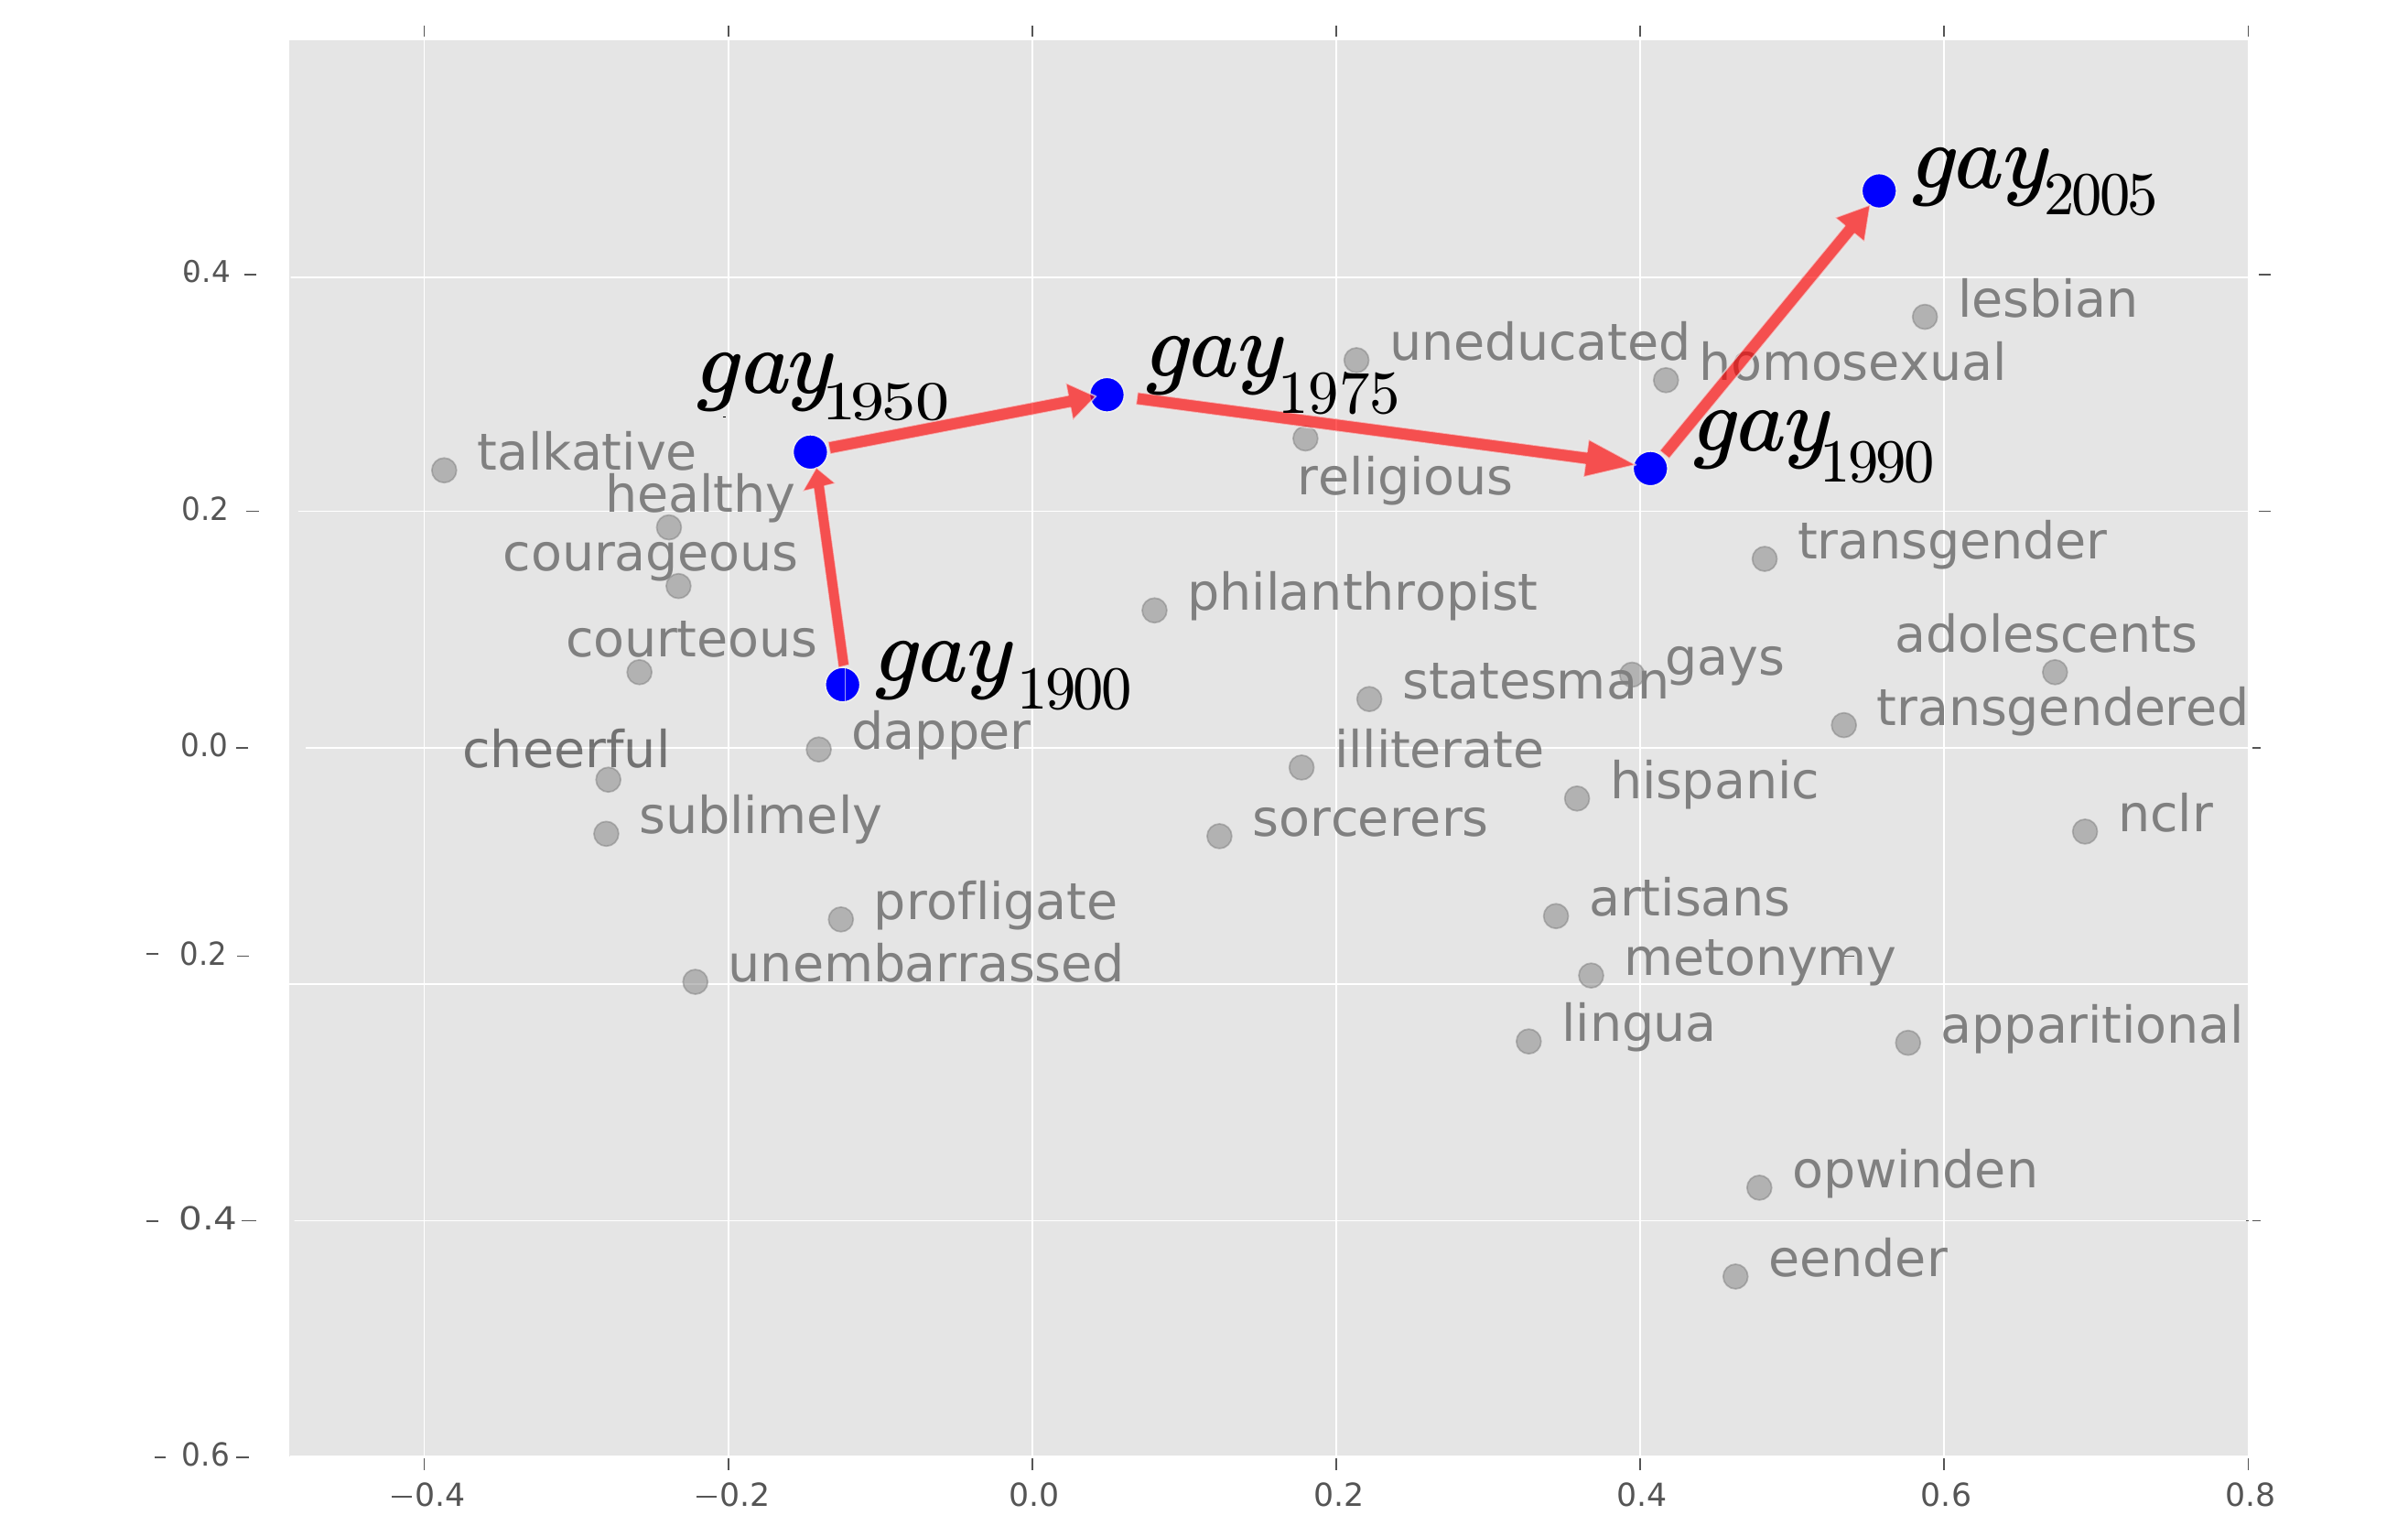}
  \caption{\small Trajectory of the word \emph{gay} in embedding space.}
%  \label{fig:vis_embeddings}
\end{figure}

\begin{table}[thb]
\begin{tabular}{l|l}
Donor Word($w_d$) & Recipient Word($w_r$) \\ \hline
glass & strength \\
football & sex \\
location & equation \\
hand & rock \\
\end{tabular}
\caption{Sample list of word pairs}
%\label{tab:wordpairs}
\end{table}

\begin{table*}
\centering
\begin{tabular}{m{2cm}|m{4cm} m{4cm} m{4cm}}

\textbf{Word} & \textbf{Frequency} & \textbf{Part of Speech} & \textbf{\dist} \\
 & & & \\
\texttt{transmitted} & \includegraphics[scale=0.25]{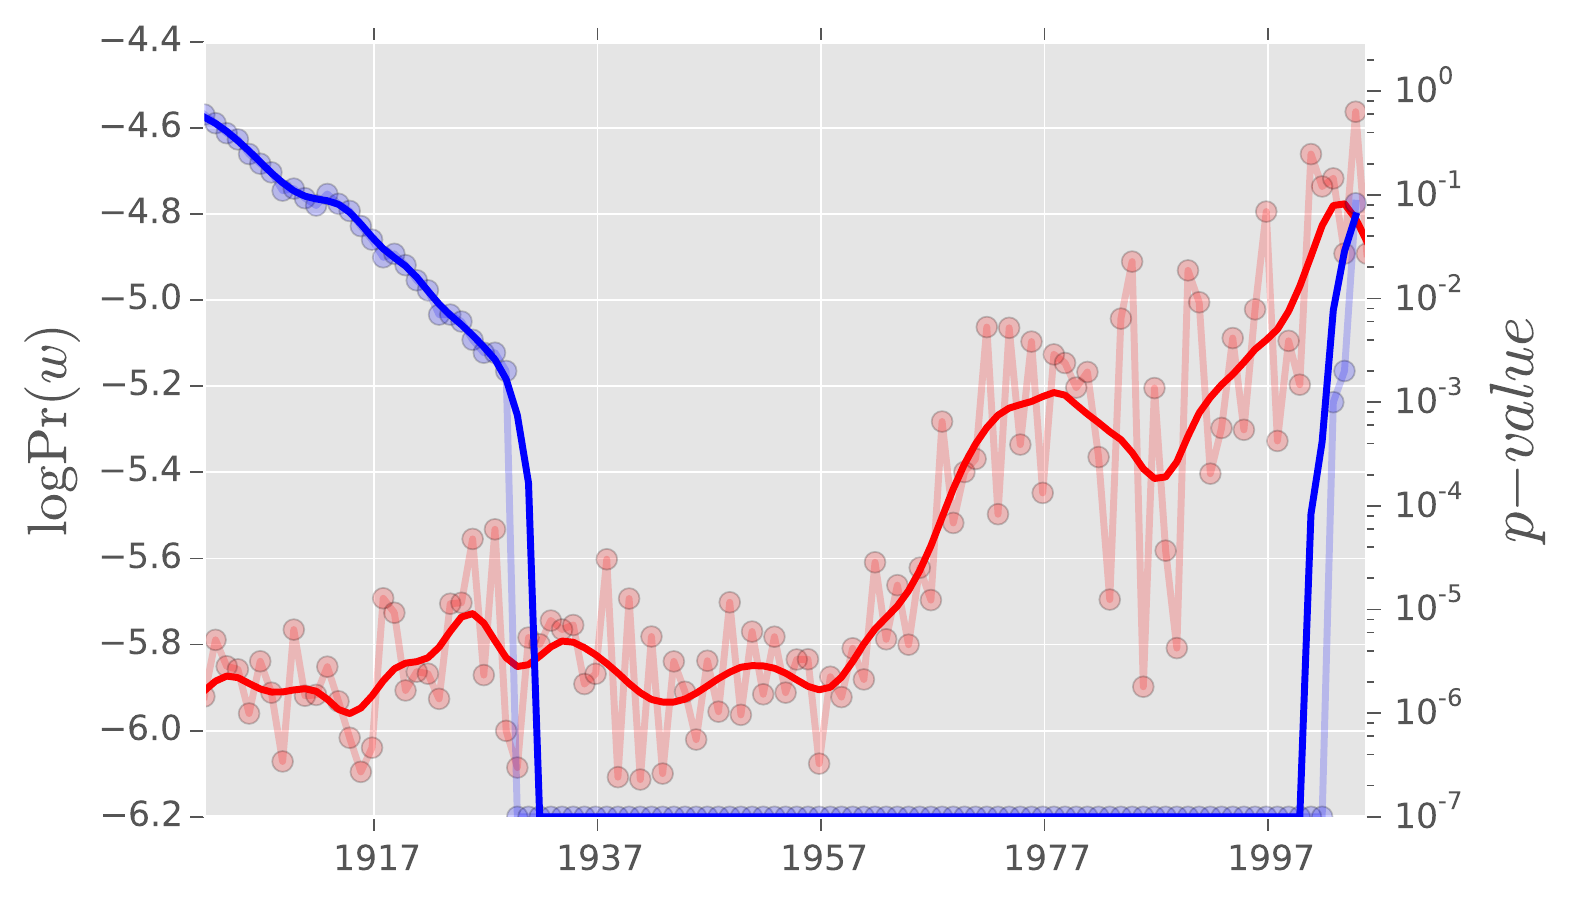} & \includegraphics[scale=0.25]{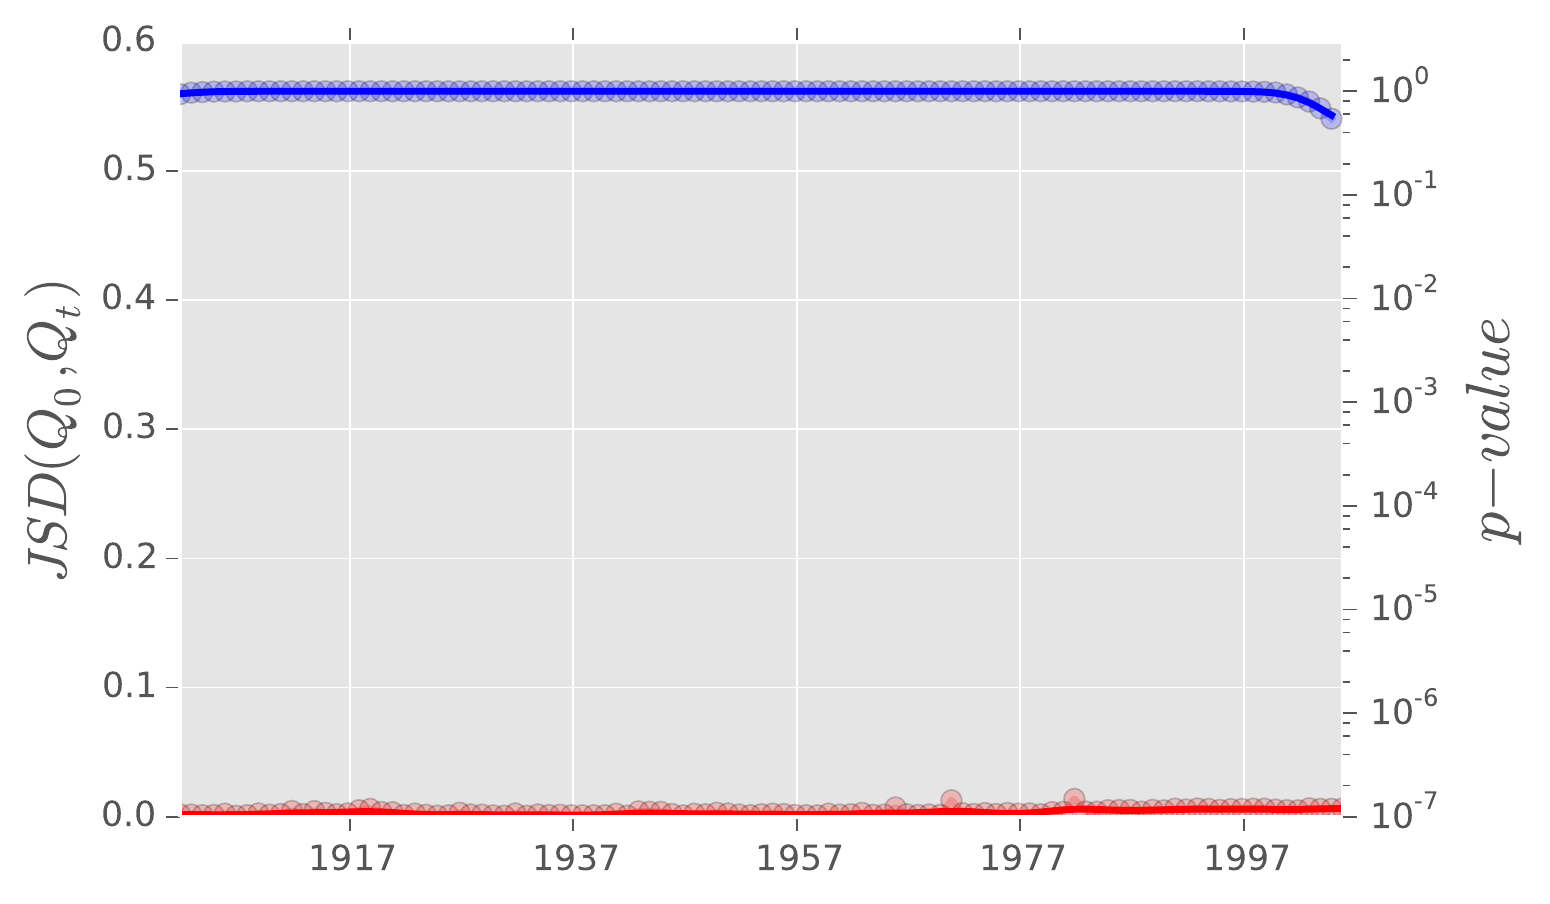} & \includegraphics[scale=0.25]{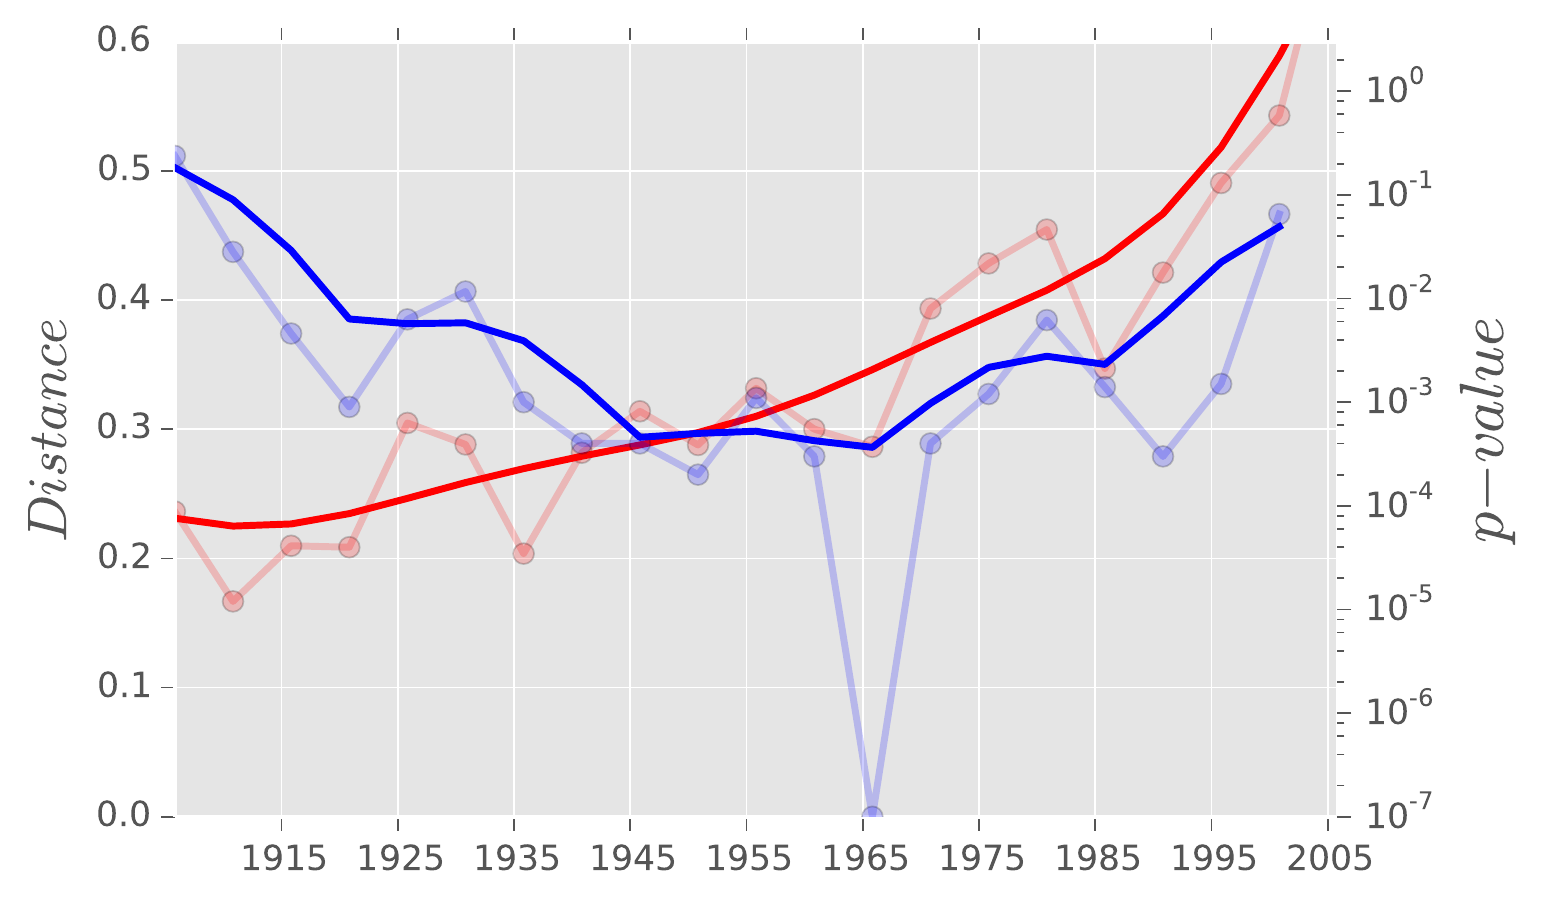}\\

\texttt{bitch} & \includegraphics[scale=0.25]{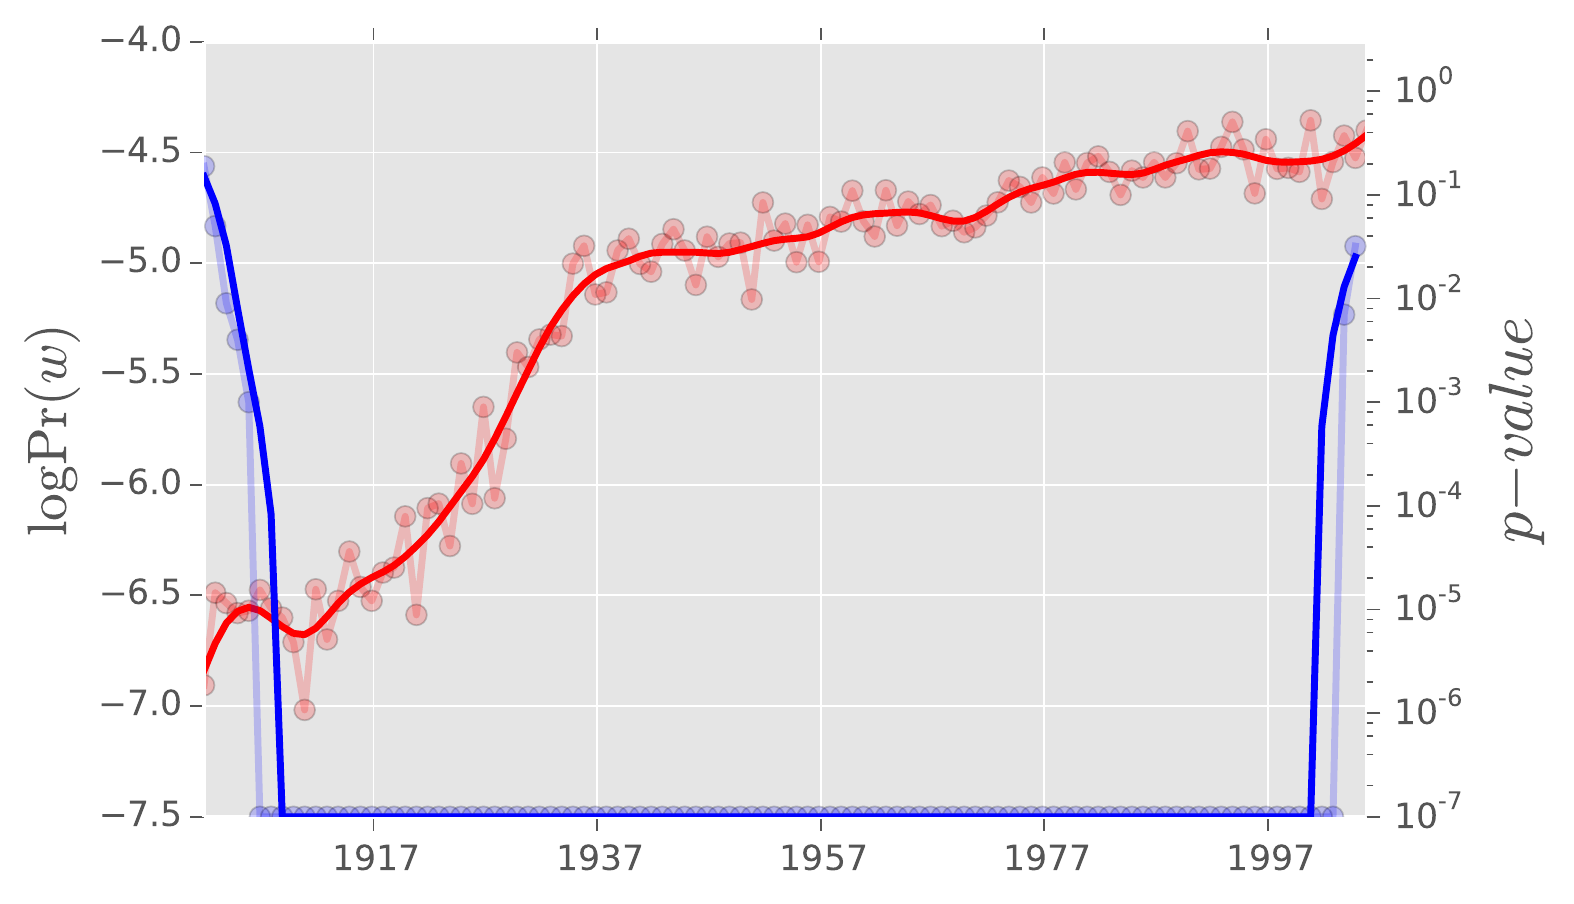}& \includegraphics[scale=0.25]{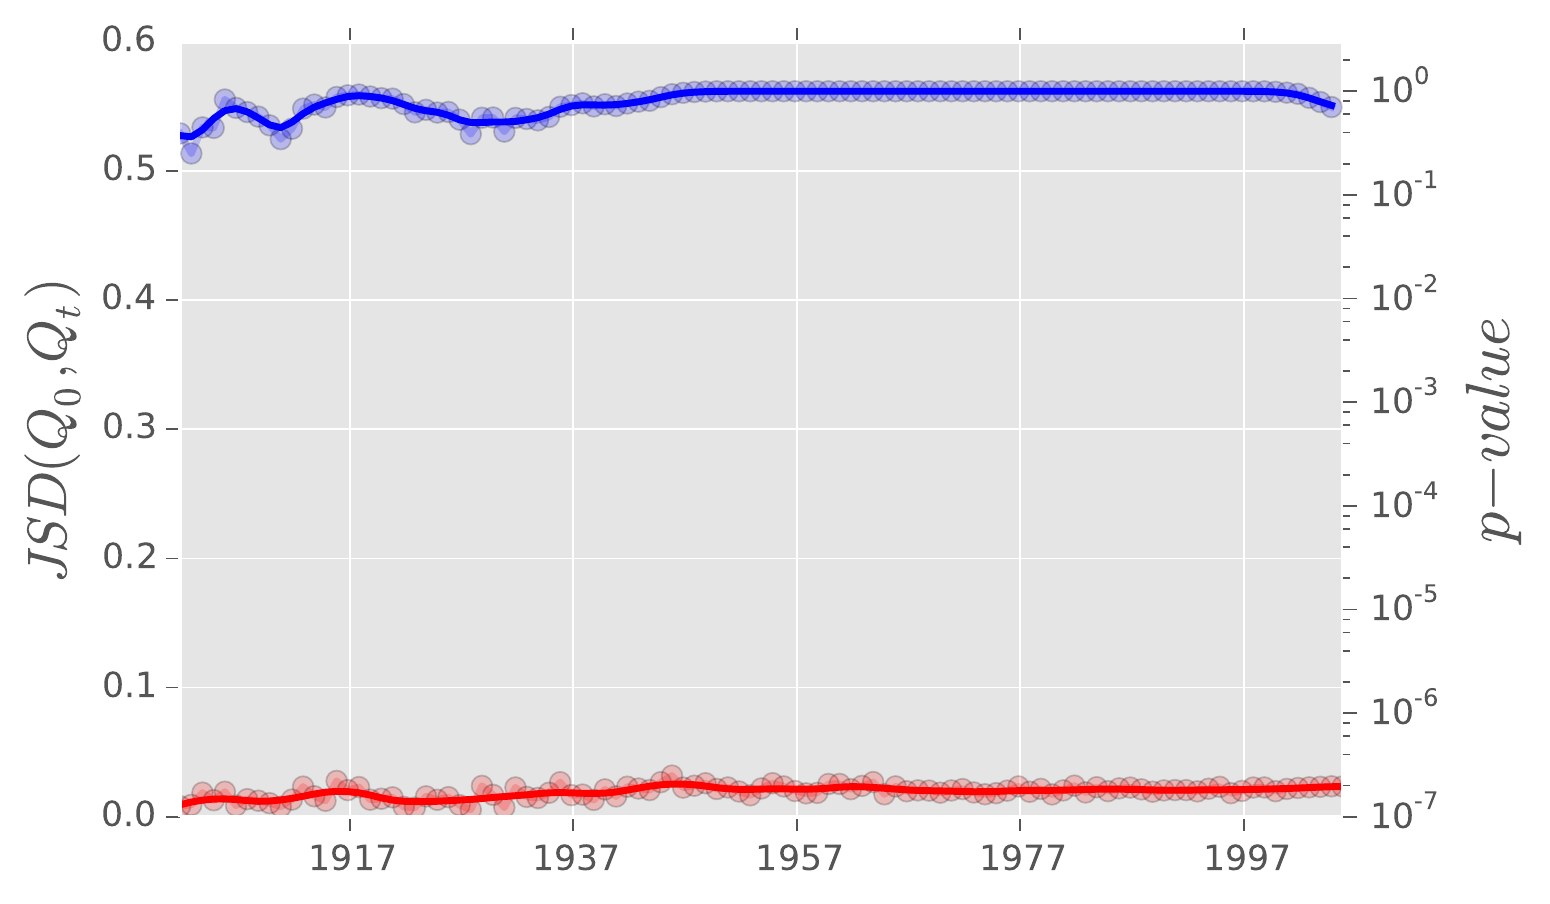} & \includegraphics[scale=0.25]{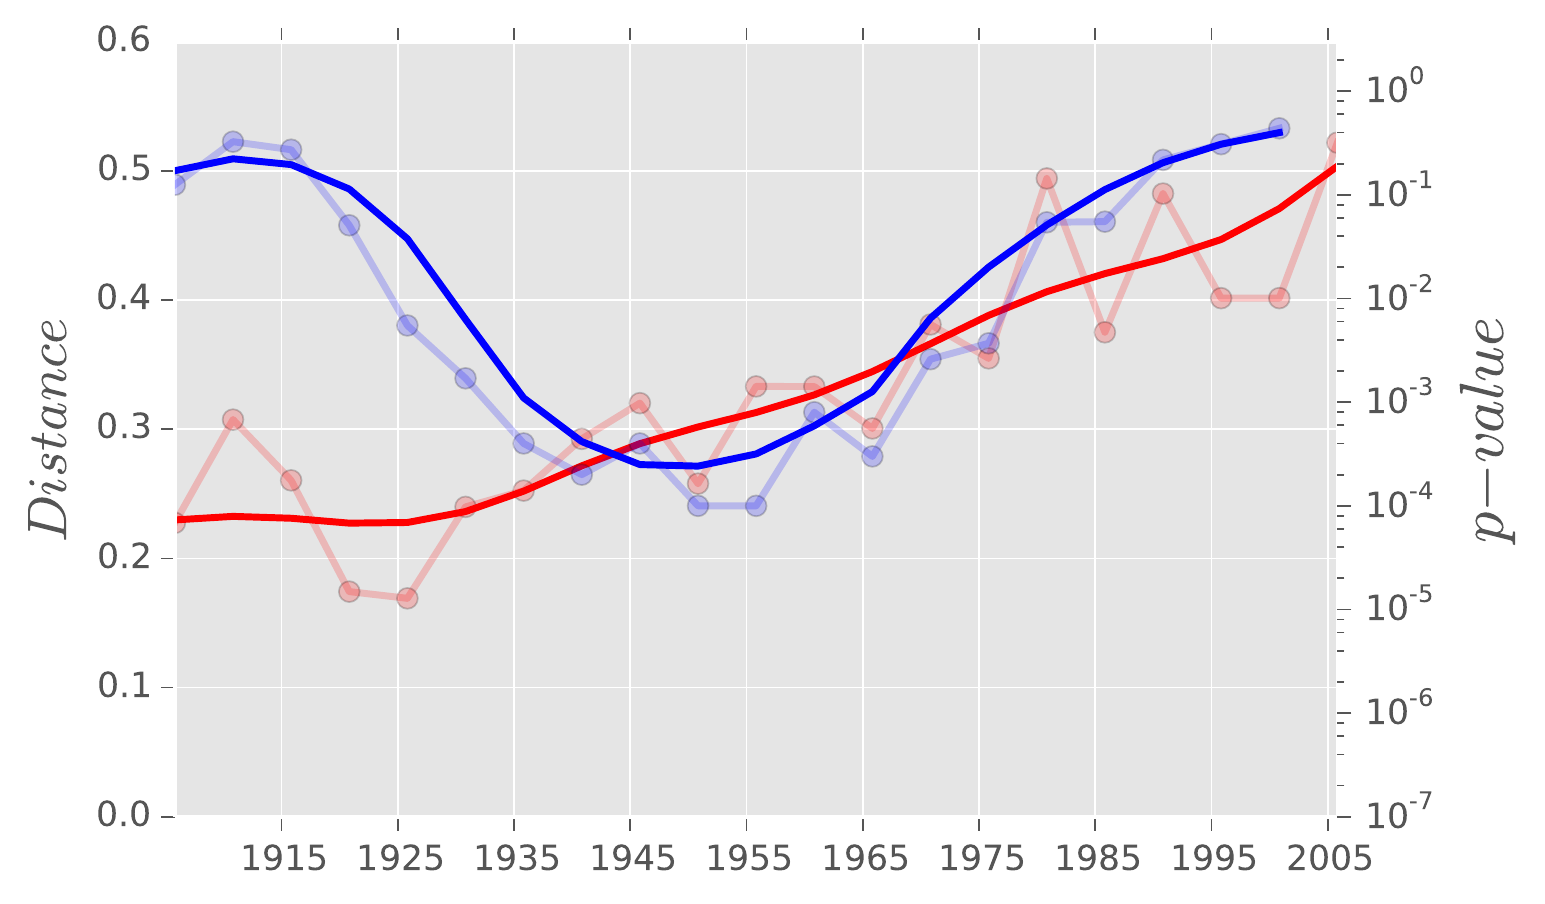}\\

%\texttt{gay} & \includegraphics[scale=0.25]{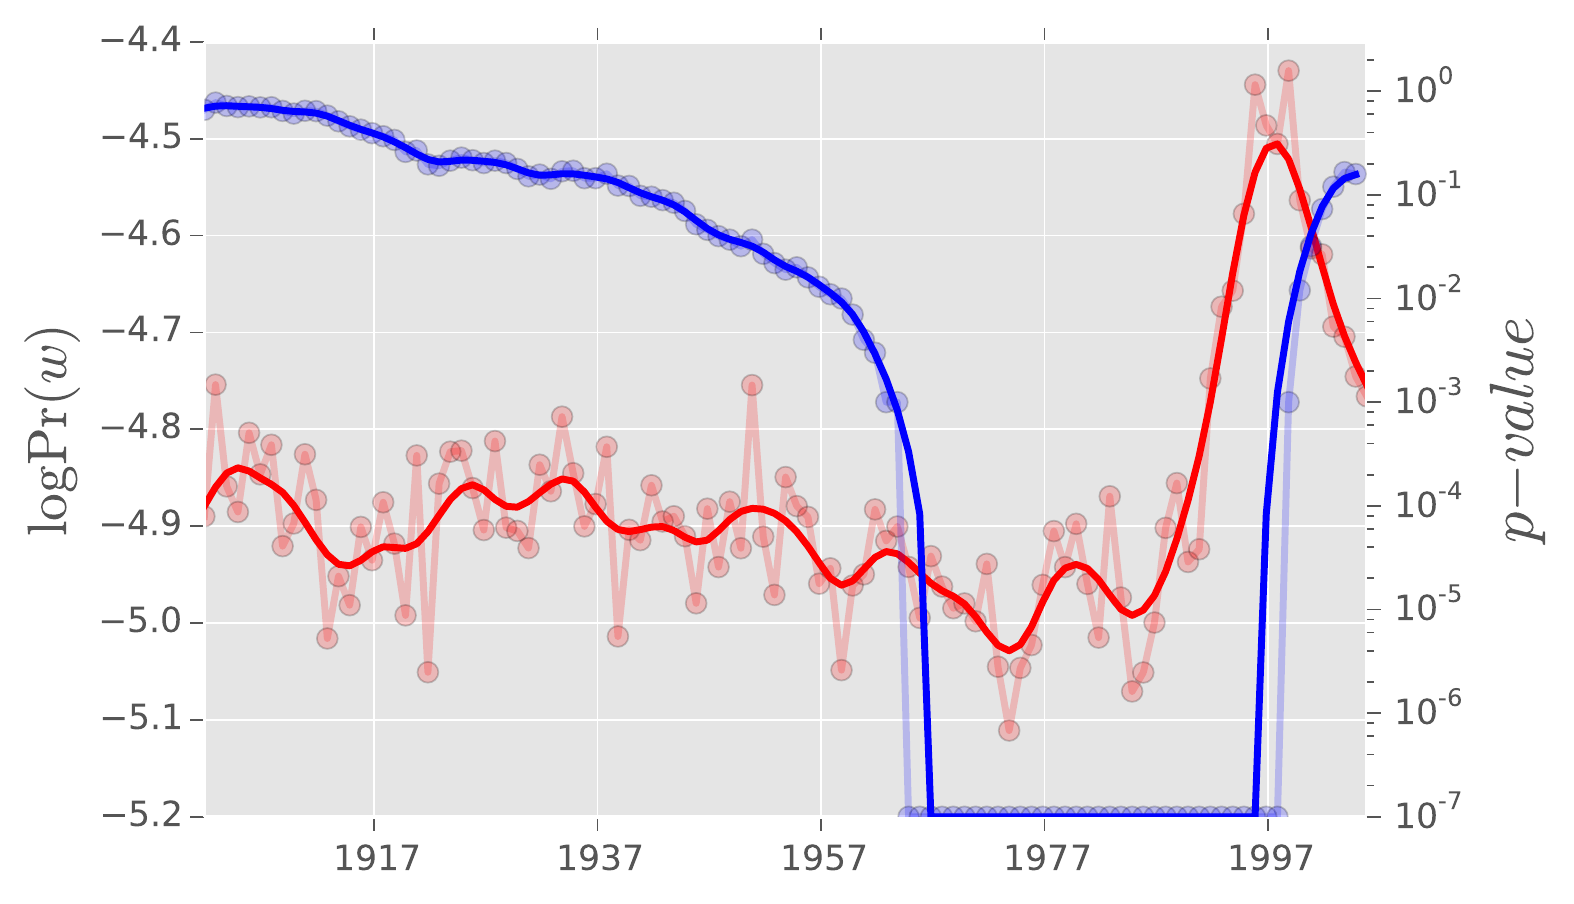}& %\includegraphics[scale=0.25]{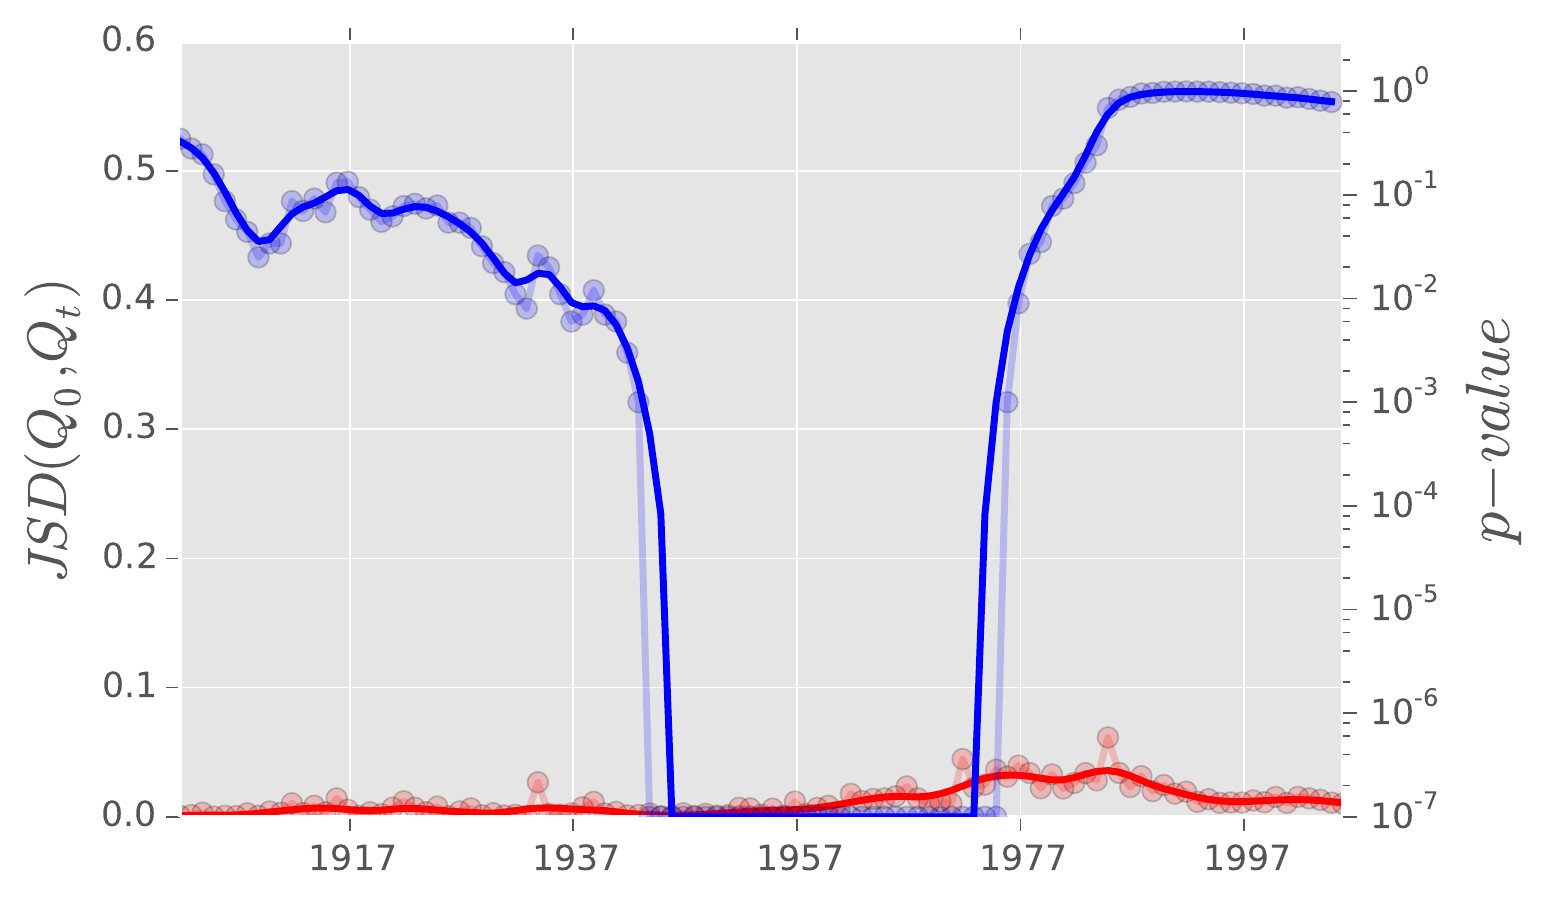} & \includegraphics[scale=0.25]{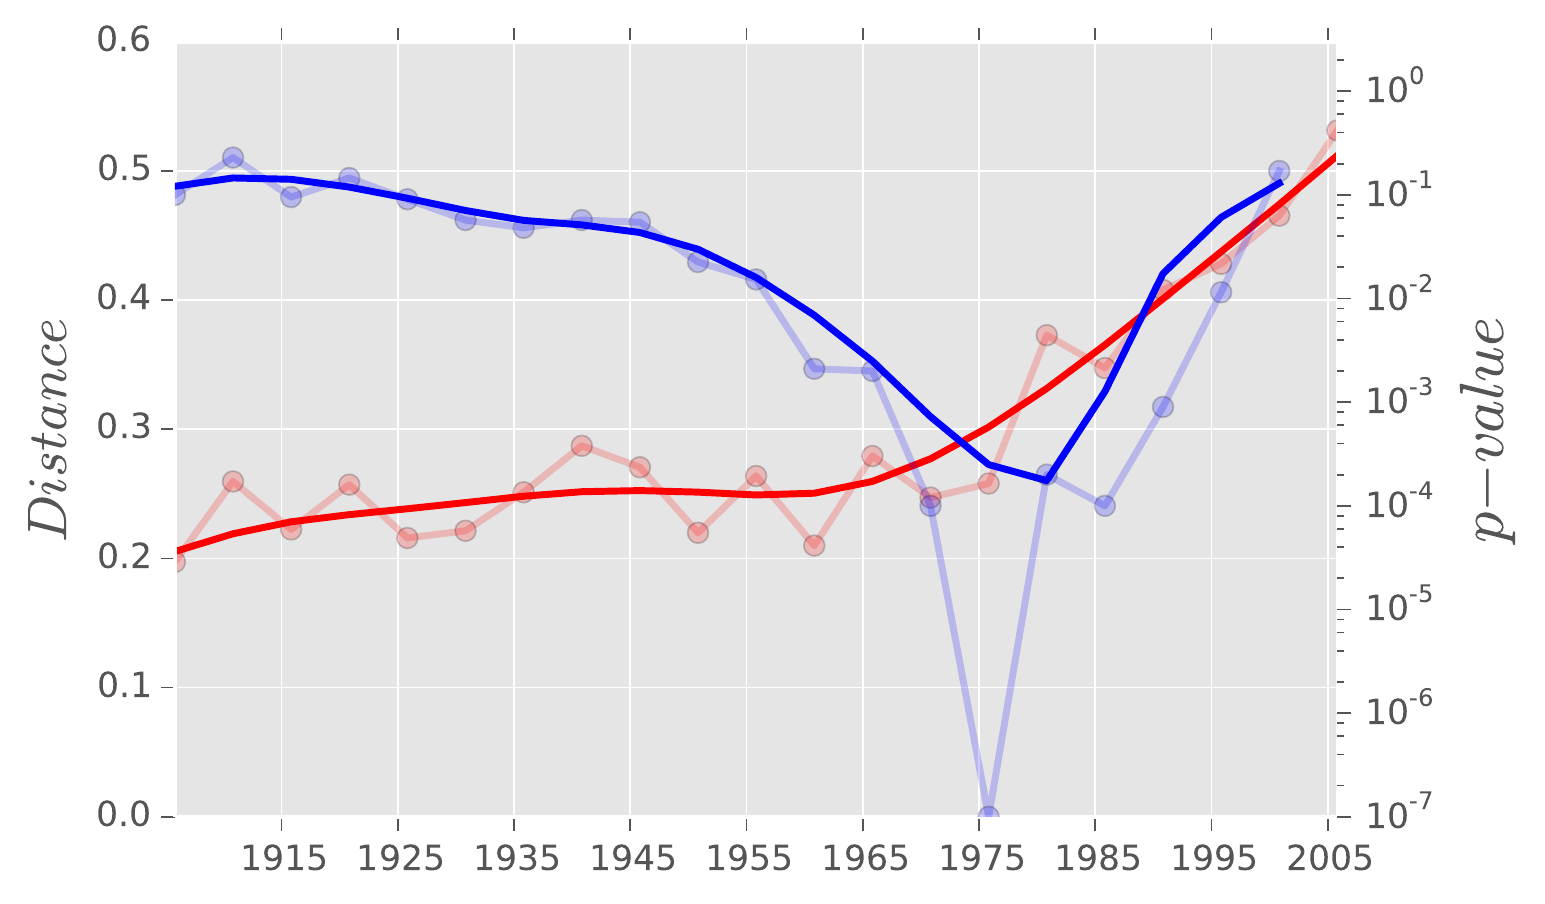}\\

%\newline
\texttt{her} & \includegraphics[scale=0.25]{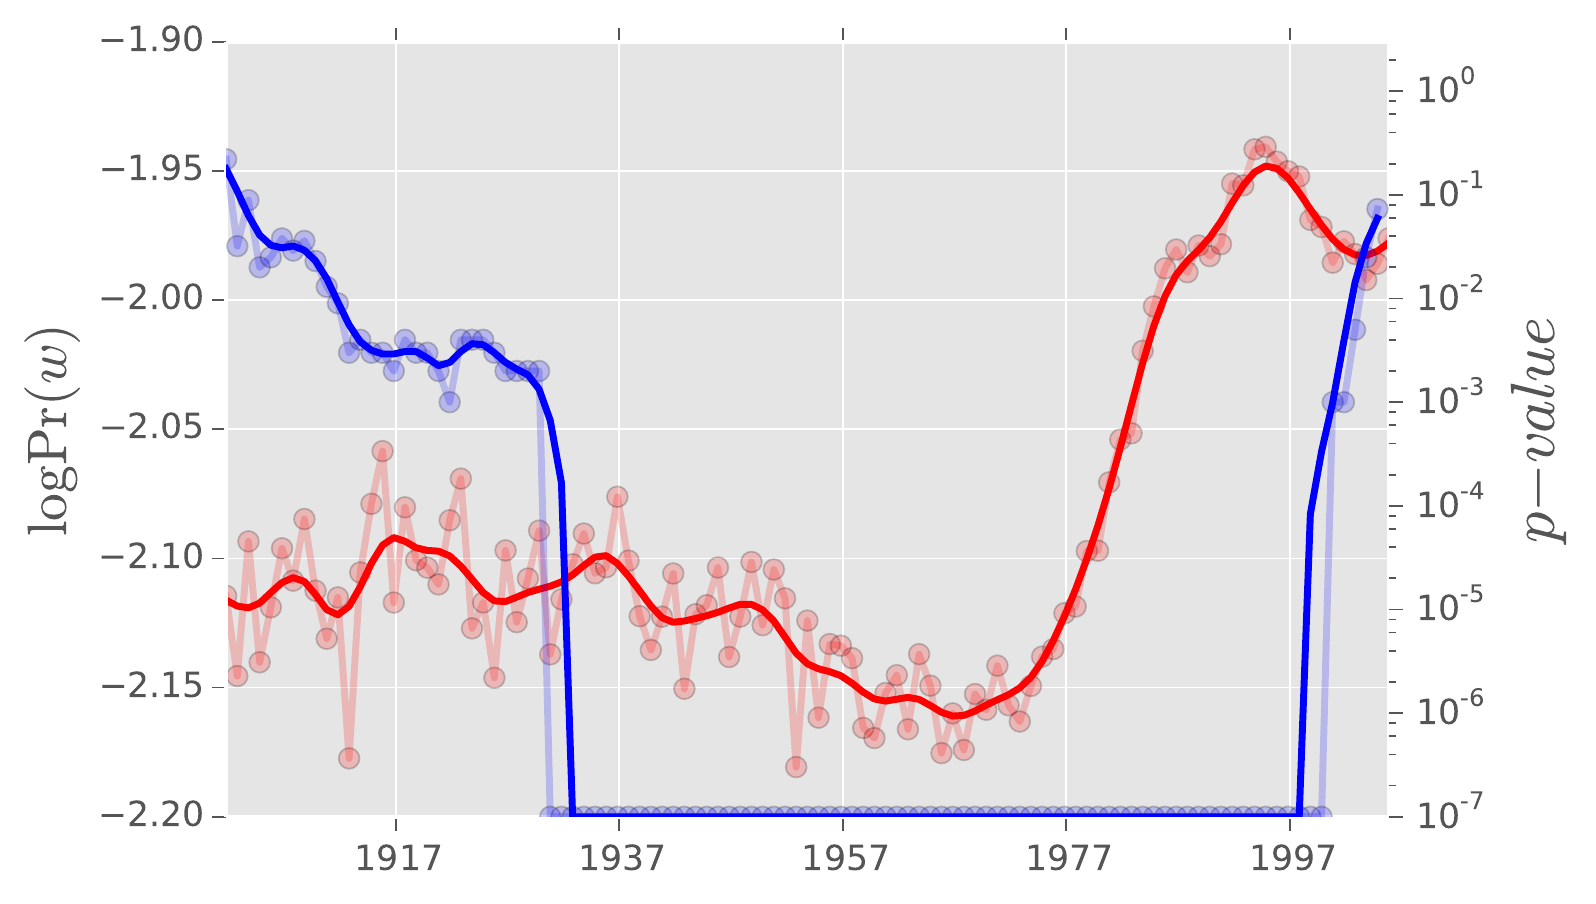}& \includegraphics[scale=0.25]{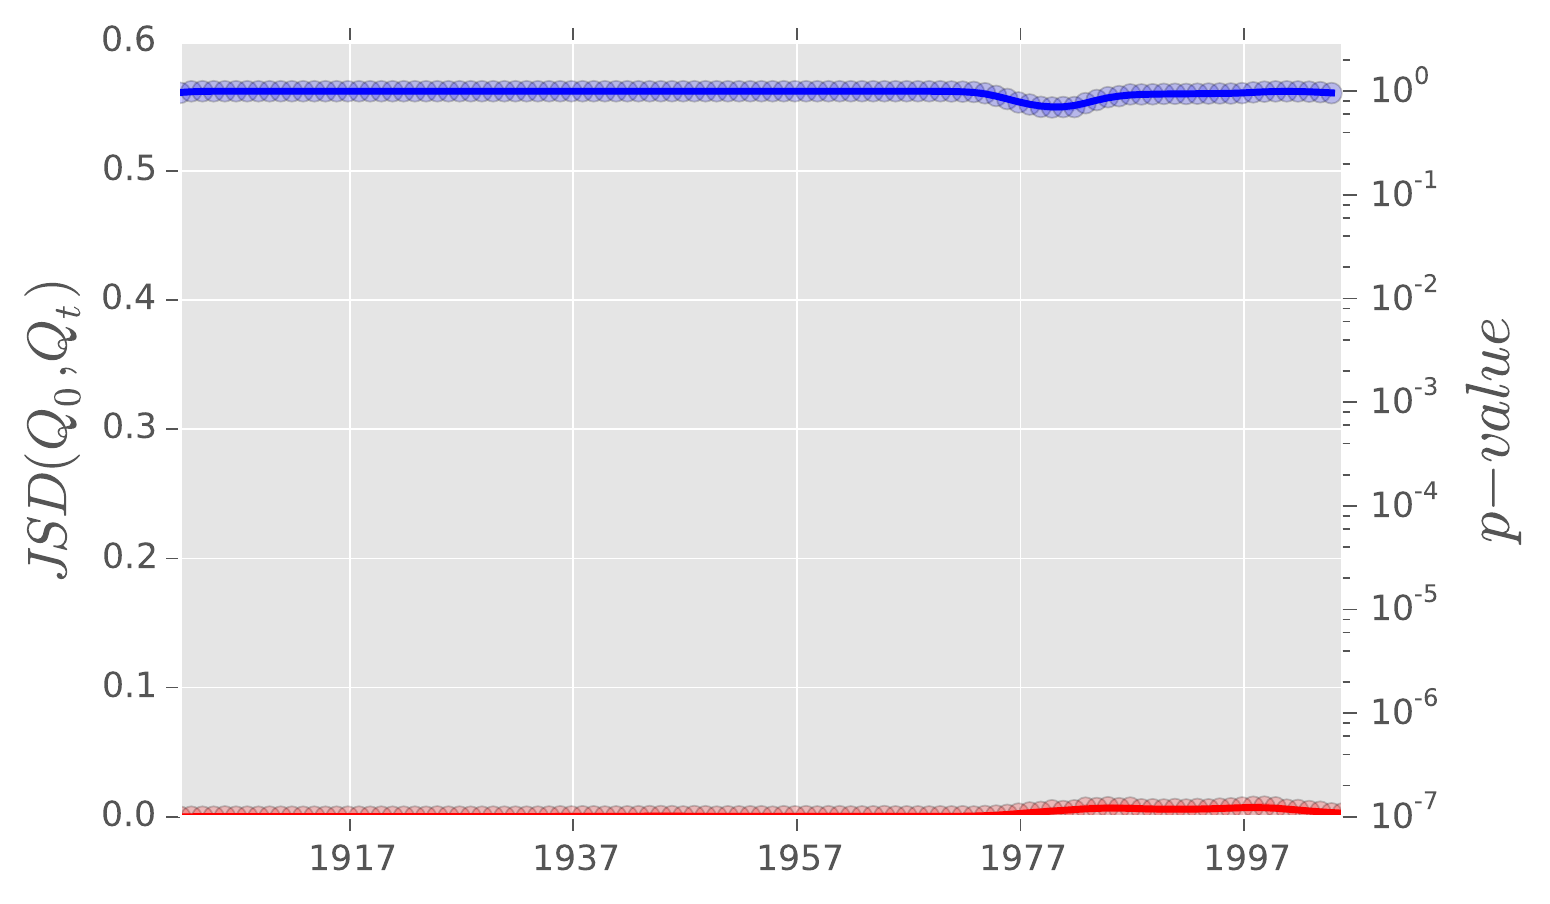} & \includegraphics[scale=0.25]{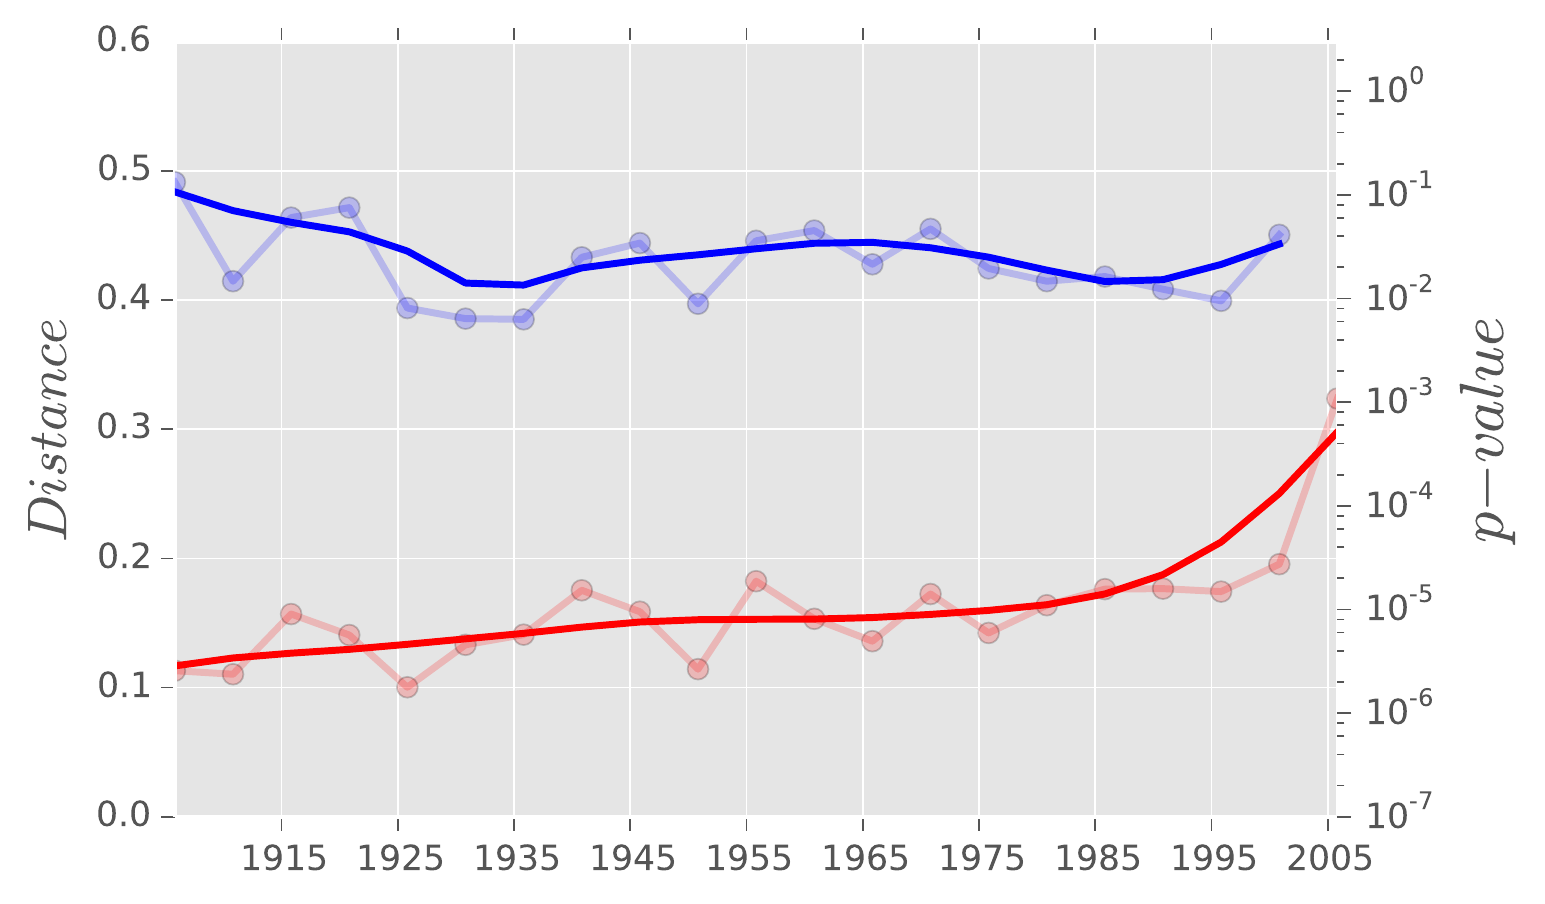}\\ %\newline
\texttt{sex} & \includegraphics[scale=0.25]{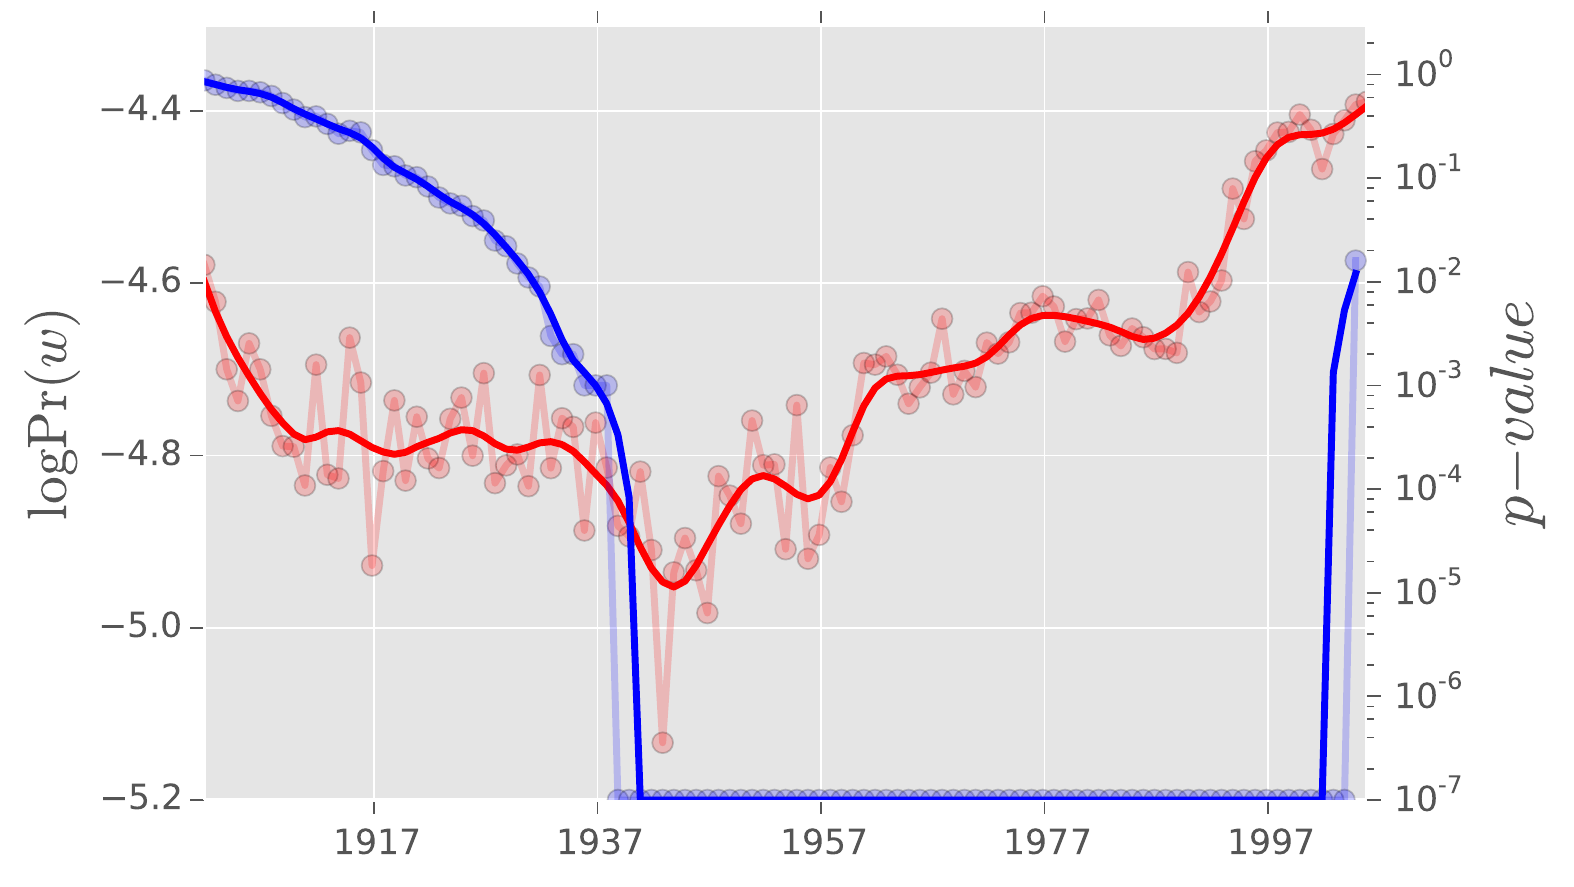}& \includegraphics[scale=0.25]{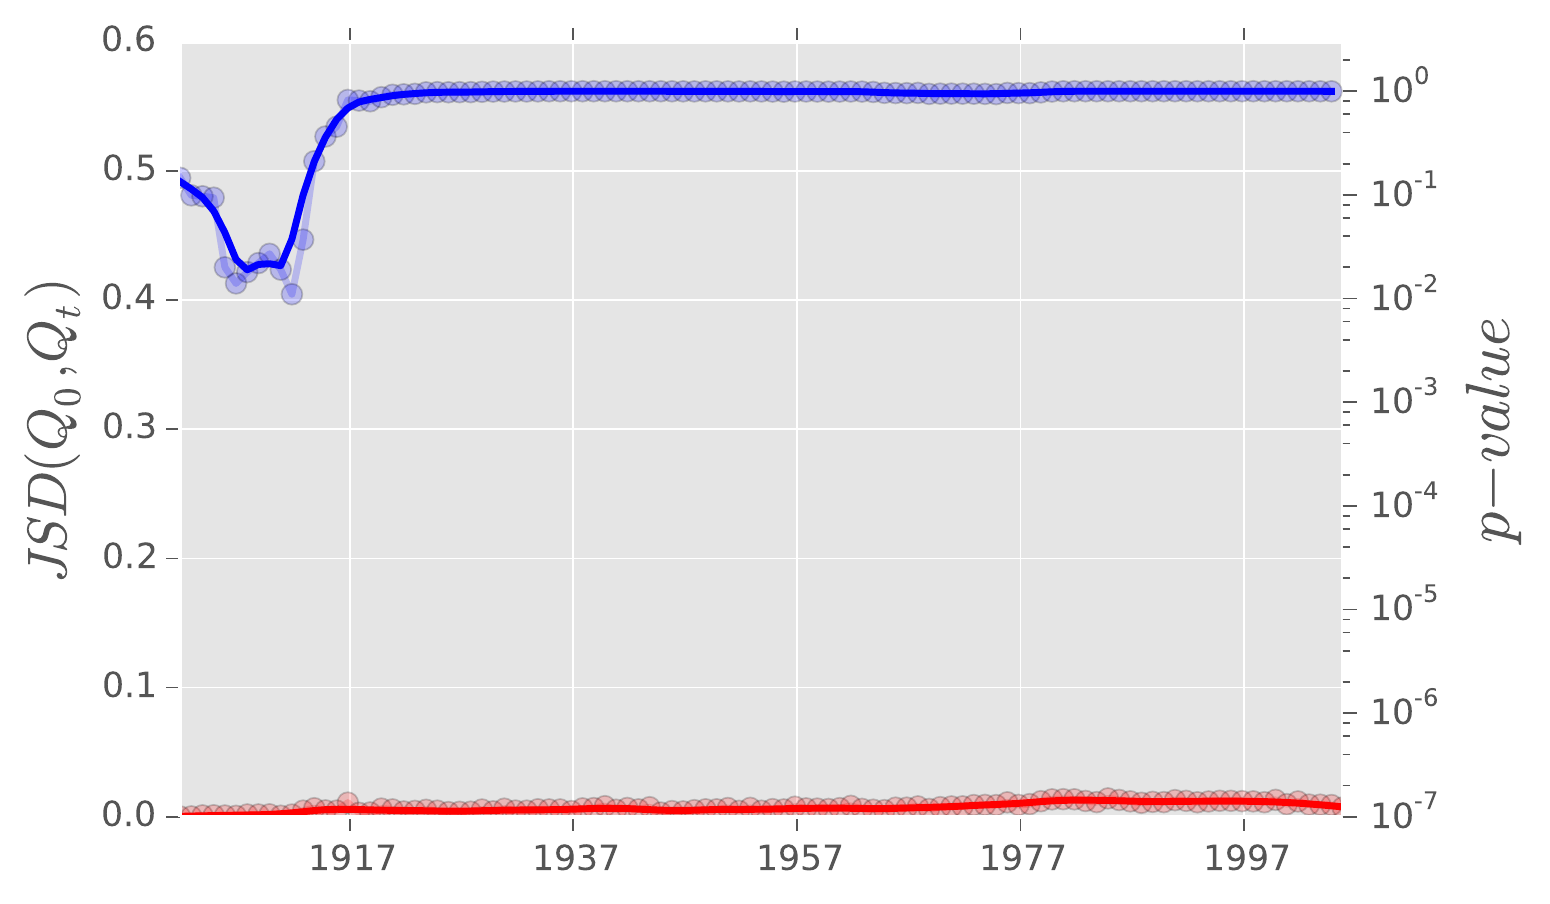} & \includegraphics[scale=0.25]{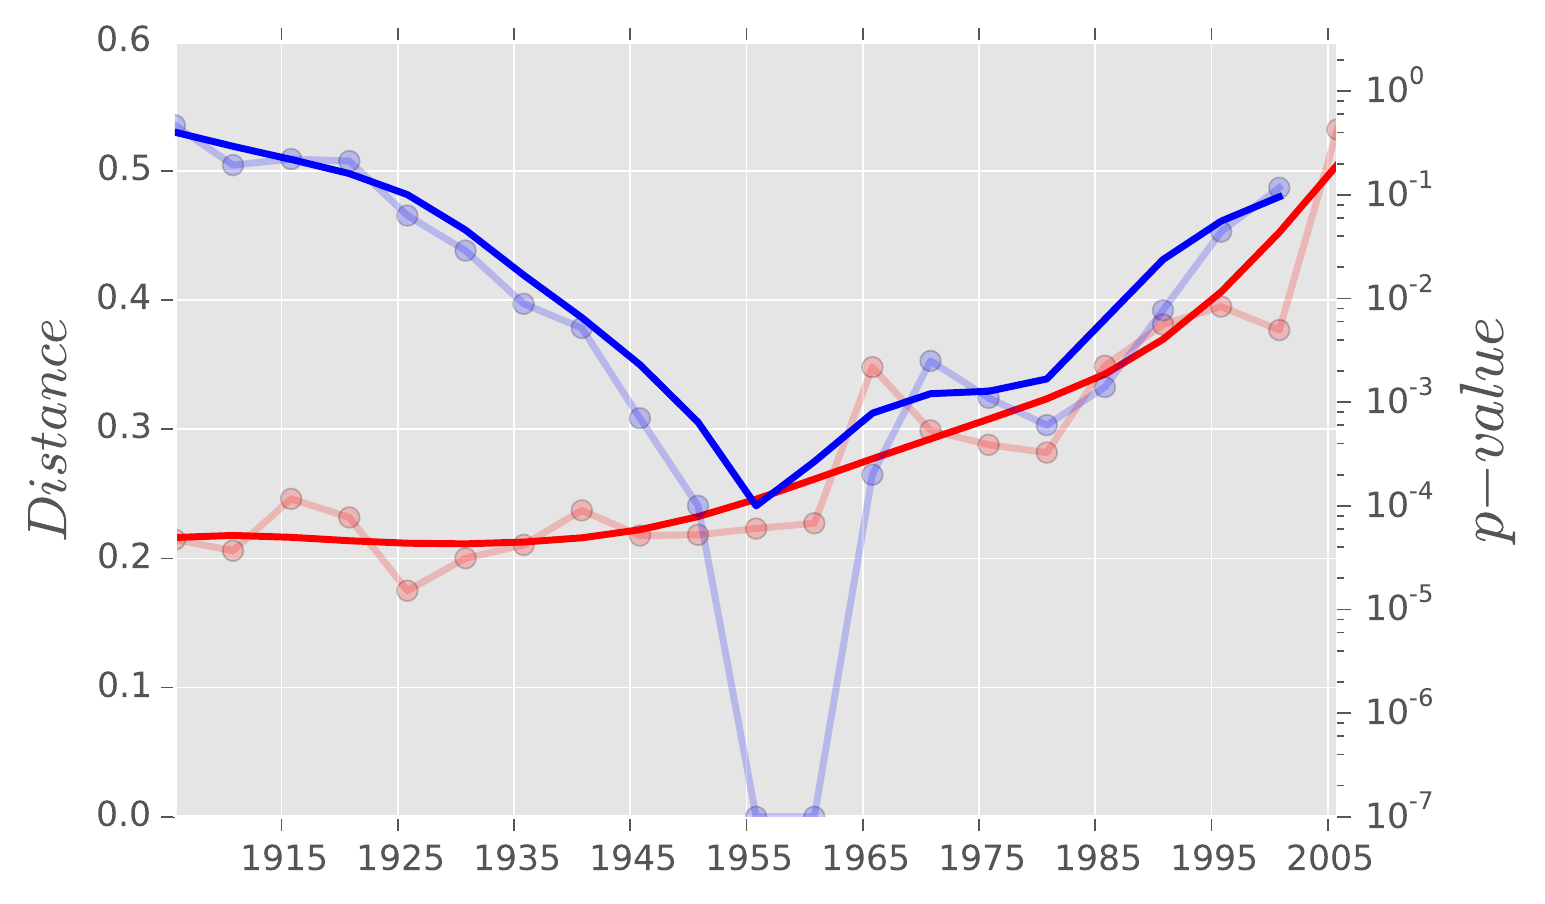}\\ %\newline
\texttt{apple} & \includegraphics[scale=0.25]{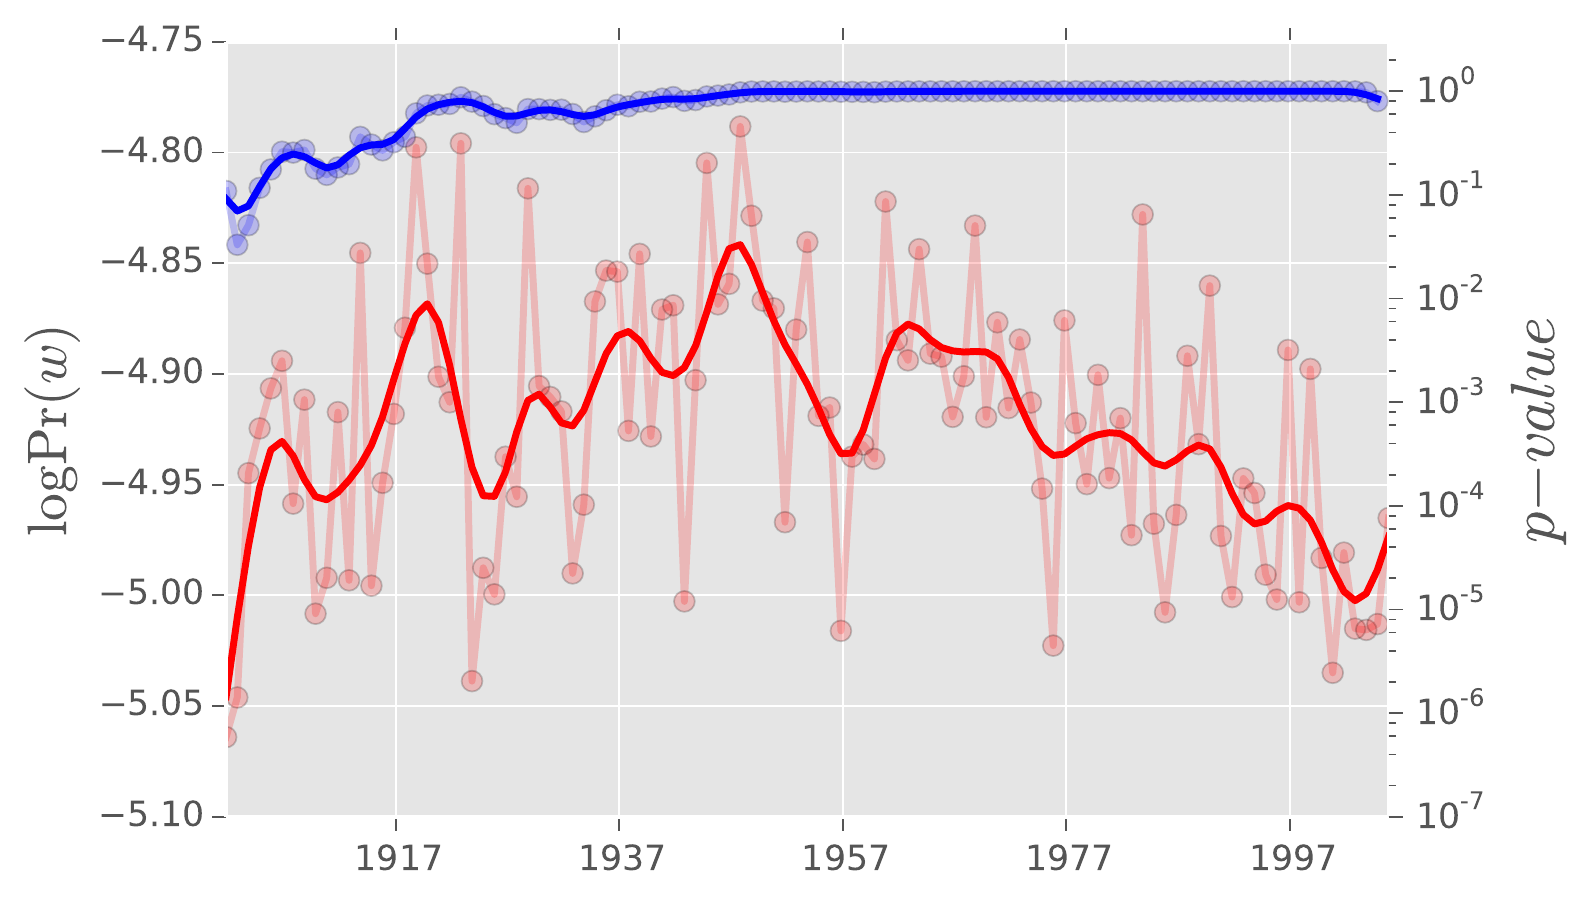}& \includegraphics[scale=0.25]{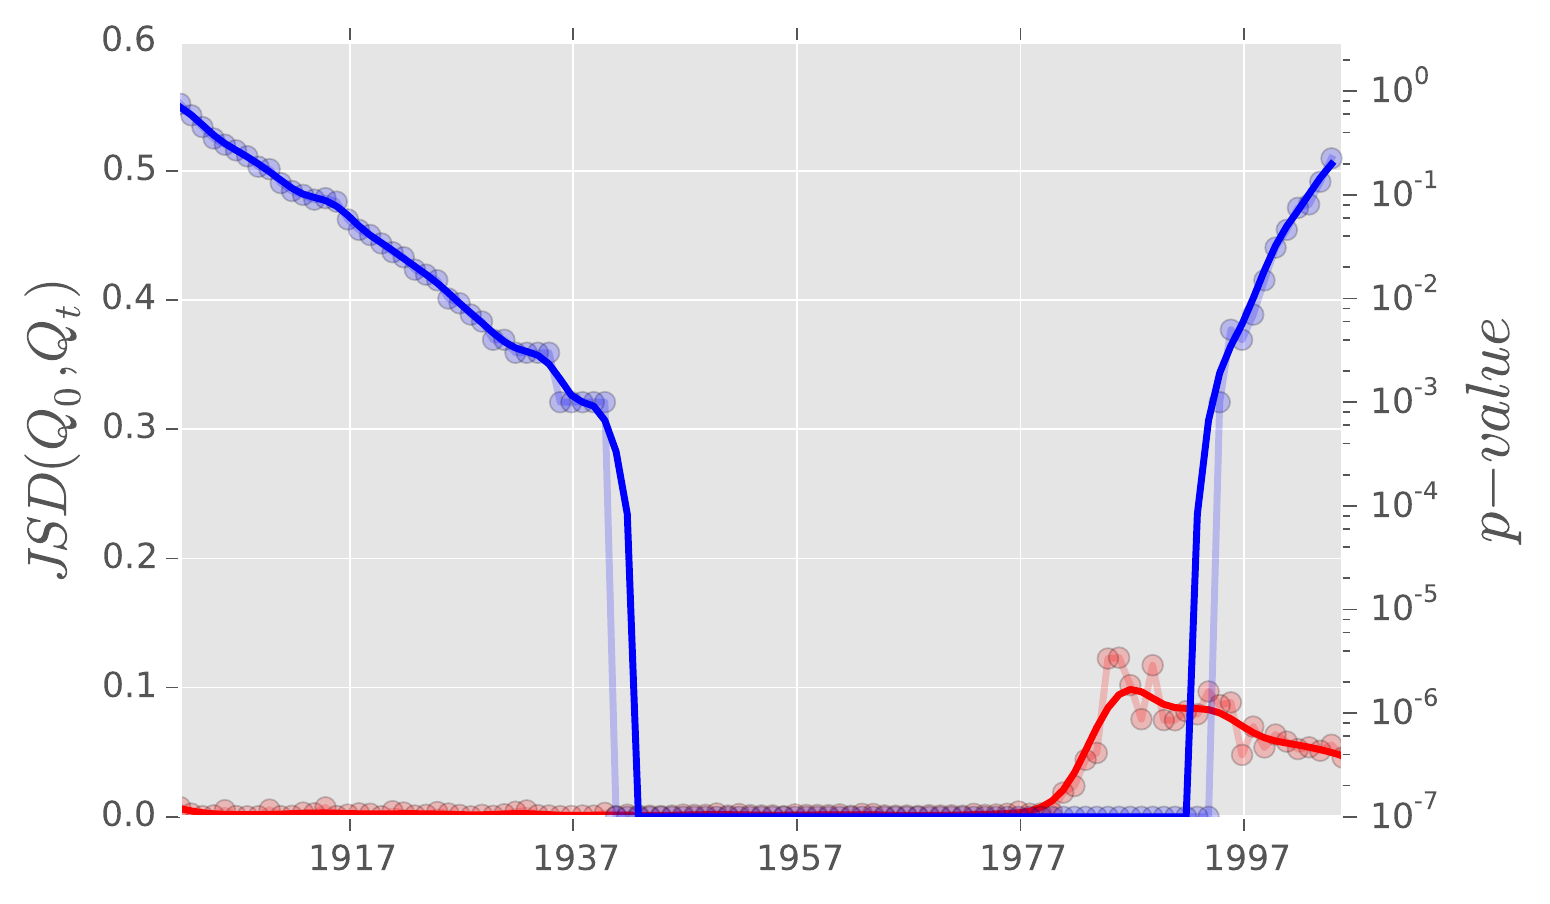} & \includegraphics[scale=0.25]{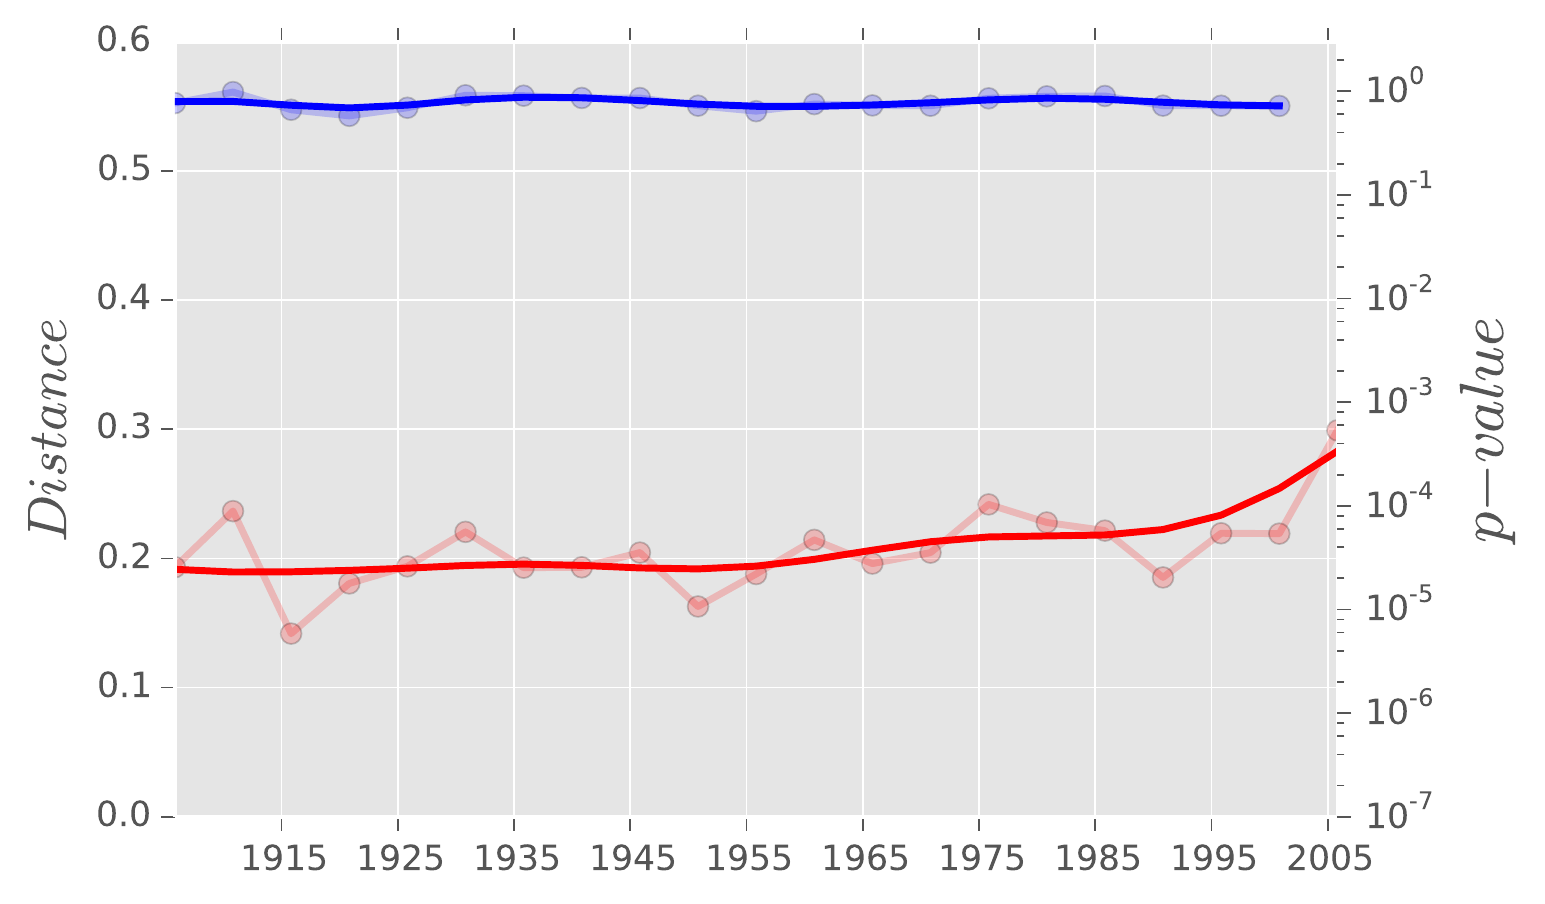}\\ %\newline
\texttt{diet} & \includegraphics[scale=0.25]{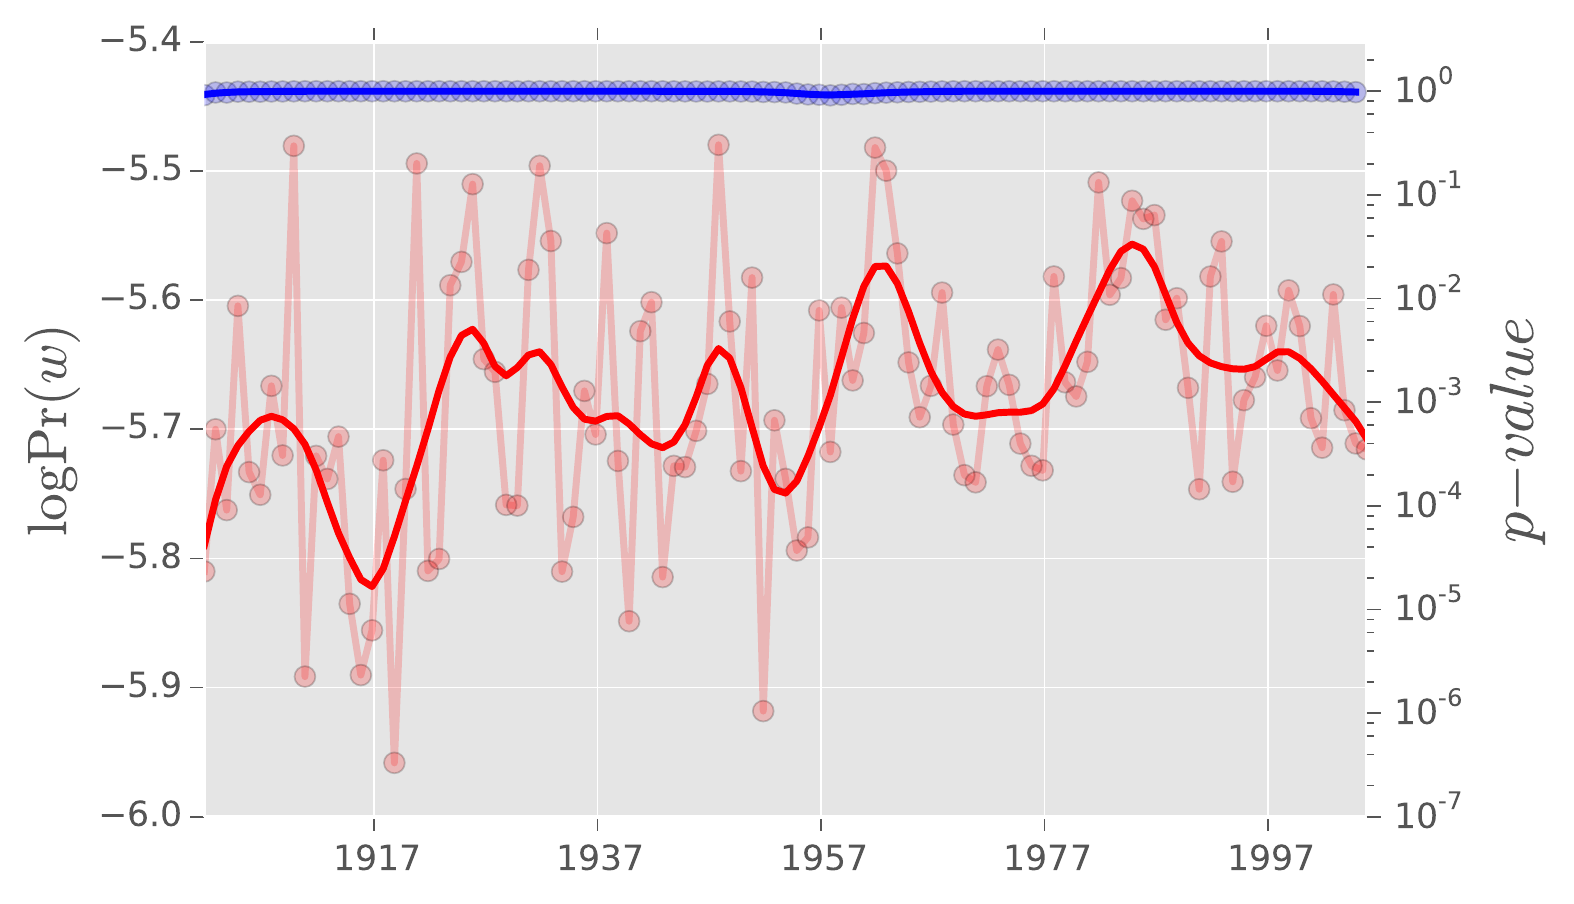}& \includegraphics[scale=0.25]{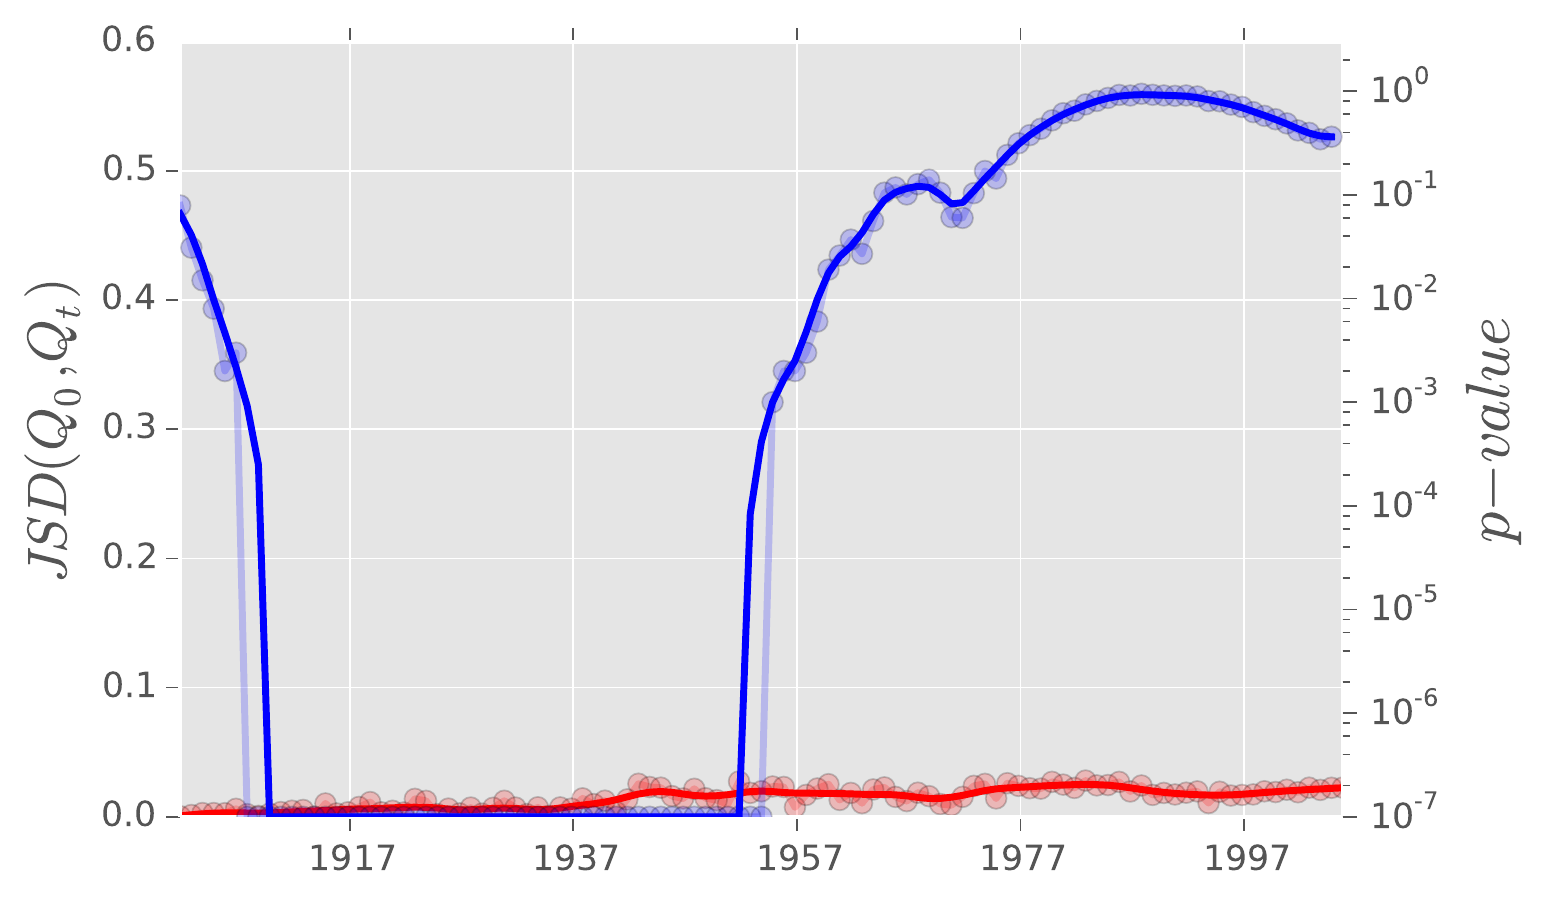} & \includegraphics[scale=0.25]{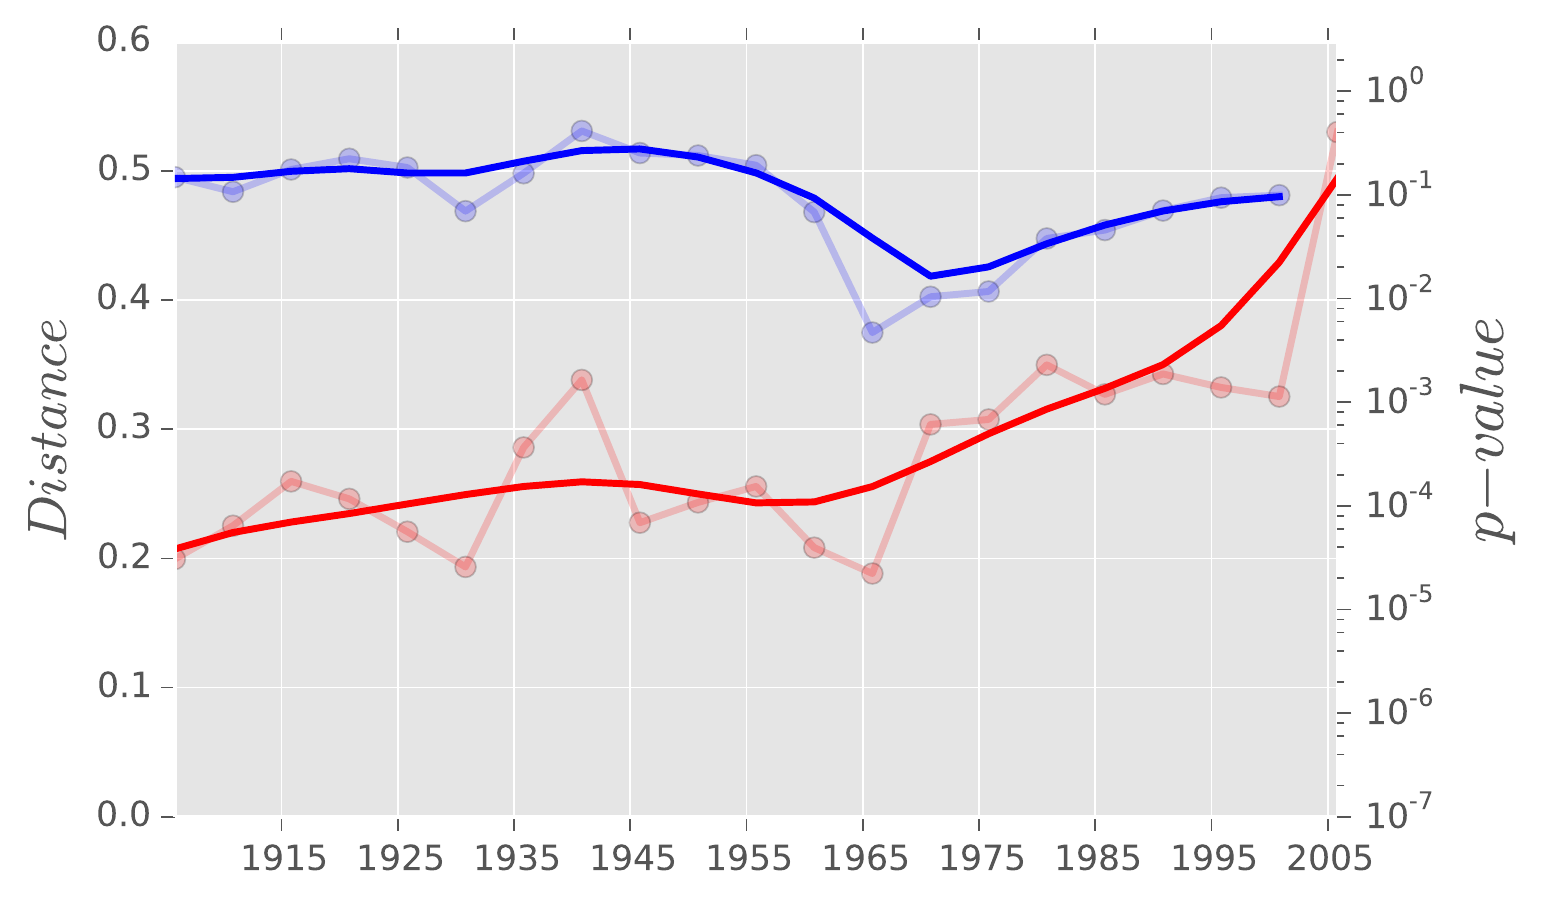} \\
\texttt{desk} & \includegraphics[scale=0.25]{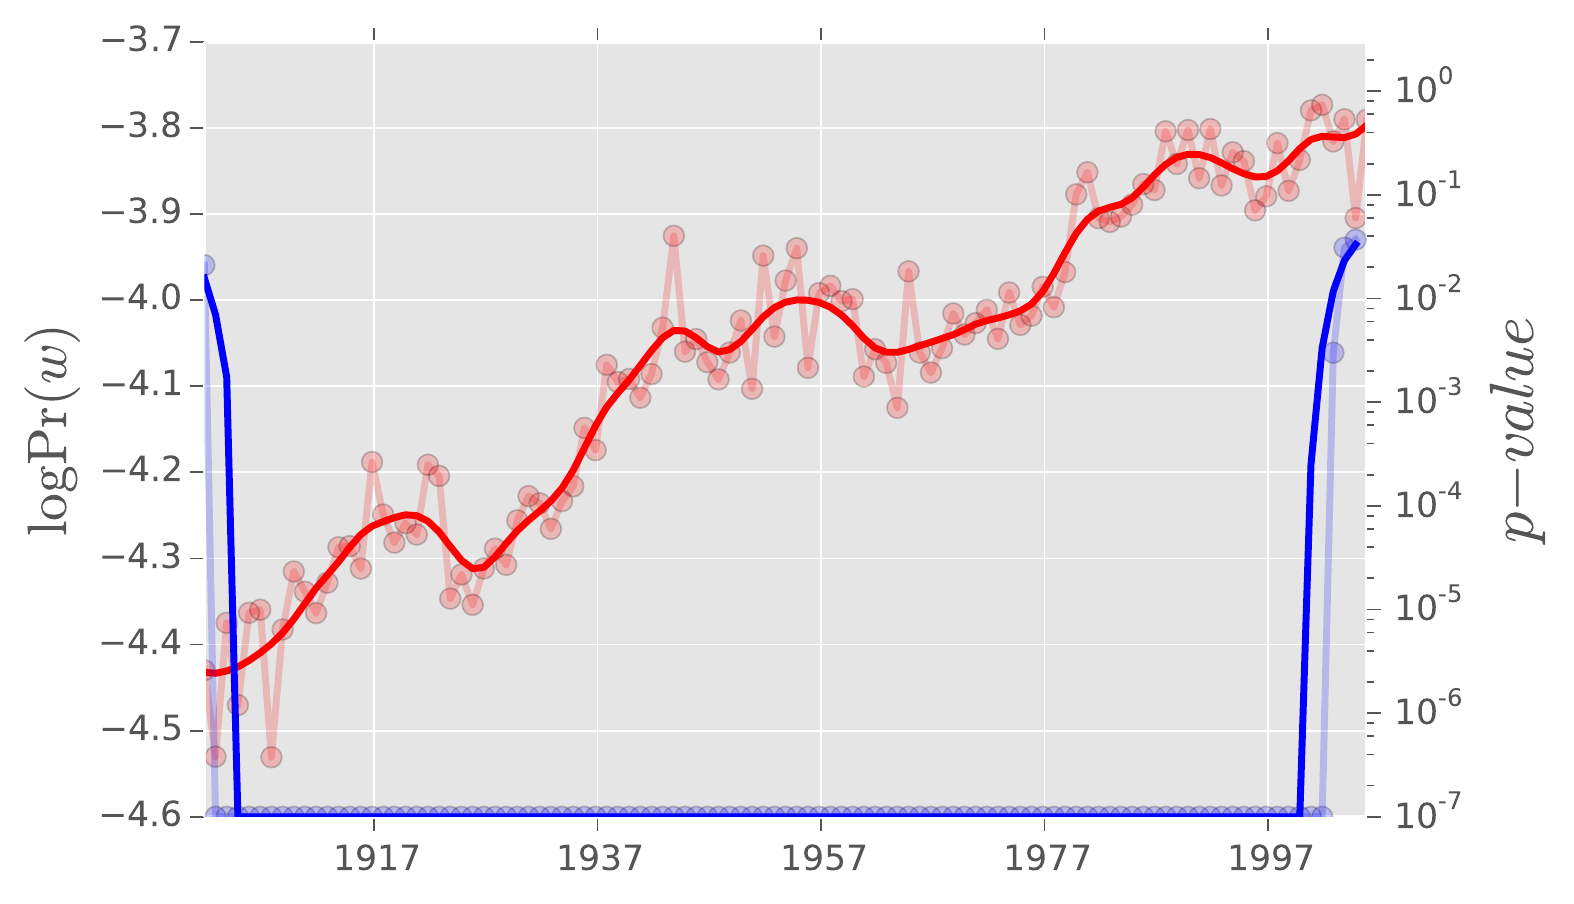}& \includegraphics[scale=0.25]{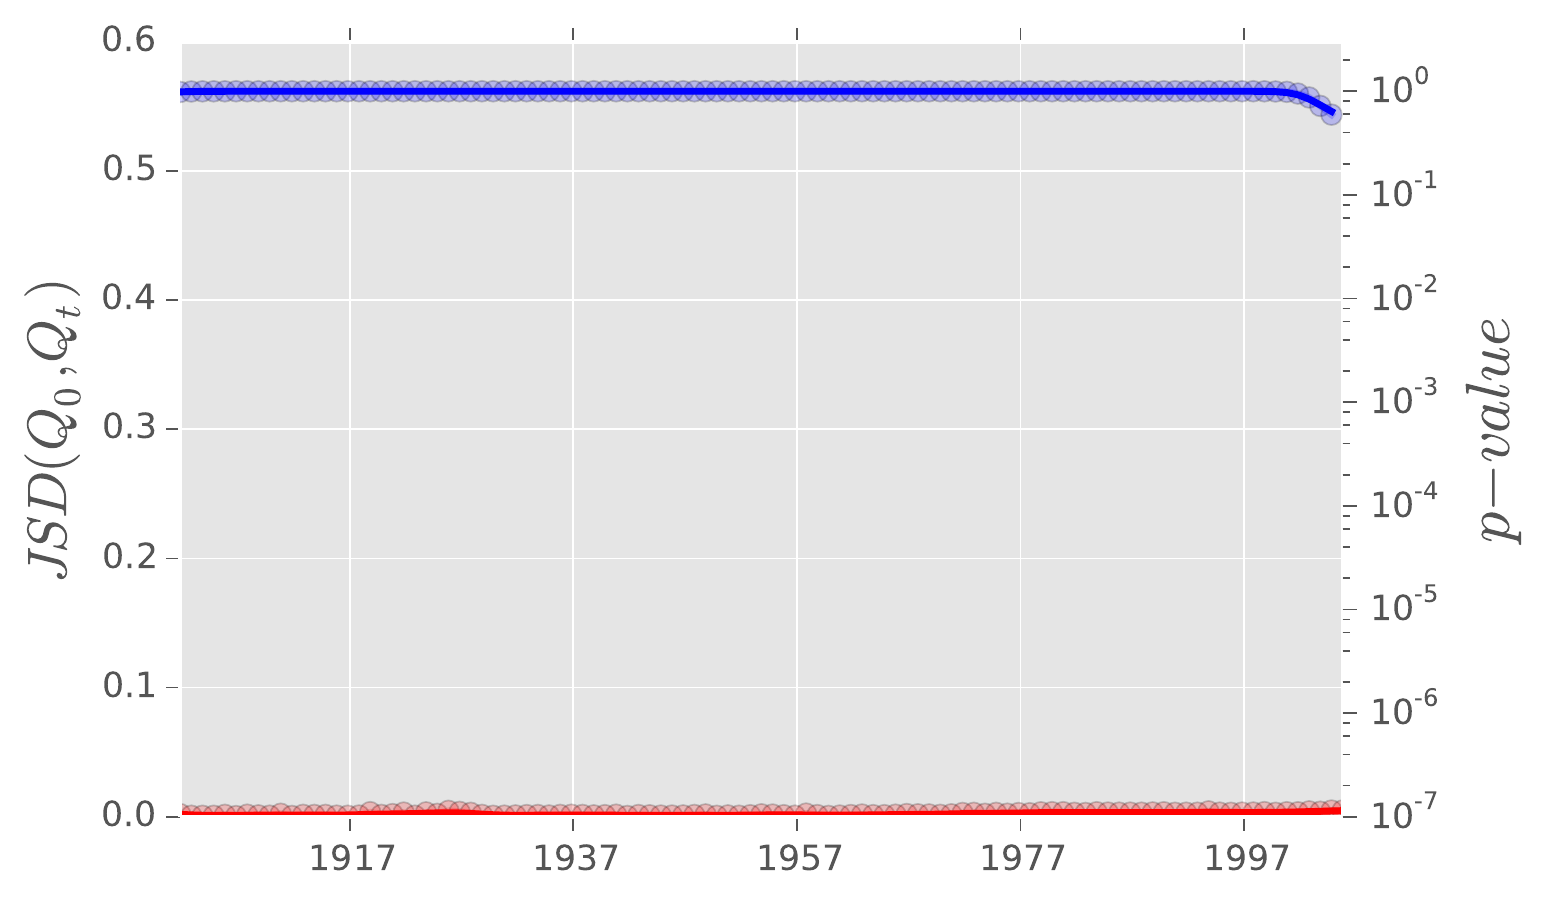} & \includegraphics[scale=0.25]{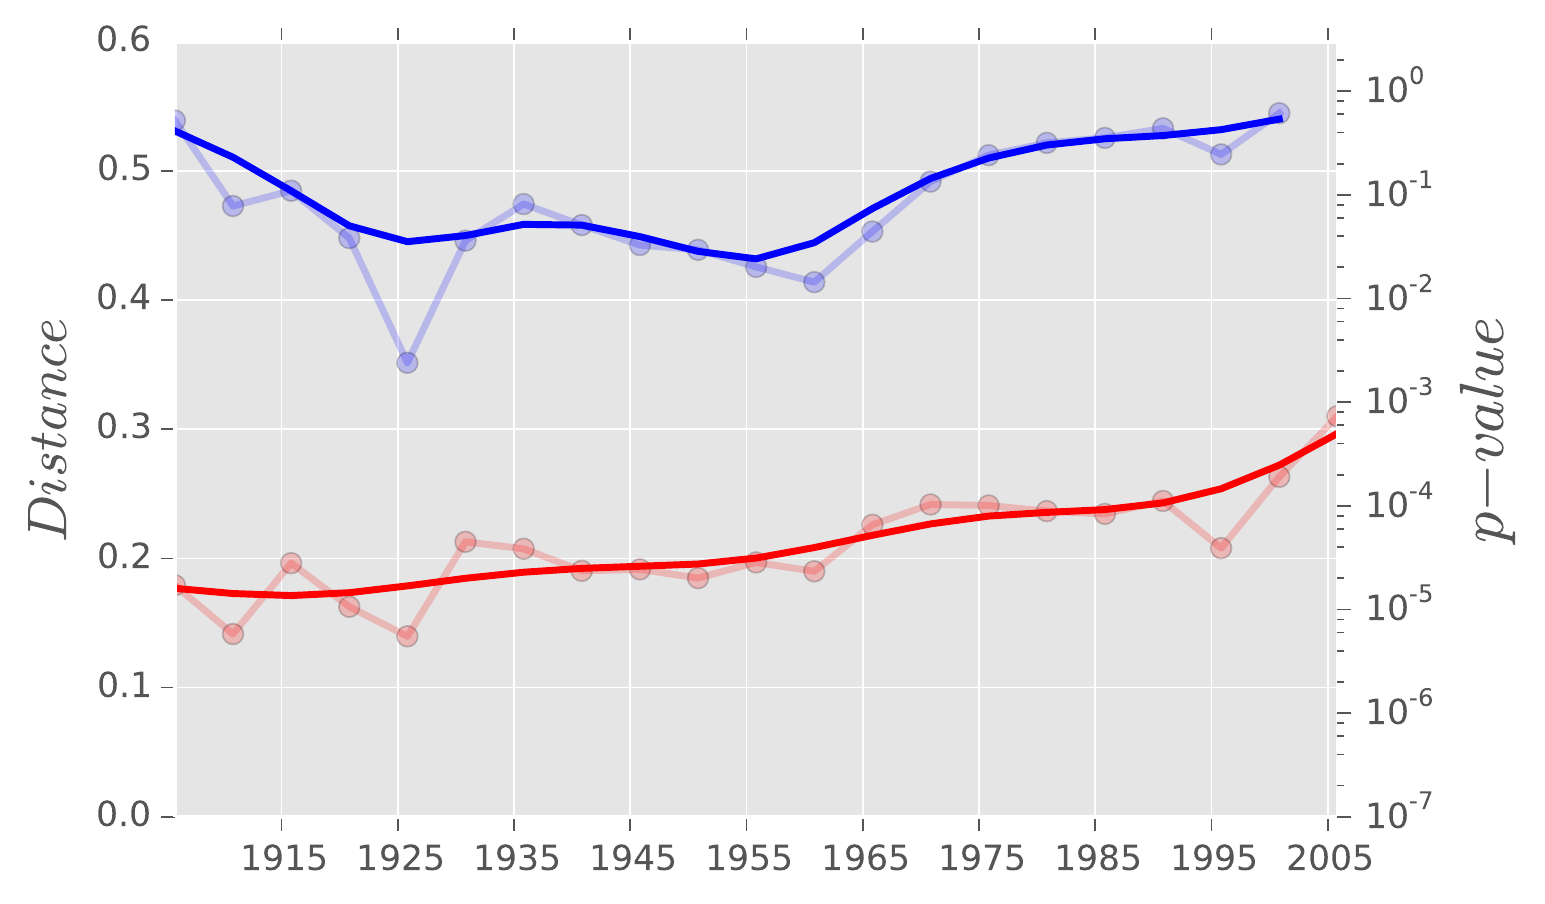} \\
\end{tabular}
%\label{tab:gt}
\caption{Time series of various words by the different methods. \comment{\todo{BP: beautify distributional method charts to look like frequency charts}}}
\end{table*}

\begin{table}
\centering
\caption{Popular words detected as changed by frequency method(pvalues $<0.0001$). These words increased in their frequency.}
\label{tab:freq}
\begin{tabular}{|c|l|} \hline
Word &  EstYear \\ \hline
texttt{face} & 1990 \\ \hline
\texttt{gay} & 1964 \\ \hline
\texttt{sex} & 1938 \\ \hline
\texttt{drugs} & 1935 \\ \hline
\texttt{her} & 1930 \\ \hline
\texttt{transmitted} & 1929  \\ \hline
\texttt{recording} & 1924 \\ \hline
\texttt{tape} & 1921 \\ \hline
\texttt{cell} & 1919 \\ \hline
\texttt{bitch} & 1906 \\ \hline
\end{tabular}
\end{table}

\begin{figure}
\begin{subfigure}{0.25\textwidth}
  \centering
  \includegraphics[width=\textwidth]{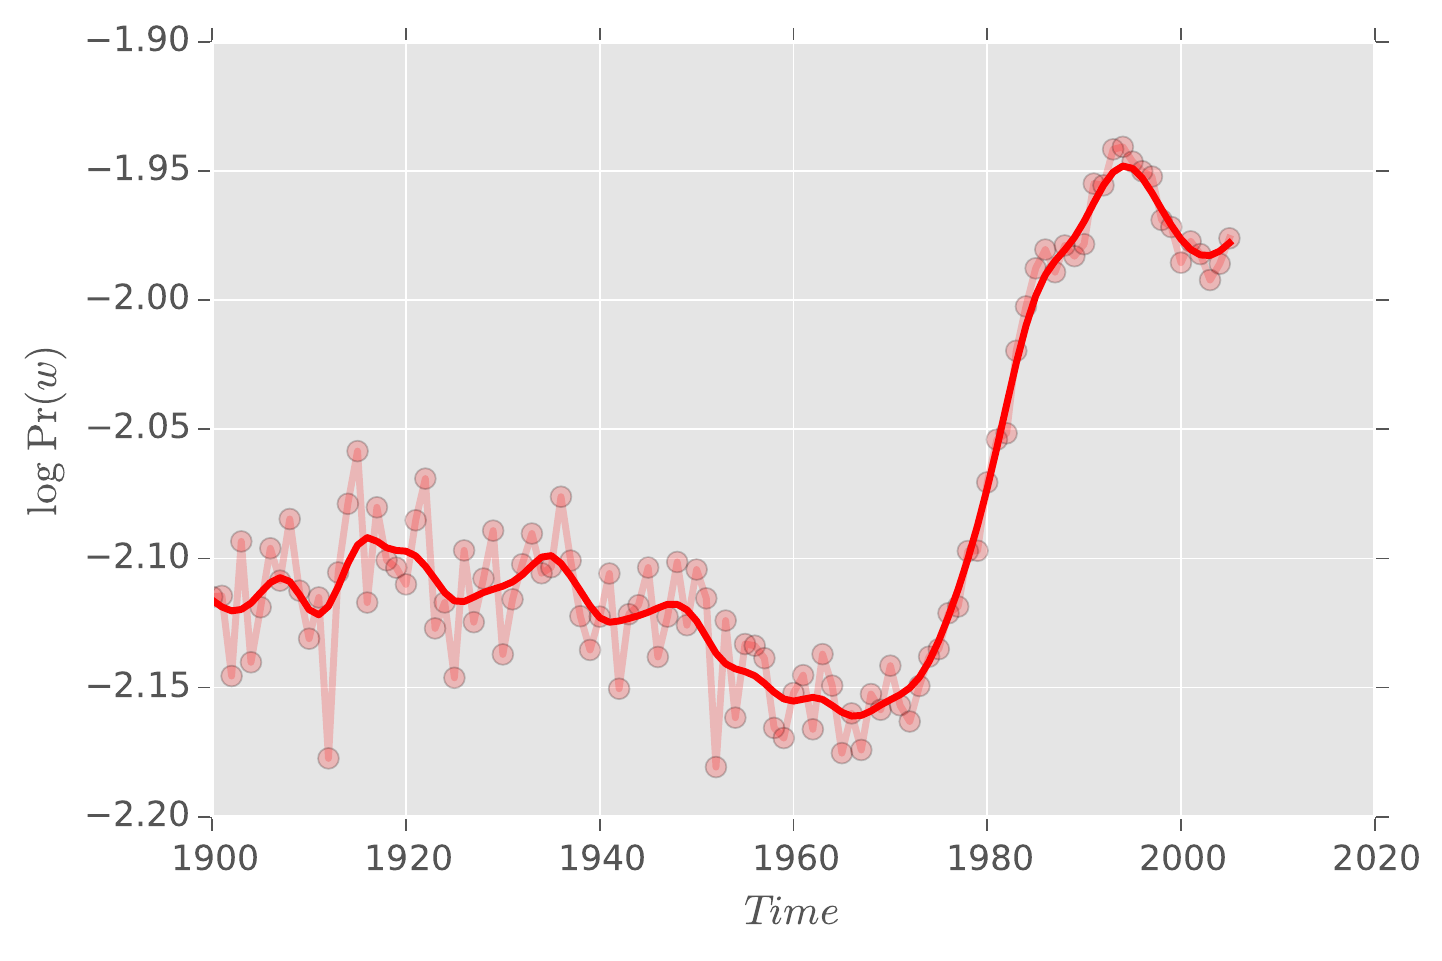}
  \caption{\texttt{her}}
  \label{fig:freqneg1}
\end{subfigure}%
\begin{subfigure}{0.25\textwidth}
  \centering
  \includegraphics[width=\textwidth]{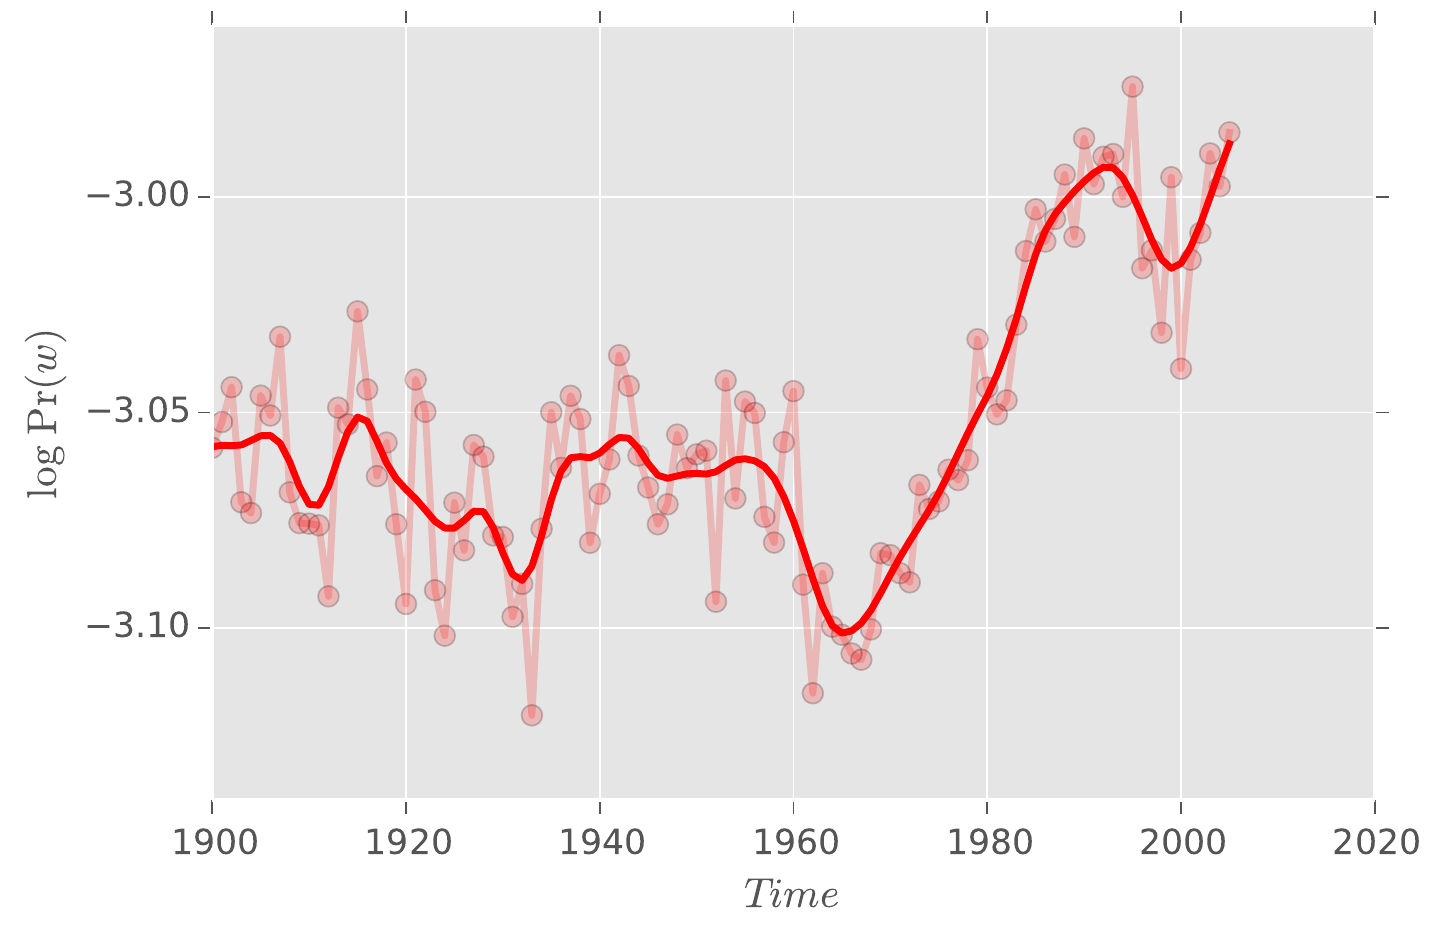}
  \caption{\texttt{face}}
  \label{fig:freqneg2}
\end{subfigure}%
\caption{Observe the rise in the usage of \emph{her} in 1960's. We believe this is due to the feminist movement picking up and not due to a change in meaning of the word.}
%\label{fig:freqneg}
\end{figure}

\begin{figure}
\begin{subfigure}{0.25\textwidth}
  \centering
  \includegraphics[width=\textwidth]{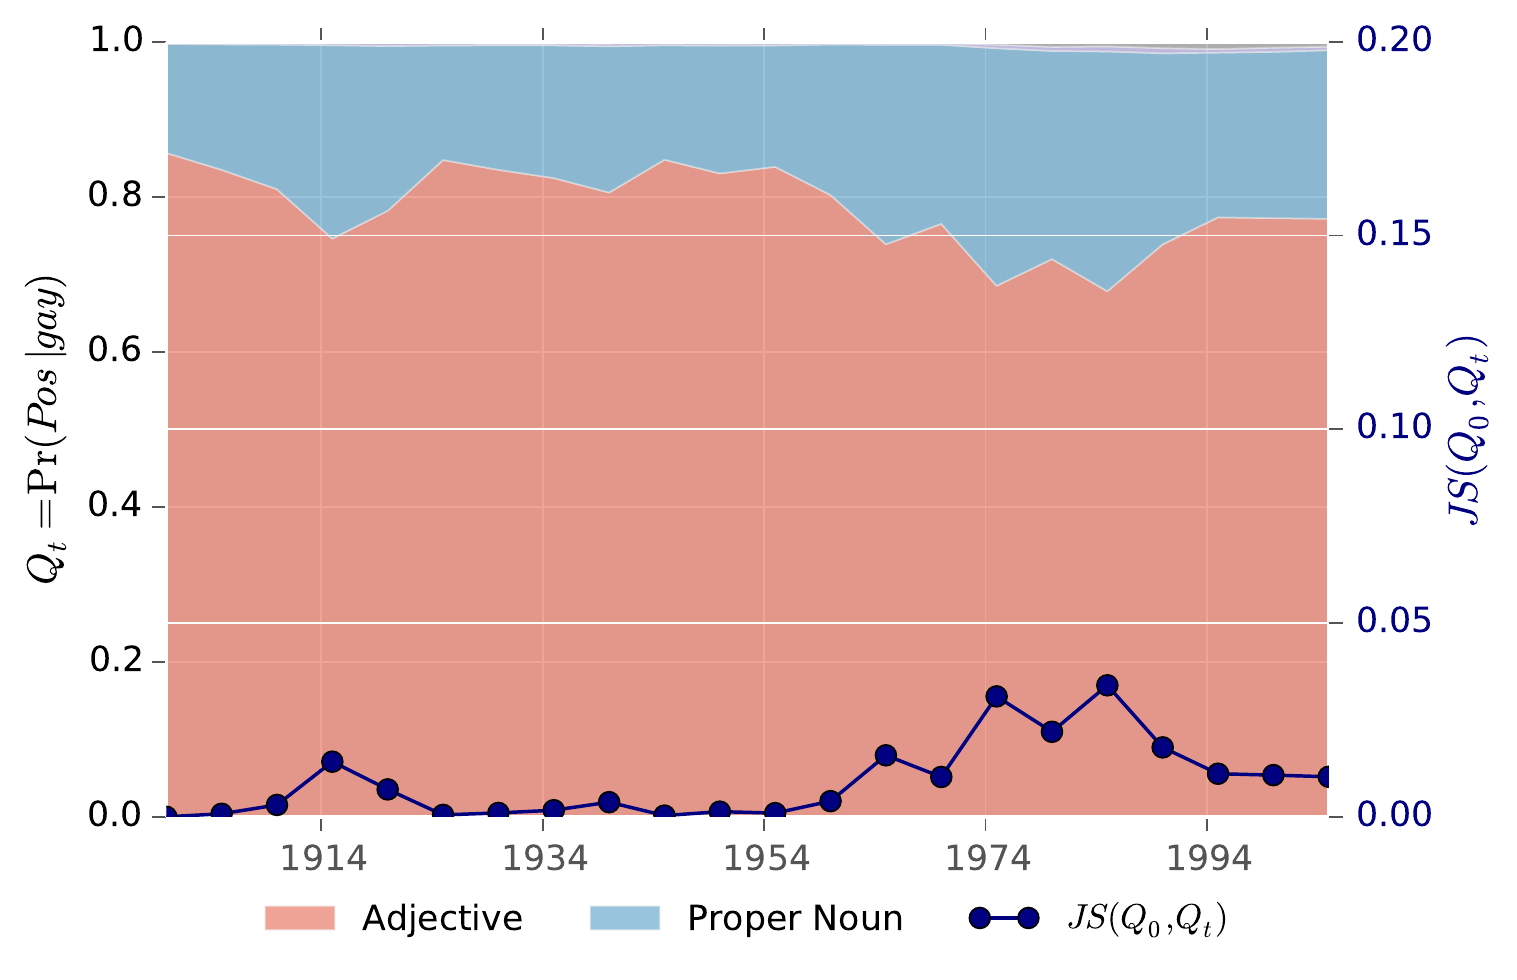}
  \caption{\texttt{gay}}
  \label{fig:posneg1}
\end{subfigure}%
\begin{subfigure}{0.25\textwidth}
  \centering
  \includegraphics[width=\textwidth]{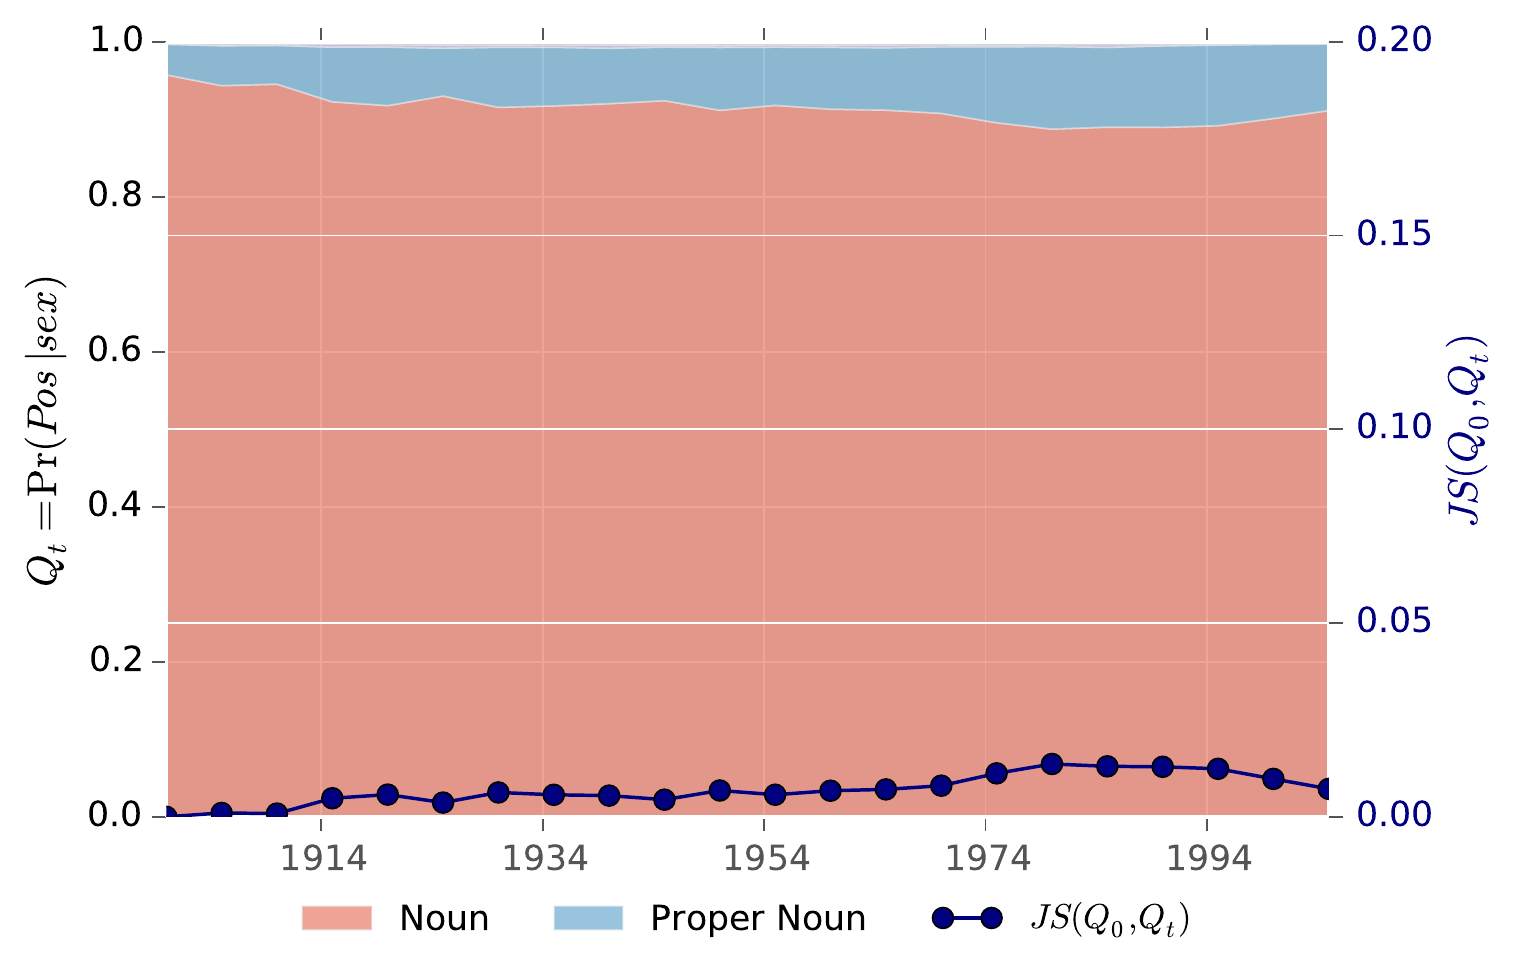}
  \caption{\texttt{sex}}
  \label{fig:posneg2}
\end{subfigure}%
\caption{Observe no significant change in POS distribution of words like \emph{gay} and \emph{sex} which undoubtedly shifted.}
%\label{fig:posneg}
\end{figure}

\begin{figure}[htb!]
\begin{subfigure}{0.25\textwidth}
  \centering
  \includegraphics[width=\textwidth]{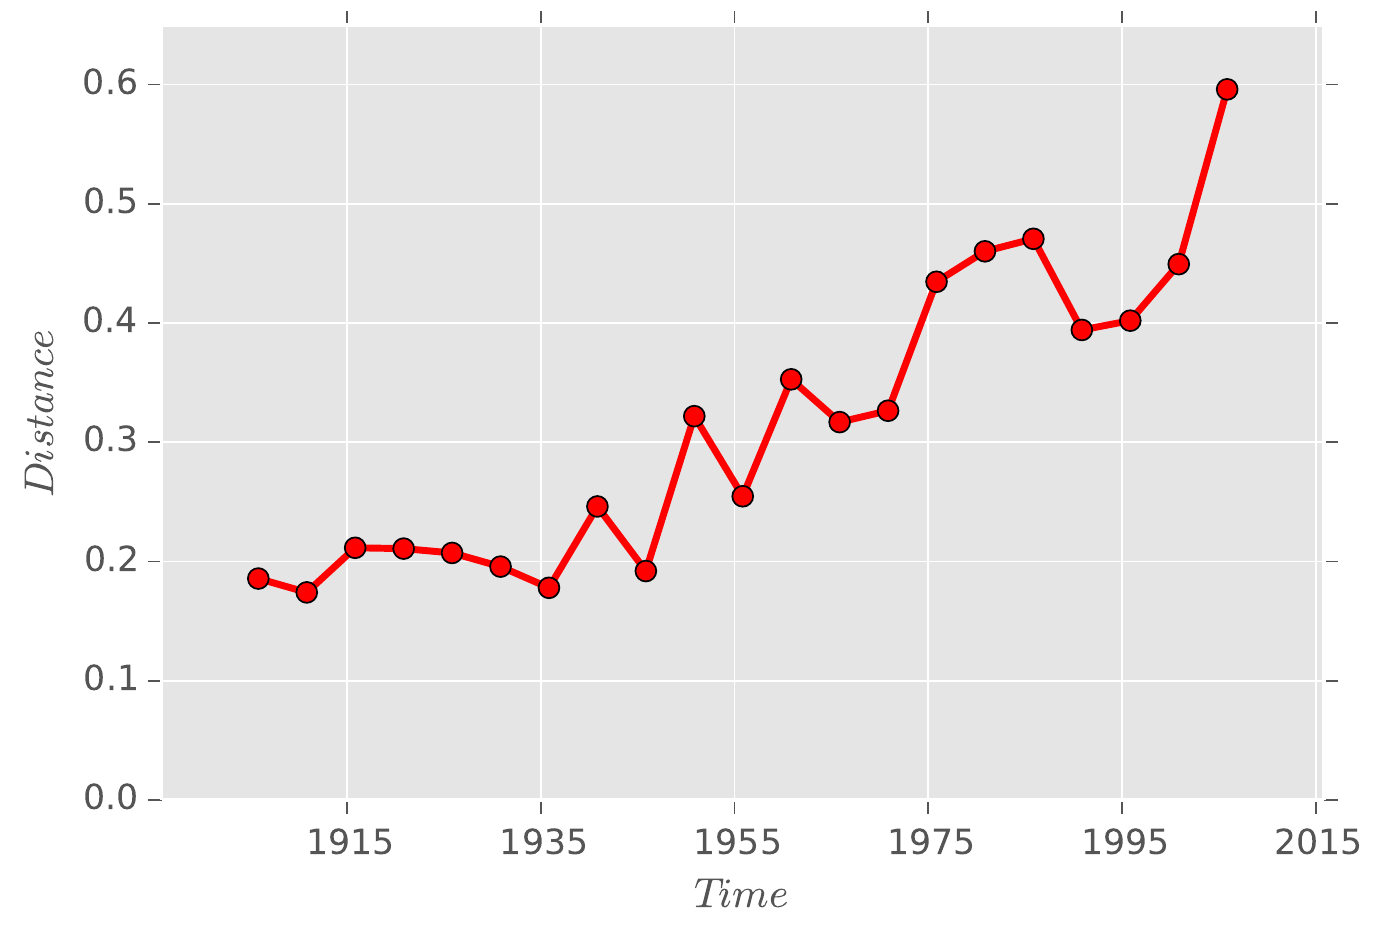}
  \caption{\texttt{tape}}
  \label{fig:etape}
\end{subfigure}%
\begin{subfigure}{0.25\textwidth}
  \centering
  \includegraphics[width = 1.0\textwidth]{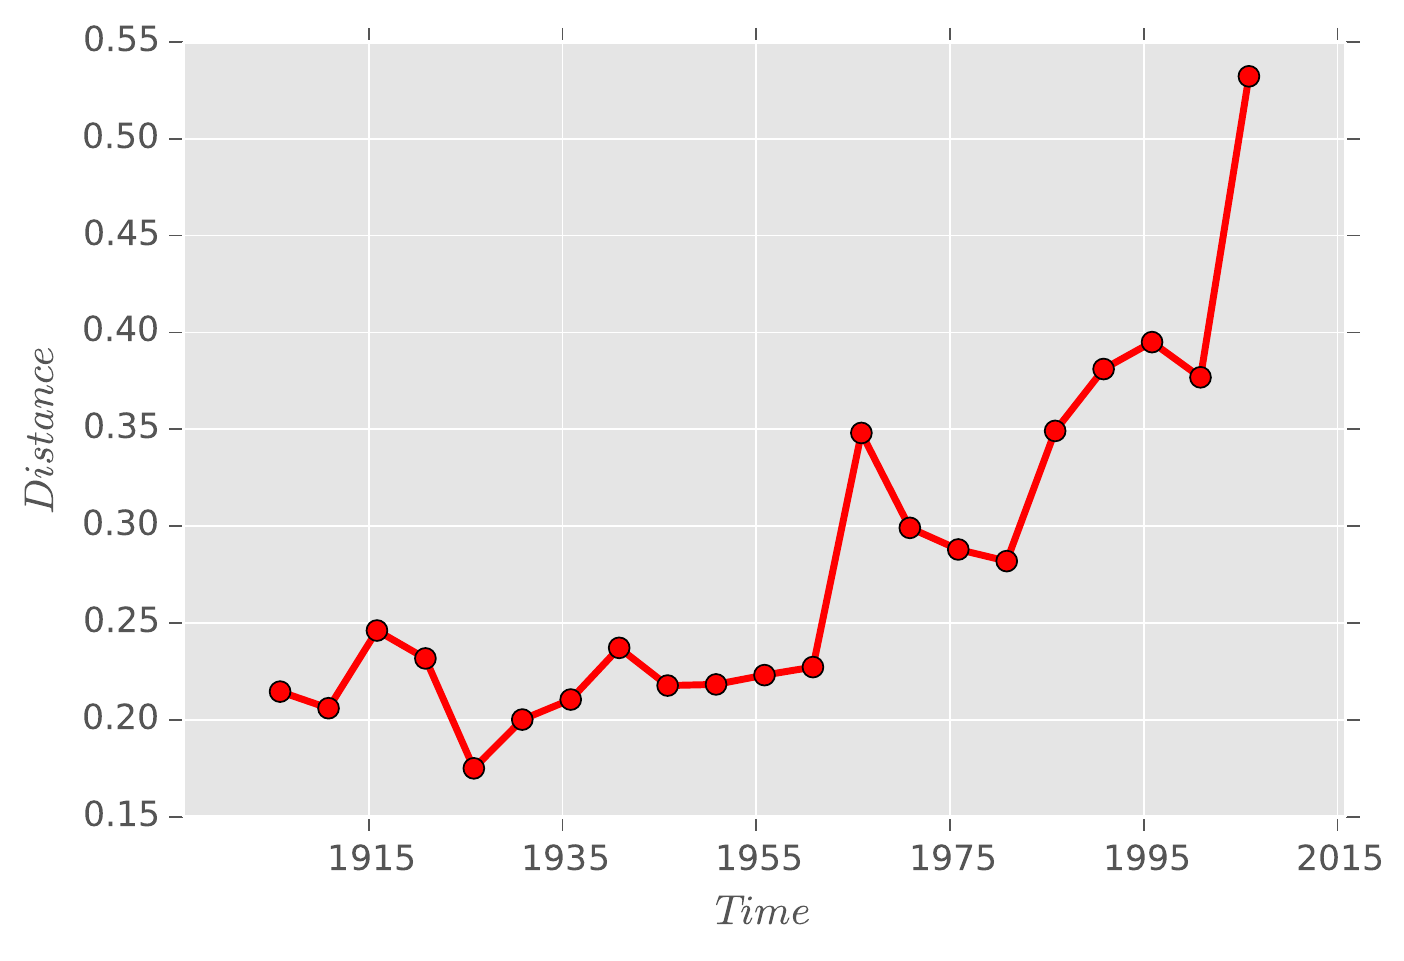}
  \caption{\texttt{sex}}
  \label{fig:esex}
\end{subfigure}%
\caption{Time series plots for \emph{tape} and \emph{sex} that shifted across time(based on the Google NGram data set)}
%\label{fig:ngrams_zscores}
\end{figure}

\begin{figure}
\begin{subfigure}{0.25\textwidth}
  \centering
  \includegraphics[width = 1.0\textwidth]{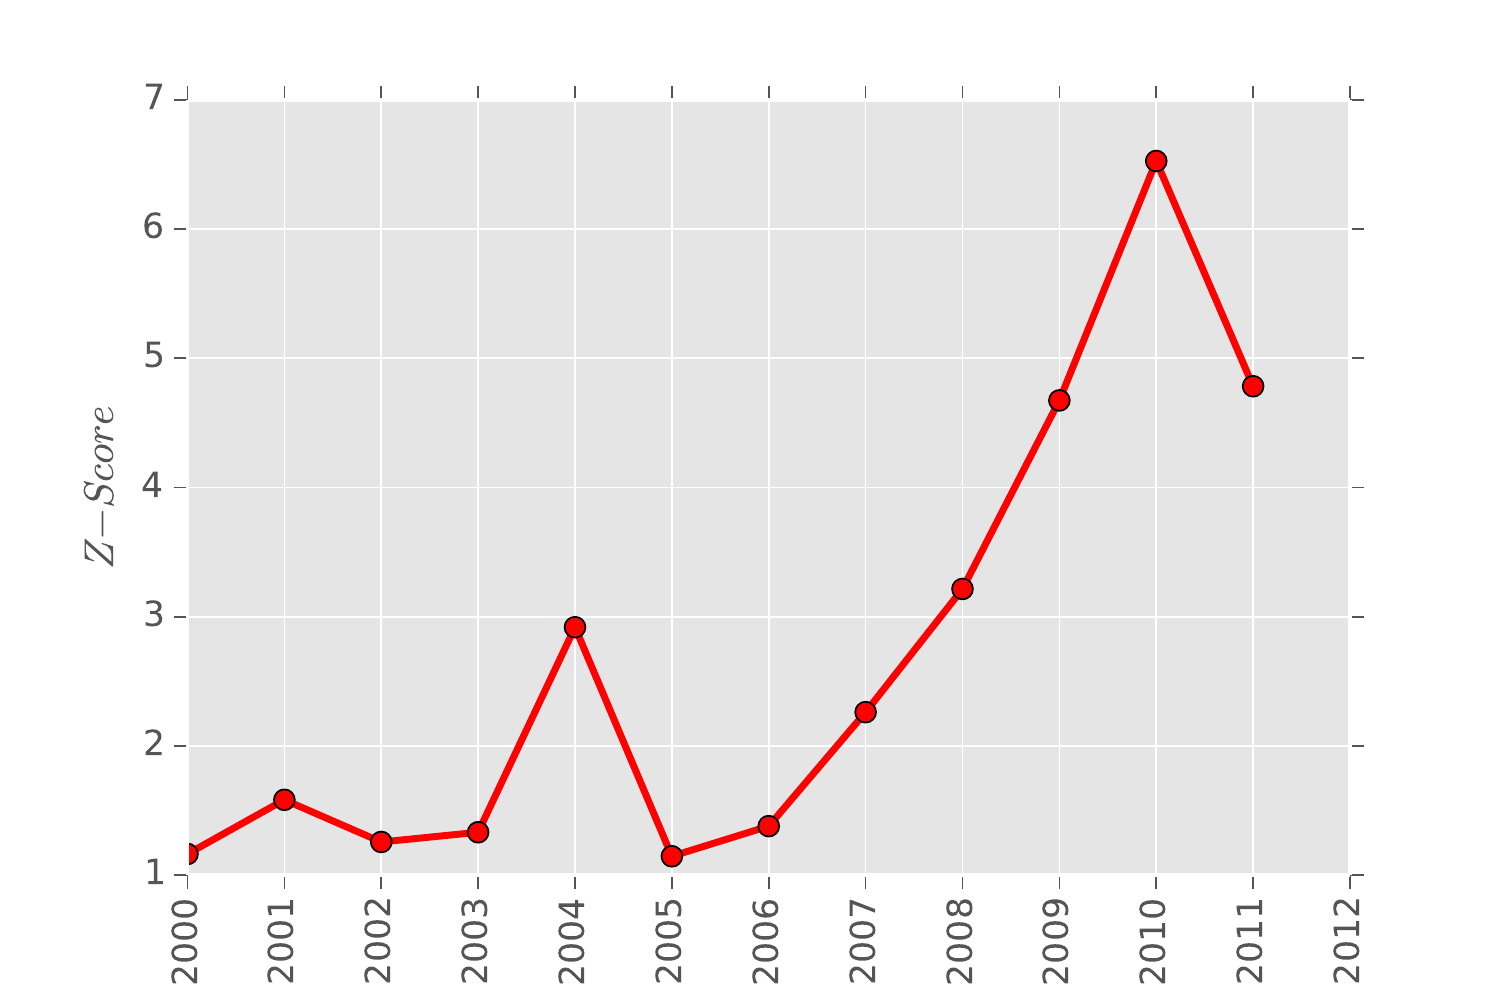}
  \caption{\texttt{streaming}}
  \label{fig:estreaming}
\end{subfigure}%
\begin{subfigure}{0.25\textwidth}
  \centering
  \includegraphics[width = 1.0\textwidth]{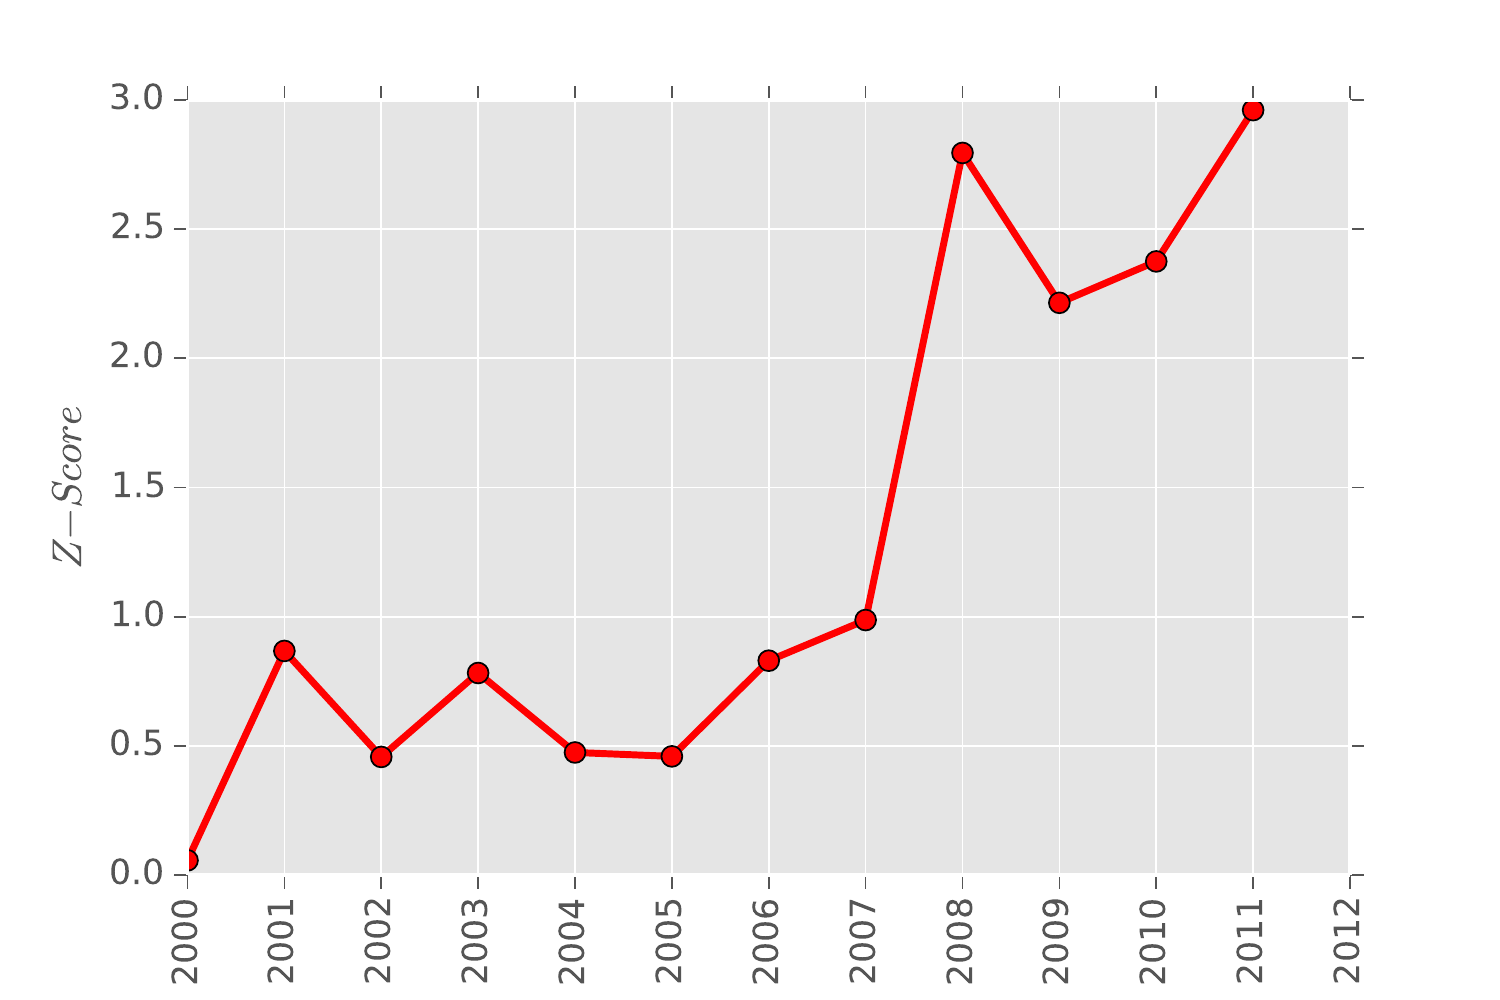}
  \caption{\texttt{twilight}}
  \label{fig:etwilight}
\end{subfigure}%
\caption{Time series plots for some words that shifted across time(based on the Amazon Movie Reviews)}
\label{fig:moviereviews}
\end{figure}

\begin{figure}
\begin{subfigure}{0.25\textwidth}
  \centering
  \includegraphics[width = 1.0\textwidth]{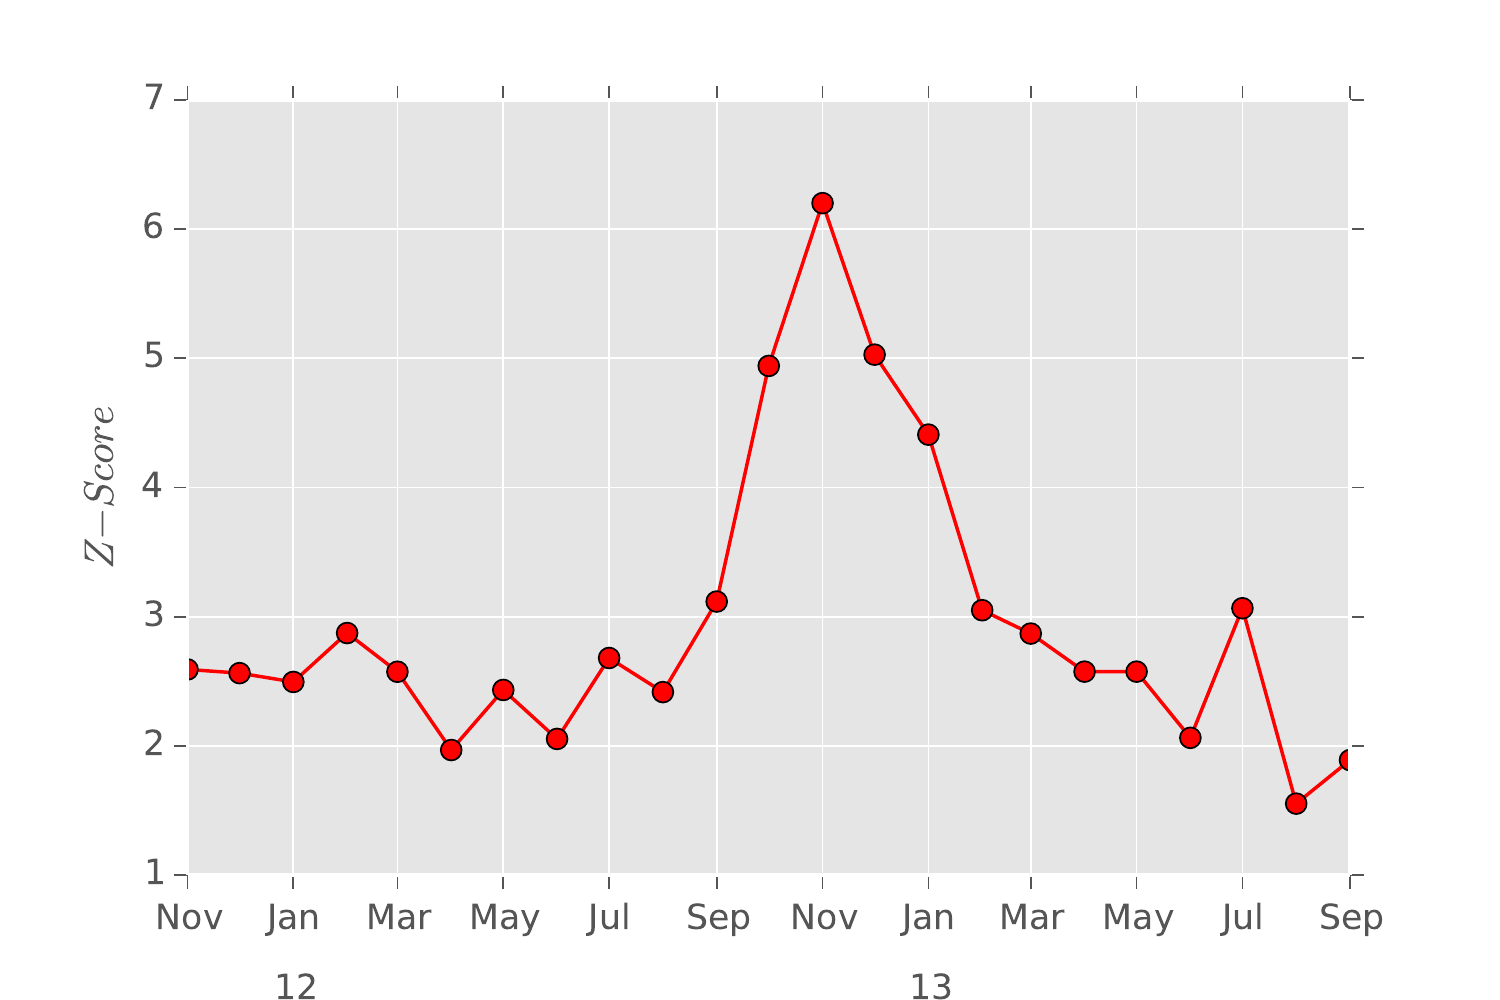}
  \caption{\texttt{sandy}}
  \label{fig:esandy}
\end{subfigure}%
\begin{subfigure}{0.25\textwidth}
  \centering
  \includegraphics[width = 1.0\textwidth]{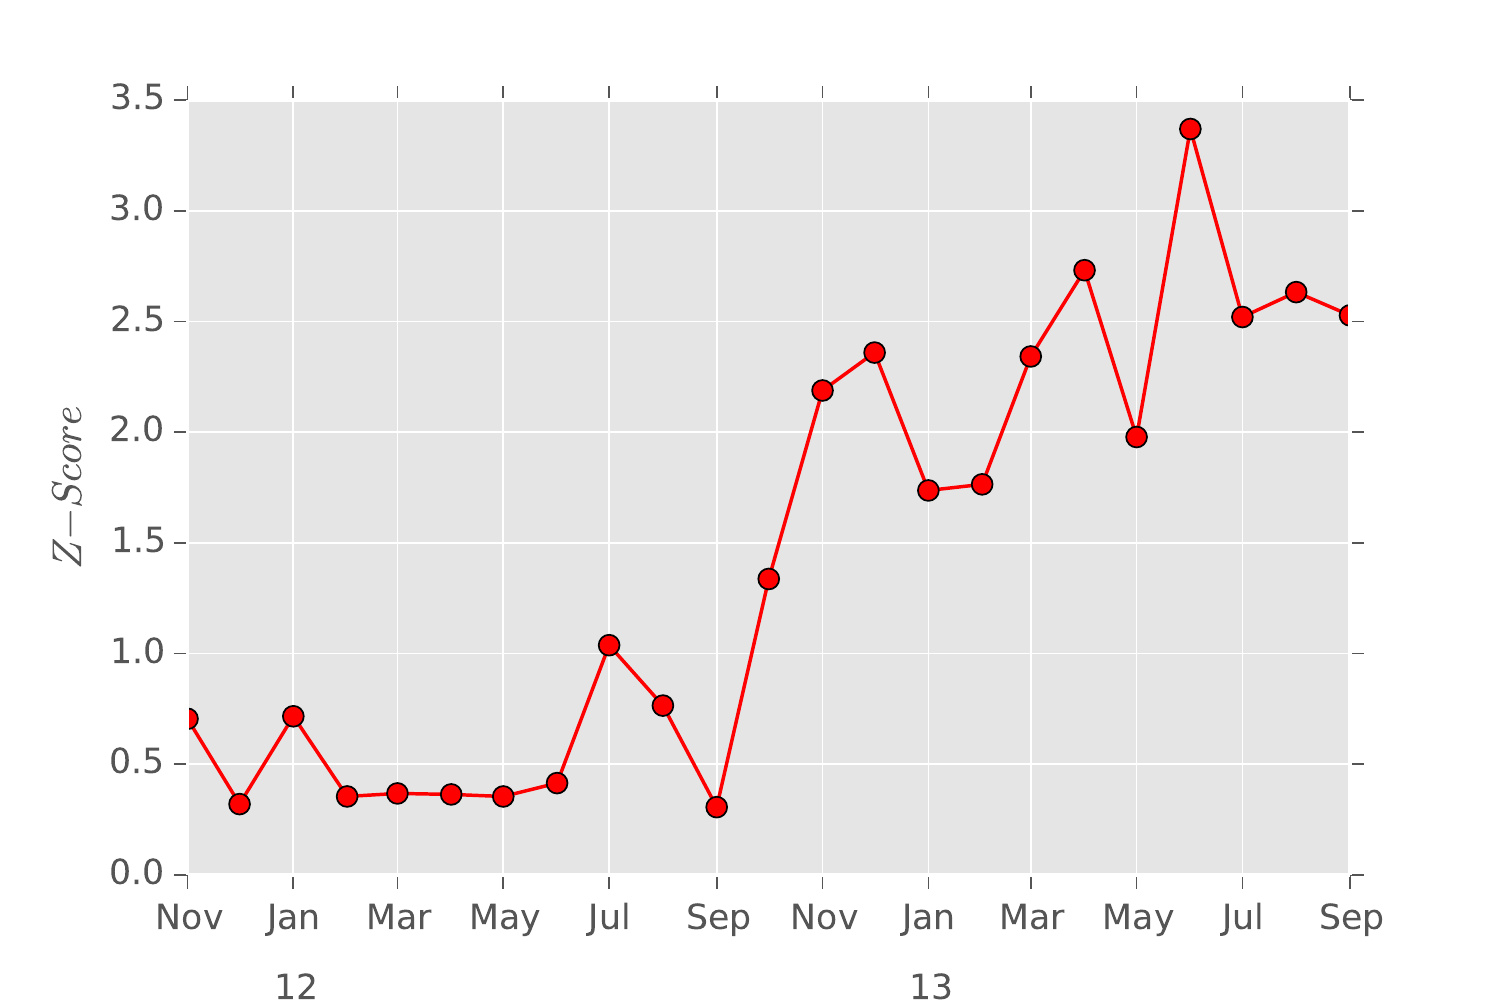}
  \caption{\texttt{snap}}
  \label{fig:esnap}
\end{subfigure}%
\caption{Time series plots for some words that shifted across time(based on Twitter data set)}
%\label{fig:twitter}
\end{figure}

\begin{table}
\centering
\caption{Popular words detected as changed by part of speech method. (pvalues $<0.001$)}
\label{tab:pos}
\begin{tabular}{|l|l|l|l|} \hline
Word & EstYear & Past Usage & Present Usage \\ \hline
\texttt{hug} & 2002 & Verb & Noun\\ \hline
\texttt{windows} & 1992 & Noun & Proper Noun \\ \hline
\texttt{bush} & 1989 & Noun & Proper Noun\\ \hline
\texttt{apple} & 1984 & Noun & Proper Noun\\ \hline
\texttt{top} & 1972 & Noun & Adjective\\ \hline
\texttt{sink} & 1972 & Verb & Noun\\ \hline
\texttt{click} & 1952 & Noun & Verb\\ \hline
\texttt{handle} & 1951 & Noun & Verb\\ \hline
\texttt{muster} & 1944 & Noun & Verb\\ \hline
\texttt{urge} & 1922 & Verb & Noun\\ \hline
\end{tabular}
\end{table}

\begin{table*}[th!]
\begin{center}
%\rowcolors{4}{white}{lightgray}
\begin{tabular}{l|l|cc|cc|cS[table-format = <1.4]|p{30mm}|p{30mm}}

& \textbf{Word} & \multicolumn{2}{c|}{\textbf{Freq}} & \multicolumn{2}{c|}{\textbf{POS}} & \multicolumn{2}{c|}{\textbf{Distributional}} & \multirow{2}{*}{\textbf{Past ngram }} & \multirow{2}{*}{\textbf{Present ngram}}\\
%\cline{1-7}
& & \textbf{ECP}  & \textbf{pvalue} & \textbf{ECP} & \textbf{pvalue} & \textbf{ECP} & \textbf{pvalue} &  & \\
\hline
&
\texttt{gay} & 1964 & < 0.001 & - & - & 1985 & 0.0001 & \emph{happy and gay} & \emph{gay and lesbians} \\

& \texttt{tape}& 1921 & < 0.001 & - & - & 1970 & <0.0001 & \emph{red tape, tape from her mouth}  & \emph{a copy of the tape} \\

& \texttt{checking} & 1921 & <0.001 & -  & - & 1970 & 0.0002 & \emph{then checking himself} & \emph{checking him out} \\

& \texttt{diet} & - & - & - & - & 1970 & 0.0104 & \emph{diet of bread and butter} & \emph{go on a diet} \\

& \texttt{sex} & 1938 & <0.001 & -  & - & 1965 & 0.0002 & \emph{and of the fair sex} & \emph{have sex with} \\

& \texttt{plastic} & 1921 & <0.001 & - & - & 1950 & 0.0005 & \emph{of plastic possibilities} & \emph{put in a plastic} \\

& \texttt{peck} & 1997 & <0.001 & - & - & 1935 & 0.0004 & \emph{brewed a peck} & \emph{a peck on the cheek} \\

\parbox[t]{1em}{\multirow{10}{*}{\rotatebox[origin=c]{90}{\dist \hspace{1pt} better}}} &

\texttt{honey} & 1907 & <0.001  & - & - & 1930 & 0.01 & \emph{land of milk and honey} & \emph{Oh honey !} \\

%\multicolumn{0}{c}{}\\
%\multicolumn{0}{c}{}\\

& \texttt{bitch} & 1906 & <0.001 & - & - & 1955 & 0.0001 & \emph{female dog (nicest black bitch) } & \emph{bitch (as a slang)} \\

& \texttt{transmitted} & 1929 & <0.001 & - & - & 1950 & 0.0002 & \emph{had been transmitted to him, transmitted from age to age} & \emph{transmitted in electronic form} \\

& \texttt{recording} & 1924 & <0.001 & 1950 & <0.001 & 1990 & 0.0263 & \emph{to be ashamed of recording that} & \emph{recording, photocopying} \\

& \texttt{her} & 1930 & <0.001 & - & - & - & >0.05 & \emph{No contextual change} & \emph{Frequency increase with no contextual change} \\

& \texttt{face} & 1921 & <0.001 & - & - & - & >0.05 & \emph{No contextual change} & \emph{Frequency increase with no contextual change} \\

\multicolumn{0}{c}{}\\
\multicolumn{8}{c}{} & \textbf{Past POS} & \textbf{Present POS} \\ \cline{9-10}

\parbox[t]{1em}{\multirow{10}{*}{\rotatebox[origin=c]{90}{\syn \hspace{1pt} better}}}

& \texttt{hug} & 1919 & <0.001 & 2002 & <0.001 & - & >0.05 & \emph{Verb} & \emph{Noun} \\

& \texttt{windows} & 1921 & <0.014 & 1992 & <0.001  & - & >0.05 &  \emph{Noun} & \emph{Proper Noun} \\

& \texttt{bush} & - & - & 1989 & <0.001 & - & >0.05 &  \emph{Noun} & \emph{Proper Noun} \\

& \texttt{apple} & - & - & 1984 & <0.001 & - & >0.05 &  \emph{Noun} & \emph{Proper Noun} \\

& \texttt{top} & 1903 & <0.001 & 1972 & <0.001 & - & >0.05 & \emph{Noun} & \emph{Adjective} \\

& \texttt{sink} & 1905 & <0.001 & 1972 & <0.001 & 1970 & 0.0031 & \emph{Verb} & \emph{Noun} \\

& \texttt{click} & 1928 & <0.001 & 1952 & <0.001 & - & >0.05 &  \emph{Noun} & \emph{Verb} \\

& \texttt{handle} & 1903 & <0.001 & 1951 & <0.001 & - & >0.05 &  \emph{Noun} & \emph{Verb} \\

\end{tabular}
\end{center}
\caption{Popular words detected to have changed using word embeddings. \small{\emph{ECP:estimated change point}} \todo{Beautify this table.}}
%\label{tab:ngrams_table}
\end{table*}

For example, we observe that this method claims that the word \emph{war} changed  in early 1900's.
However, observe that although the frequency of \emph{war} changed due to the World Wars during that period, the meaning did not change.
